# Supplementary material for: Linear bound in terms of maxmaxflow for the chromatic roots of series-parallel graphs
Source: arXiv:1307.1721 ancillary file (2013-07-05)

## Approximate shapes of $S_1$ and $S_2$ for $R = 2.2$

This document contains supporting plots for the paper “*Linear bound in terms of maxmaxflow for the chromatic roots of series-parallel graphs*” by Gordon Royle and Alan Sokal.

Each of the following pages contains a single plot showing the approximations for the sets  $S_1$  and  $S_2$  for a particular value of  $q$ . The chosen values of  $q$  all lie on the circle  $|q - 1| = 2.2$  and are spaced equally around the circle in increments of 5 degree. Thus for  $k = 0, 5, 10, \dots, 180$ , there are plots for each  $q$  of the form  $q = 1 + 2.2e^{2\pi i(k/360)}$ .

Each plot shows in light-green the approximation for  $S_2$  and in dark-blue the approximation for  $S_1$ . The important points  $t_0 = 1/(1-q)$  and  $t_0^2$  are marked by a + and a  $\times$  respectively. If the true regions  $S_1$  and  $S_2$  are contained completely within the circle  $|t| = 1$  then this certifies that  $q$  is not a chromatic root for any series-parallel graph of maxmaxflow  $\Lambda = 3$ .

*Plot for  $q = 3.200 + 0.000\ i$  ( $R = 2.200$ ,  $k = 000$ )*

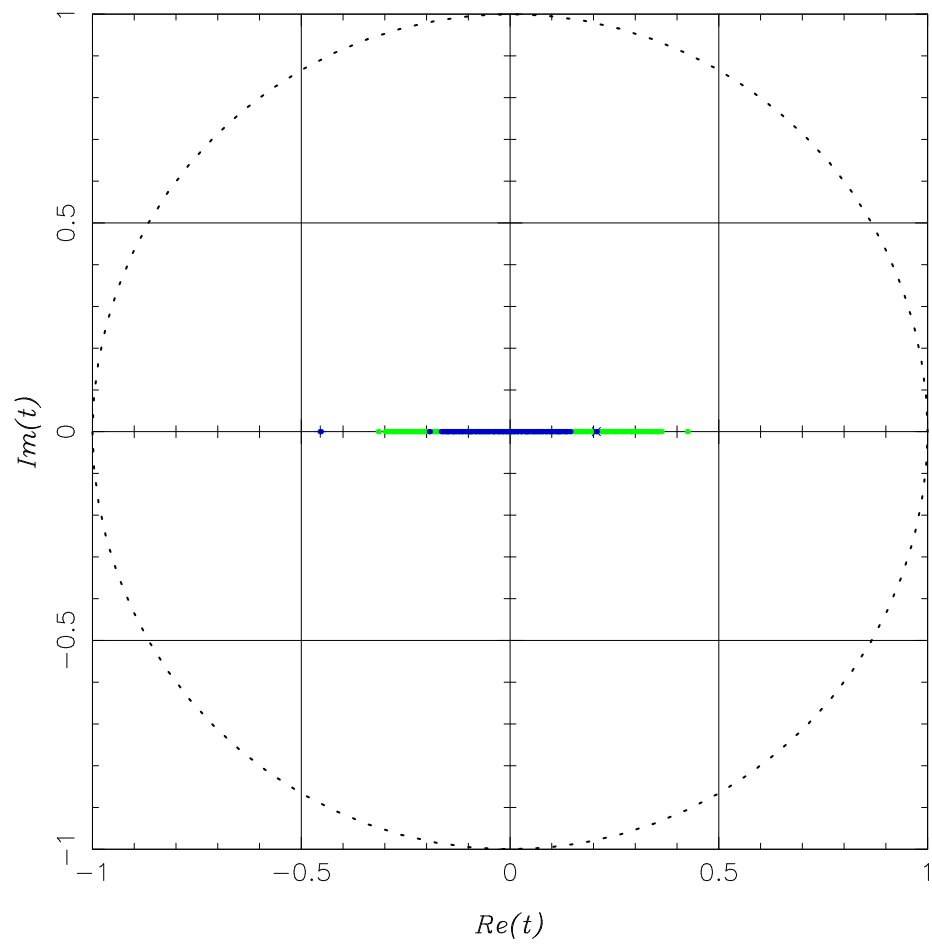

*Plot for  $q = 3.192 + 0.192 i$  ( $R = 2.200$ ,  $k = 005$ )*

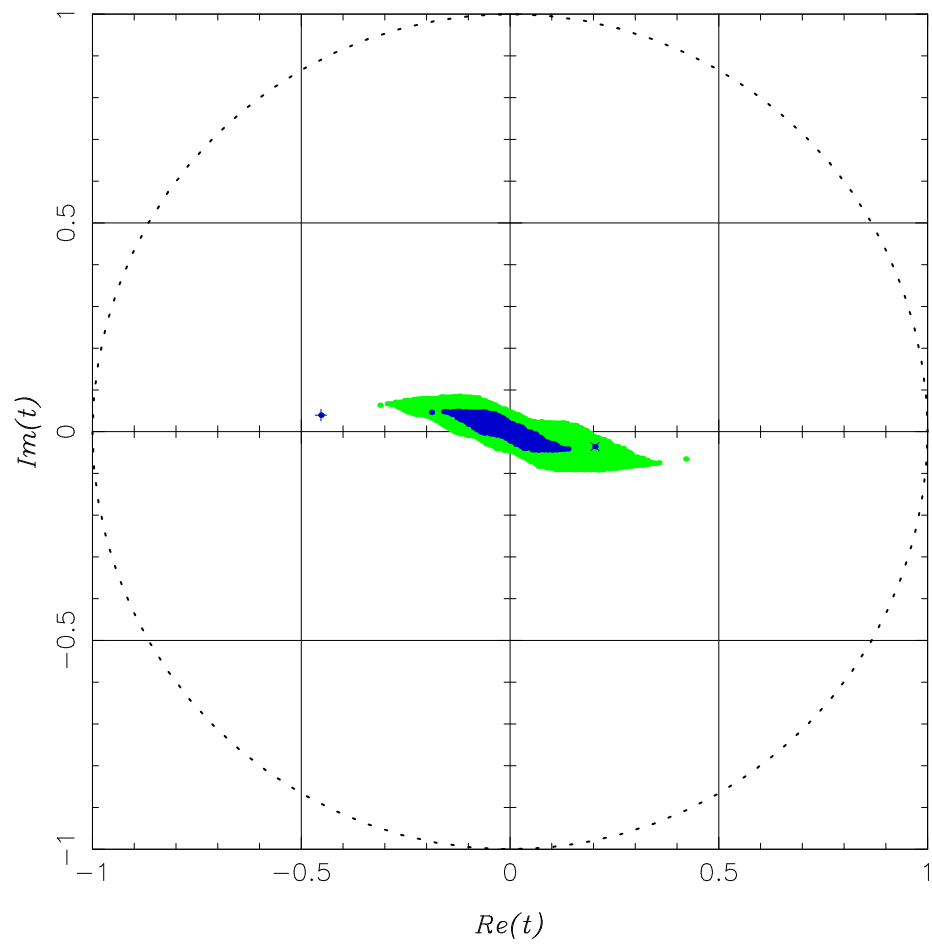

*Plot for  $q = 3.167 + 0.382 i$  ( $R = 2.200$ ,  $k = 010$ )*

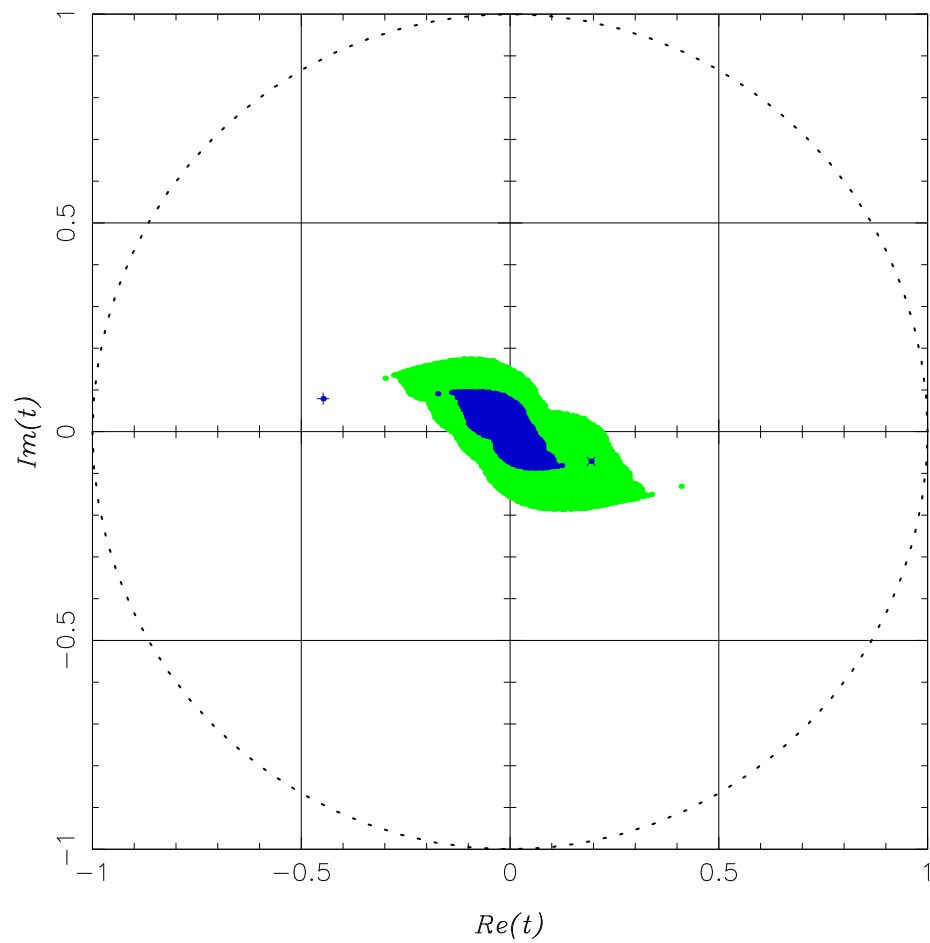

*Plot for  $q = 3.125 + 0.569 i$  ( $R = 2.200$ ,  $k = 015$ )*

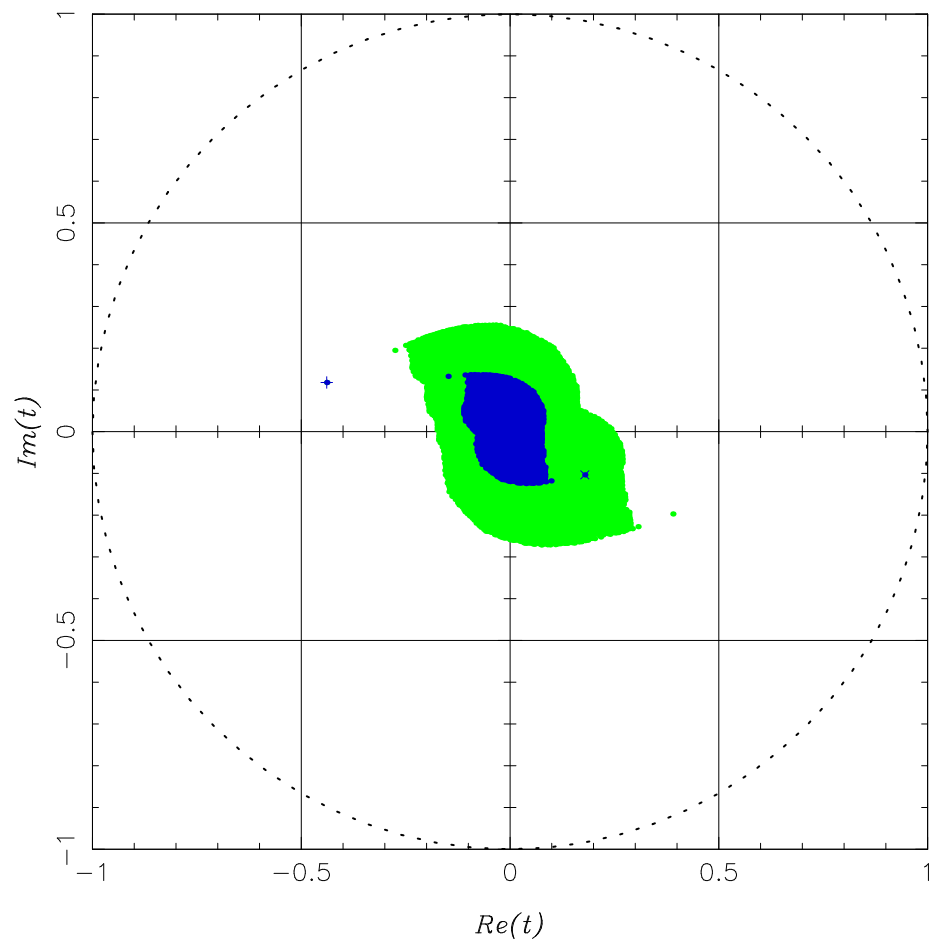

*Plot for  $q = 3.067 + 0.752 i$  ( $R = 2.200$ ,  $k = 020$ )*

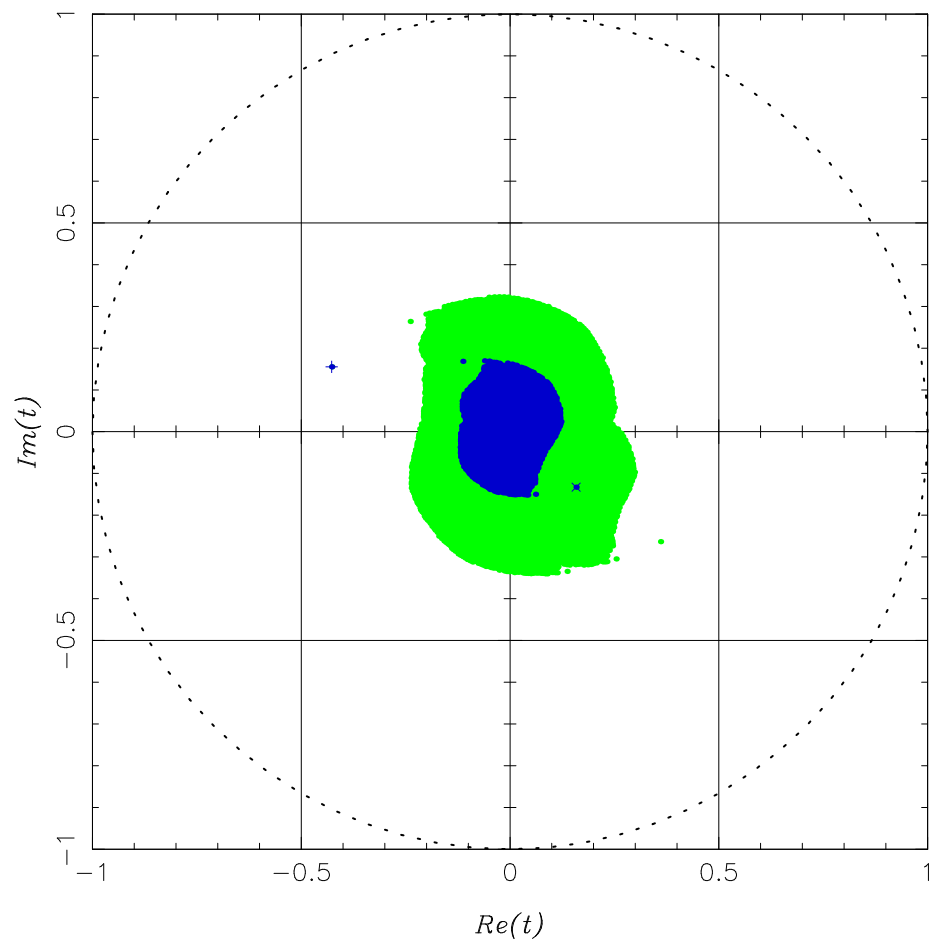

*Plot for  $q = 2.994 + 0.930 i$  ( $R = 2.200$ ,  $k = 025$ )*

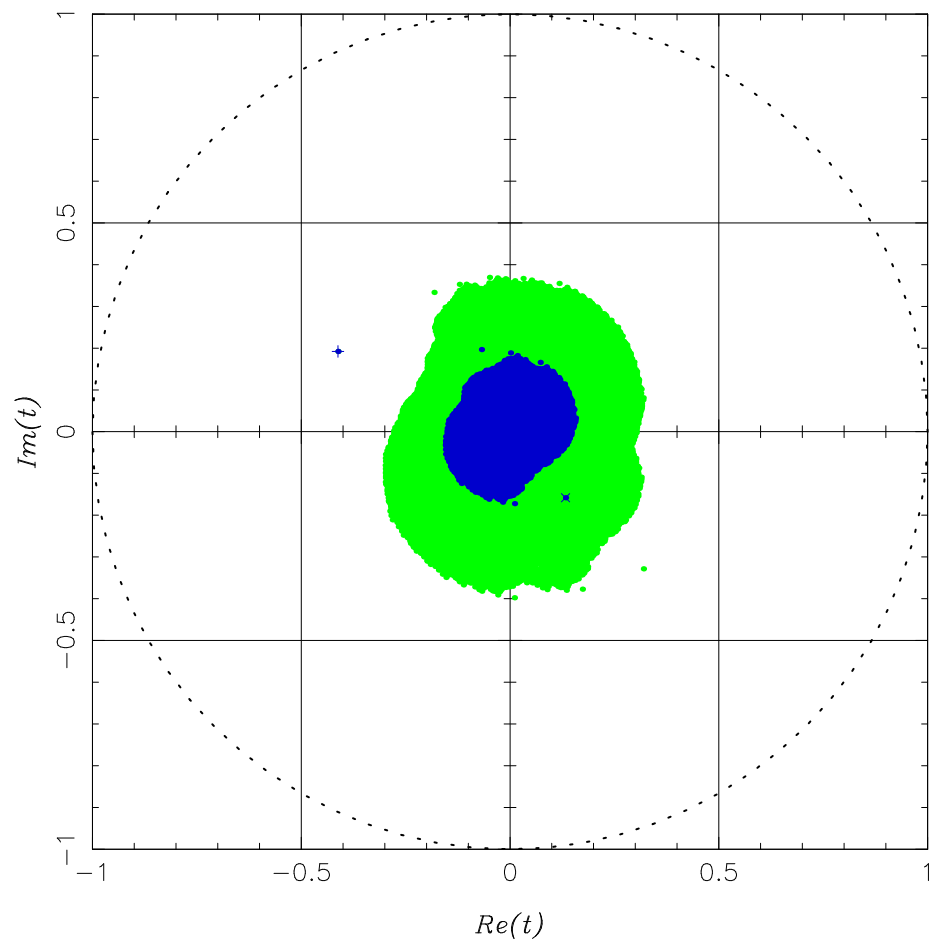

*Plot for  $q = 2.905 + 1.100 i$  ( $R = 2.200$ ,  $k = 030$ )*

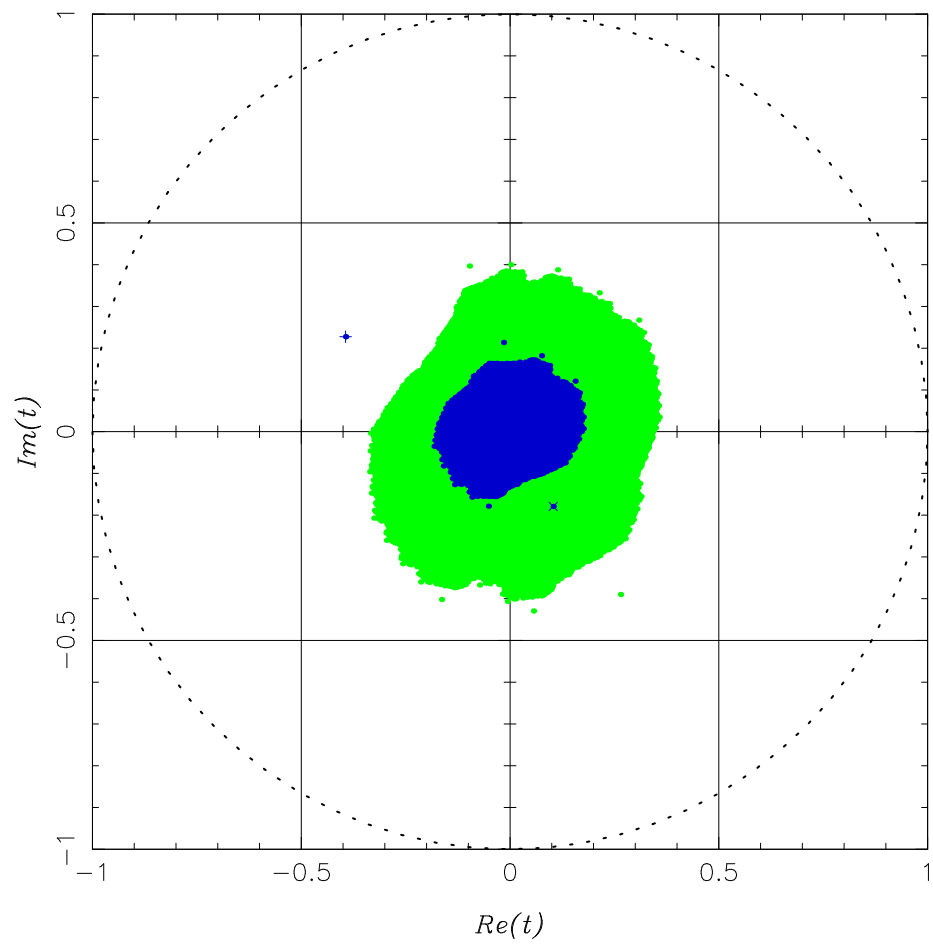



*Plot for  $q = 2.802 + 1.262 i$  ( $R = 2.200$ ,  $k = 035$ )*

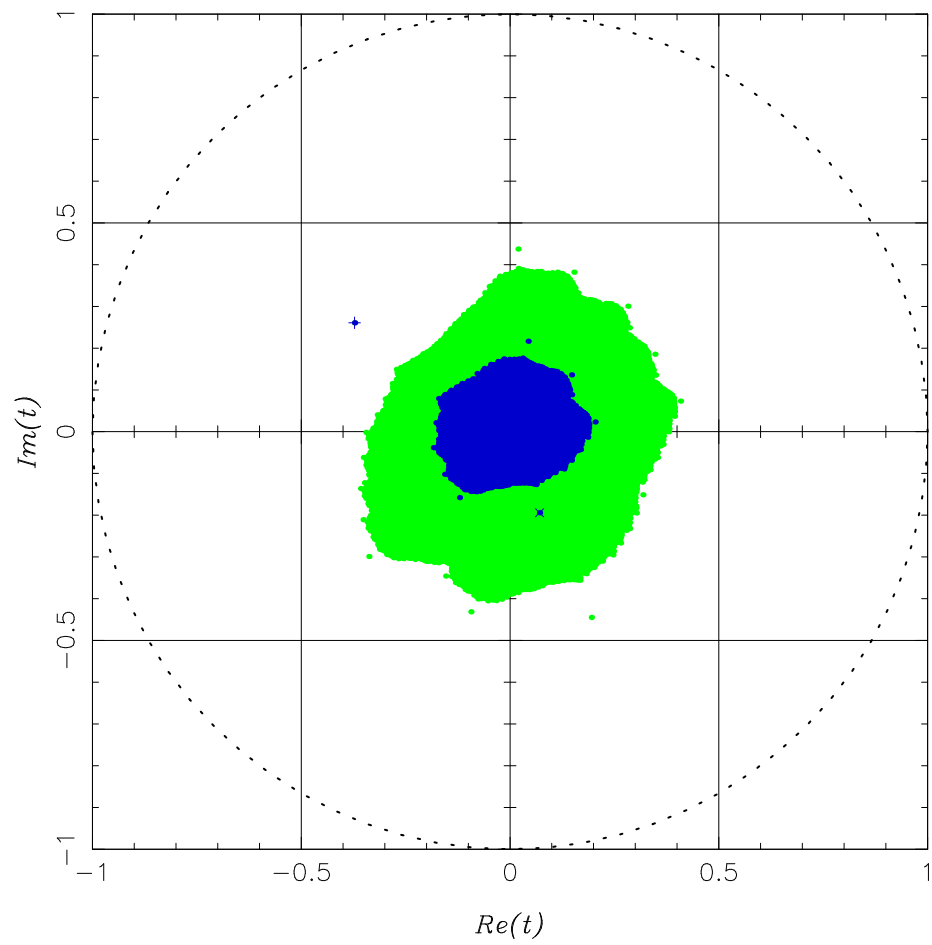

*Plot for  $q = 2.685 + 1.414 i$  ( $R = 2.200$ ,  $k = 040$ )*

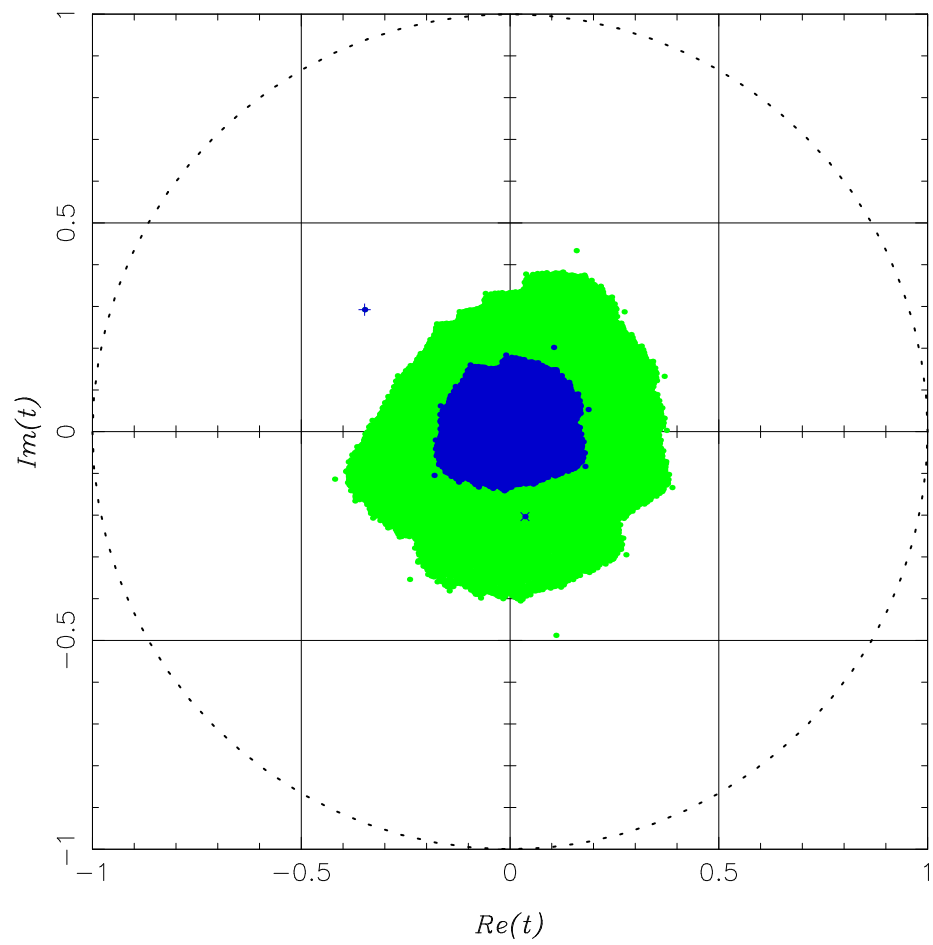

*Plot for  $q = 2.556 + 1.556 i$  ( $R = 2.200$ ,  $k = 045$ )*

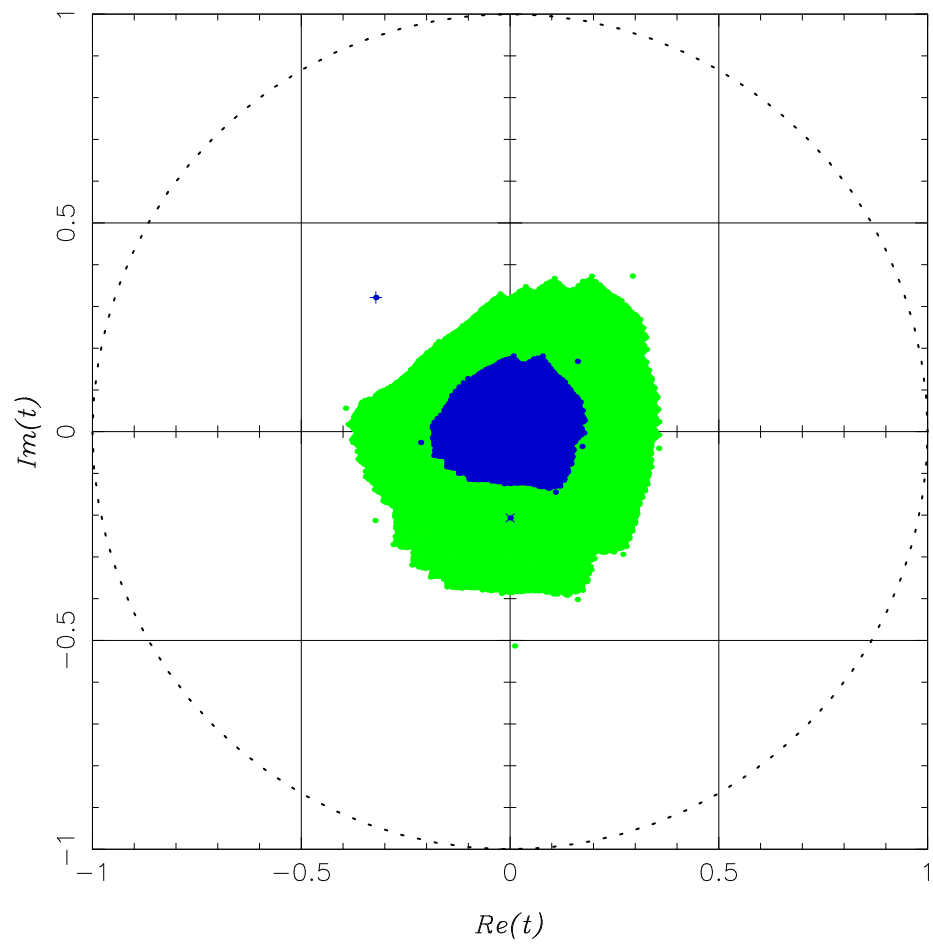

*Plot for  $q = 2.414 + 1.685 i$  ( $R = 2.200$ ,  $k = 050$ )*

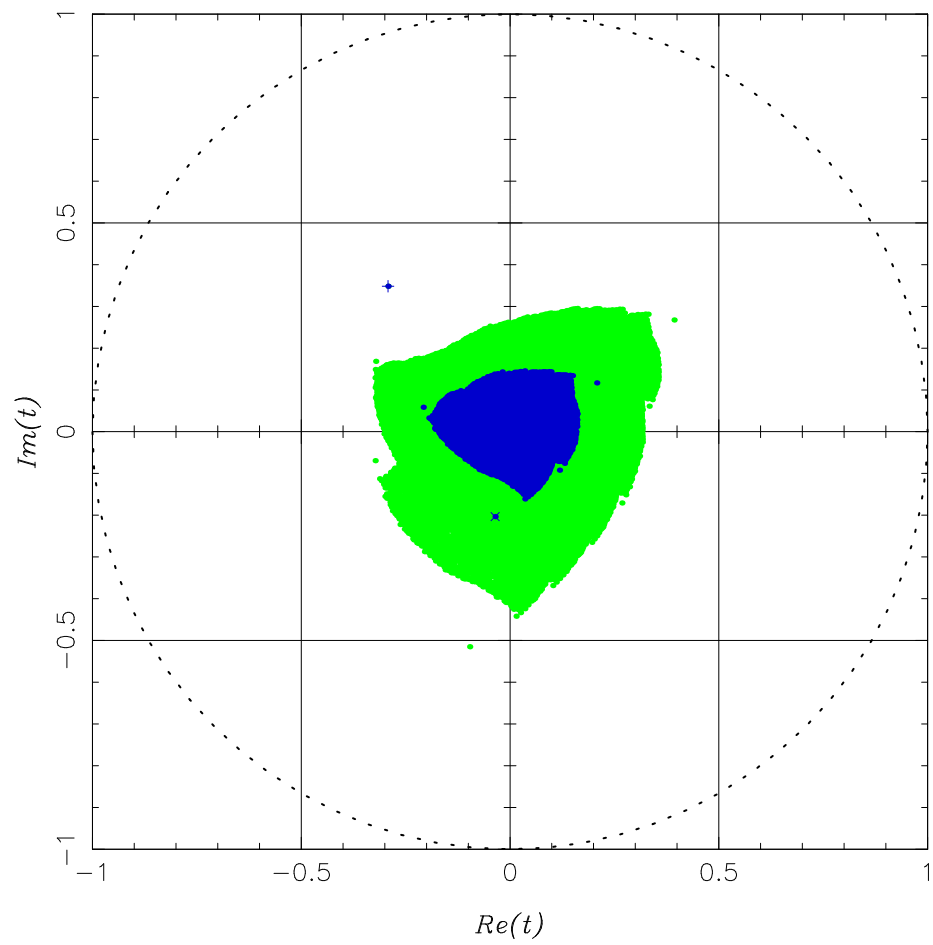

*Plot for  $q = 2.262 + 1.802 i$  ( $R = 2.200$ ,  $k = 055$ )*

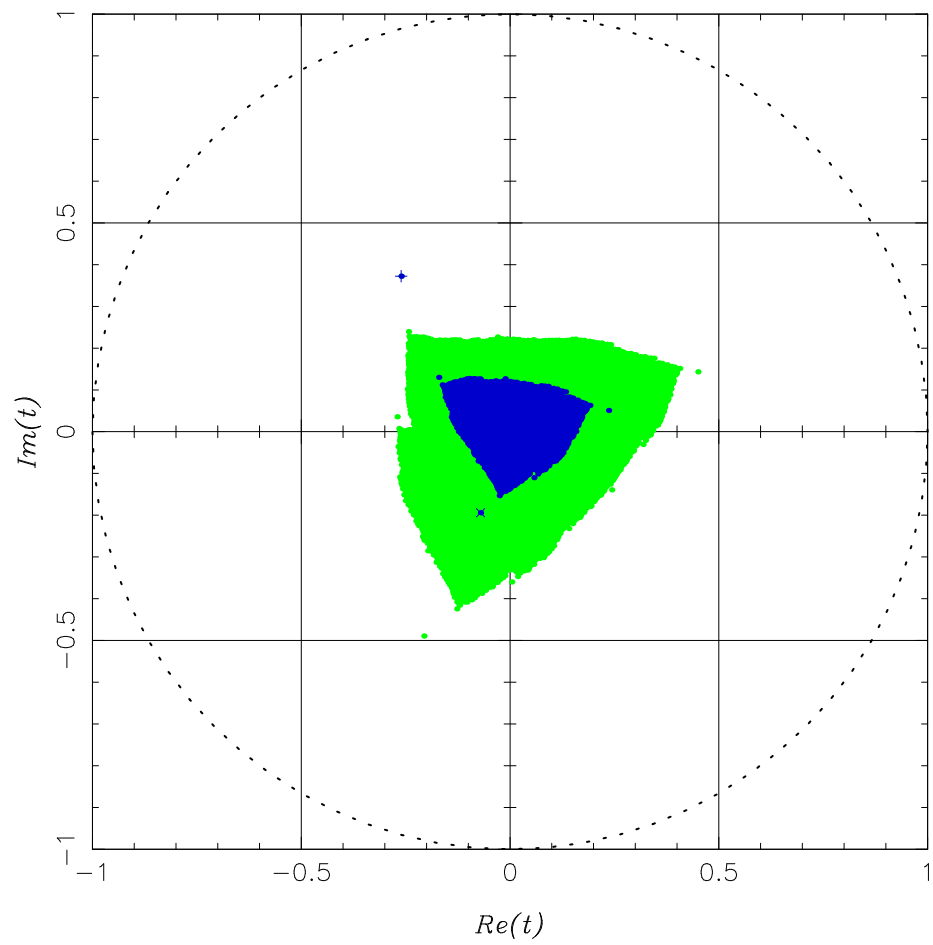

*Plot for  $q = 2.100 + 1.905 i$  ( $R = 2.200$ ,  $k = 060$ )*

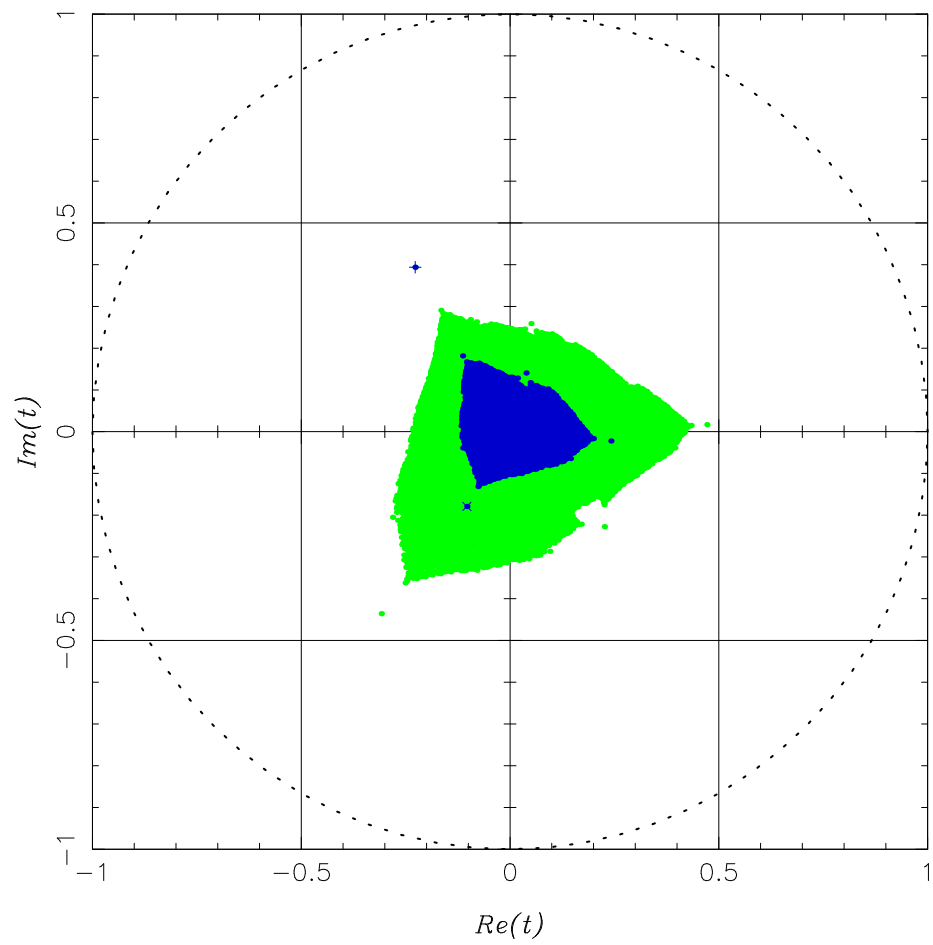

*Plot for  $q = 1.930 + 1.994 i$  ( $R = 2.200$ ,  $k = 065$ )*

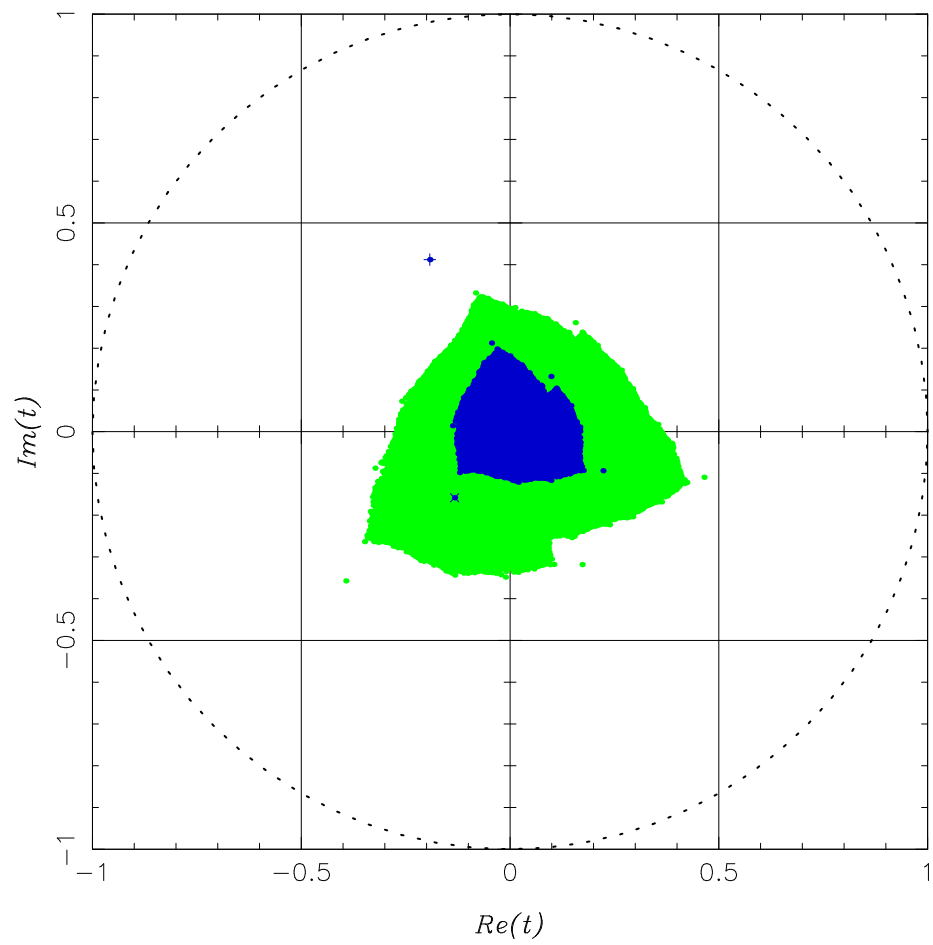

*Plot for  $q = 1.752 + 2.067 i$  ( $R = 2.200$ ,  $k = 070$ )*

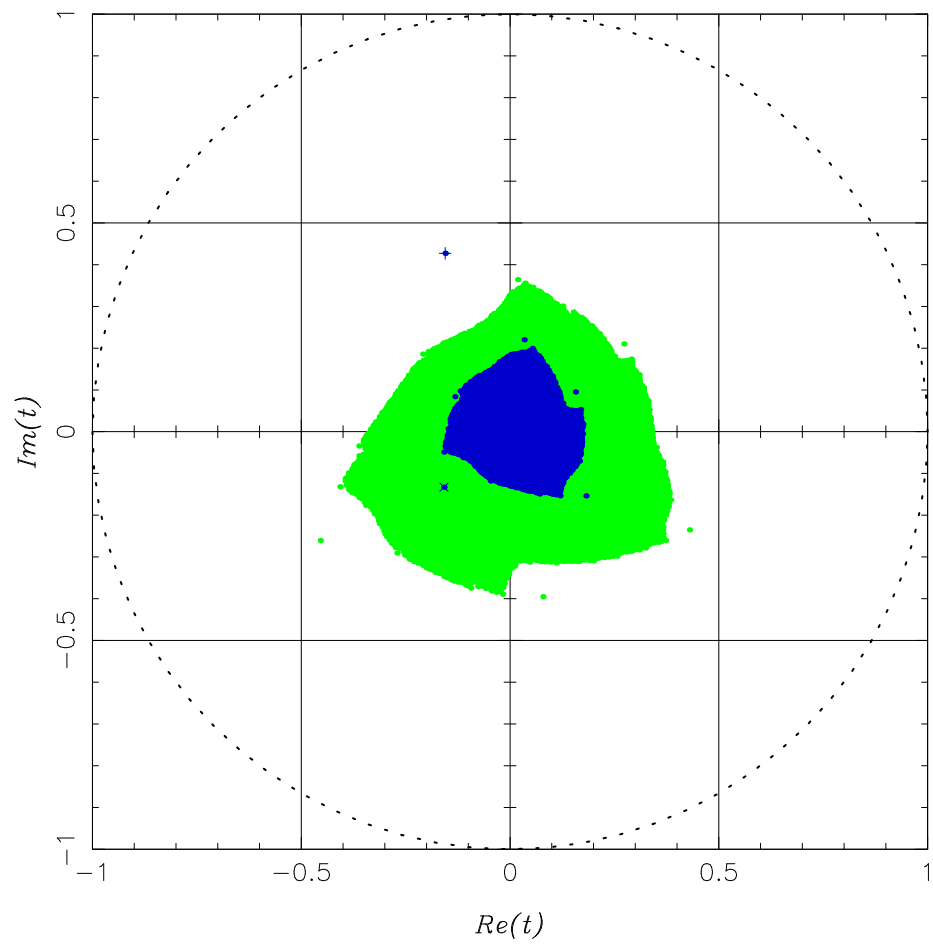



*Plot for  $q = 1.569 + 2.125 i$  ( $R = 2.200$ ,  $k = 075$ )*

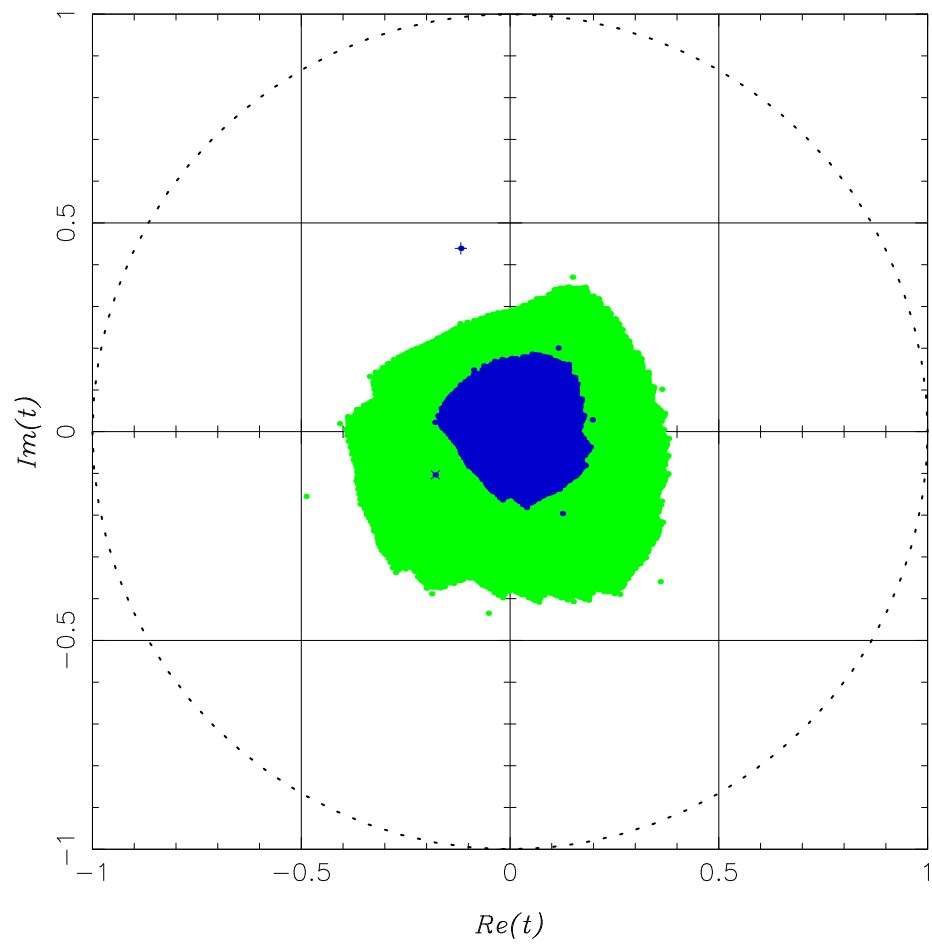

*Plot for  $q = 1.382 + 2.167 i$  ( $R = 2.200$ ,  $k = 080$ )*

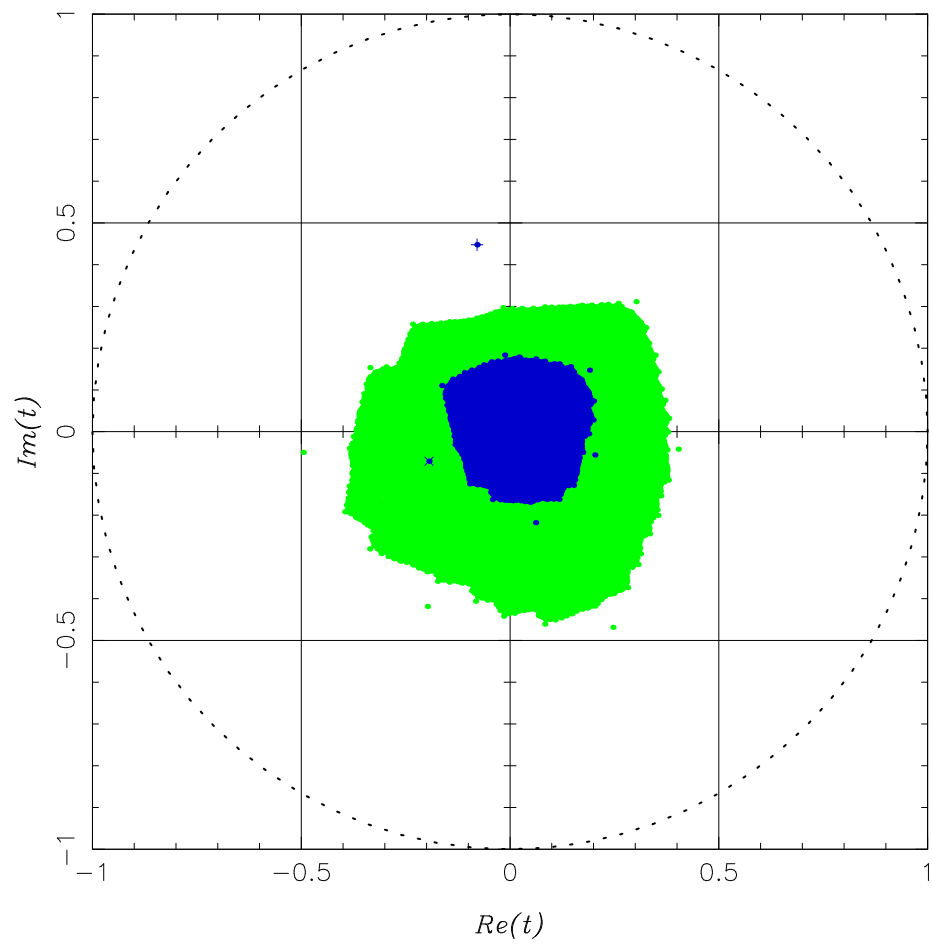

*Plot for  $q = 1.192 + 2.192 i$  ( $R = 2.200$ ,  $k = 085$ )*

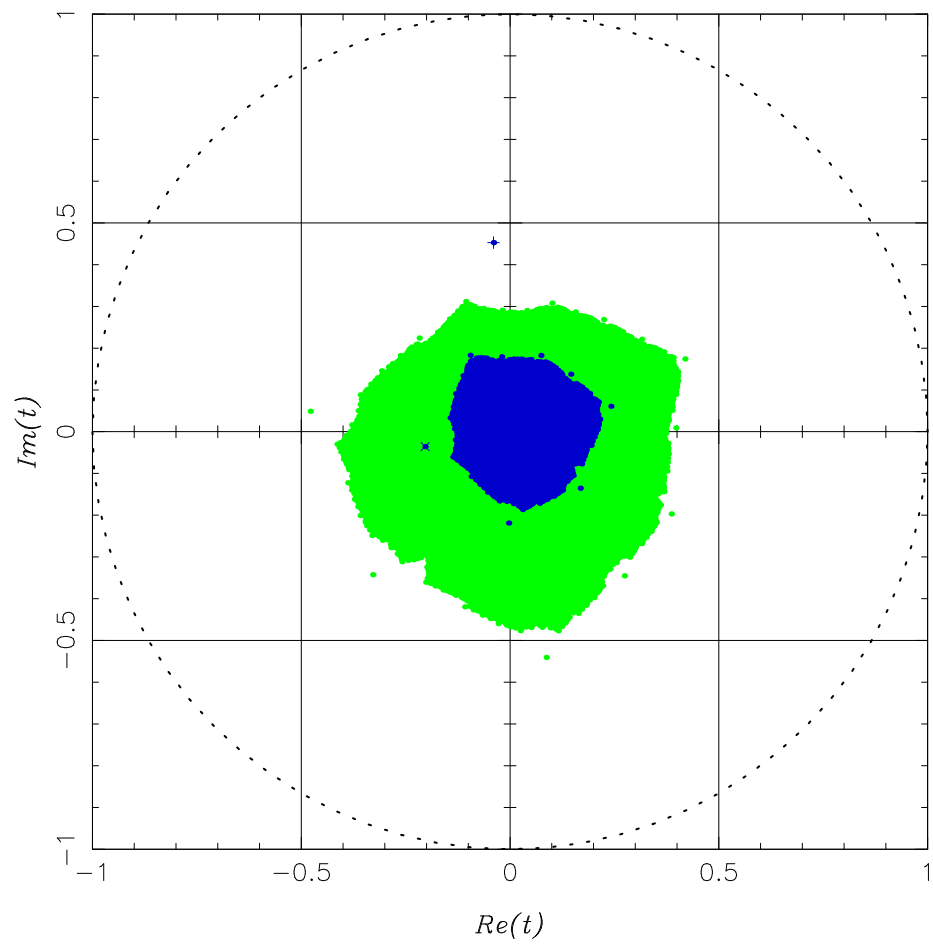

*Plot for  $q = 1.000 + 2.200\ i$  ( $R = 2.200$ ,  $k = 090$ )*

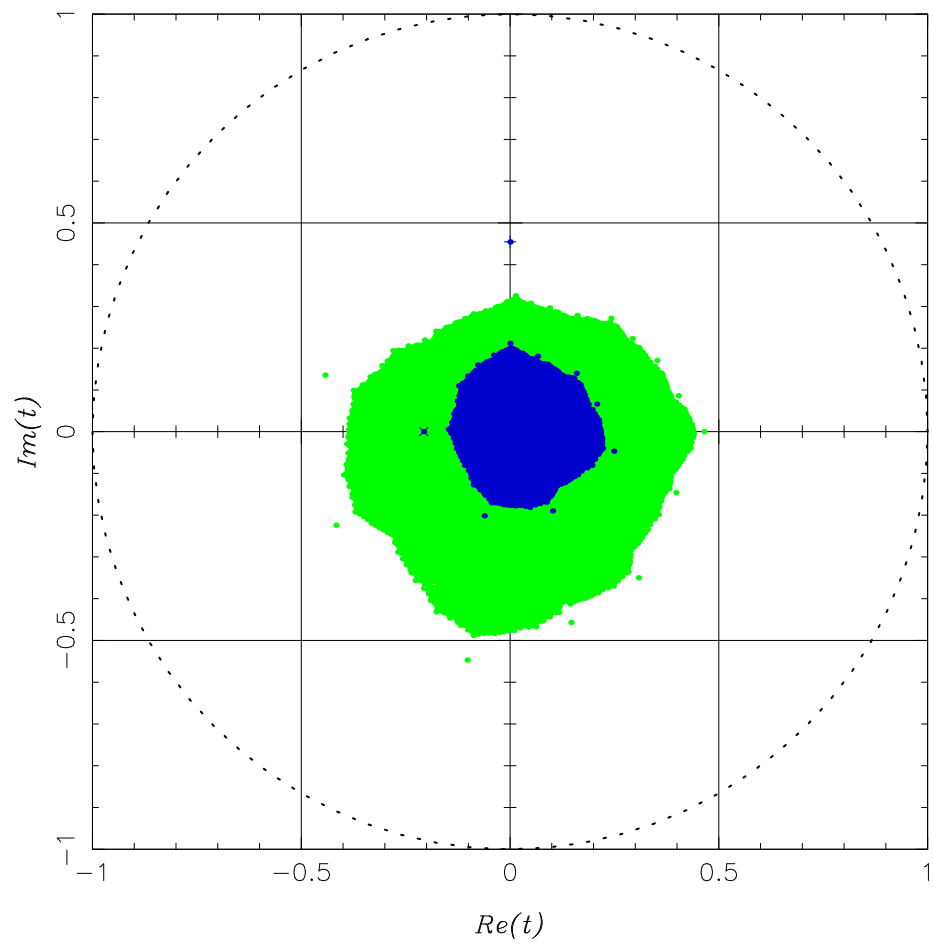

*Plot for  $q = 0.808 + 2.192 i$  ( $R = 2.200$ ,  $k = 095$ )*

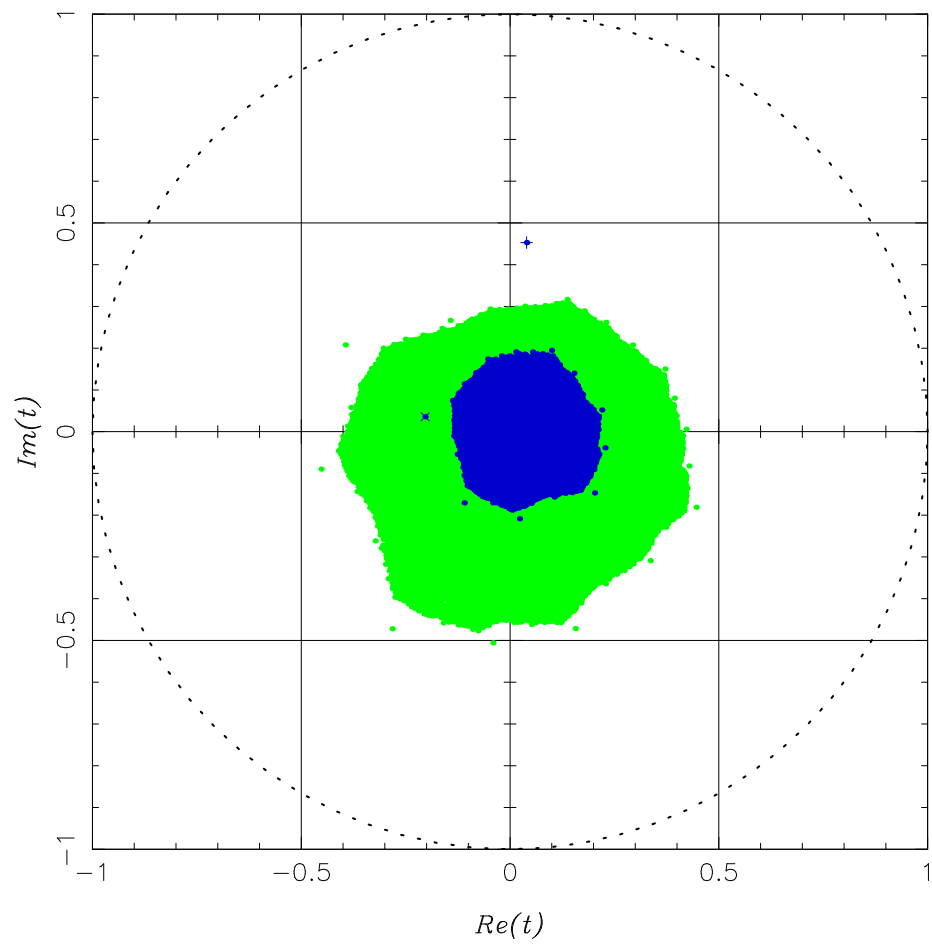

*Plot for  $q = 0.618 + 2.167 i$  ( $R = 2.200$ ,  $k = 100$ )*

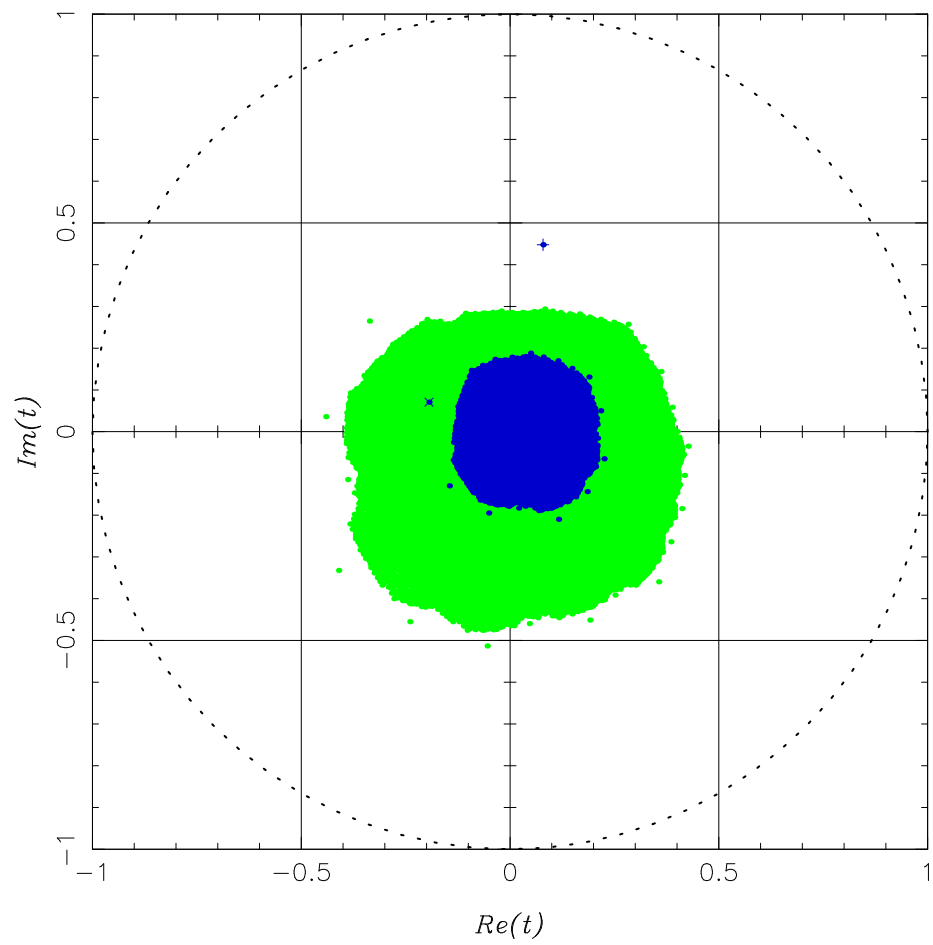

*Plot for  $q = 0.431 + 2.125 i$  ( $R = 2.200$ ,  $k = 105$ )*

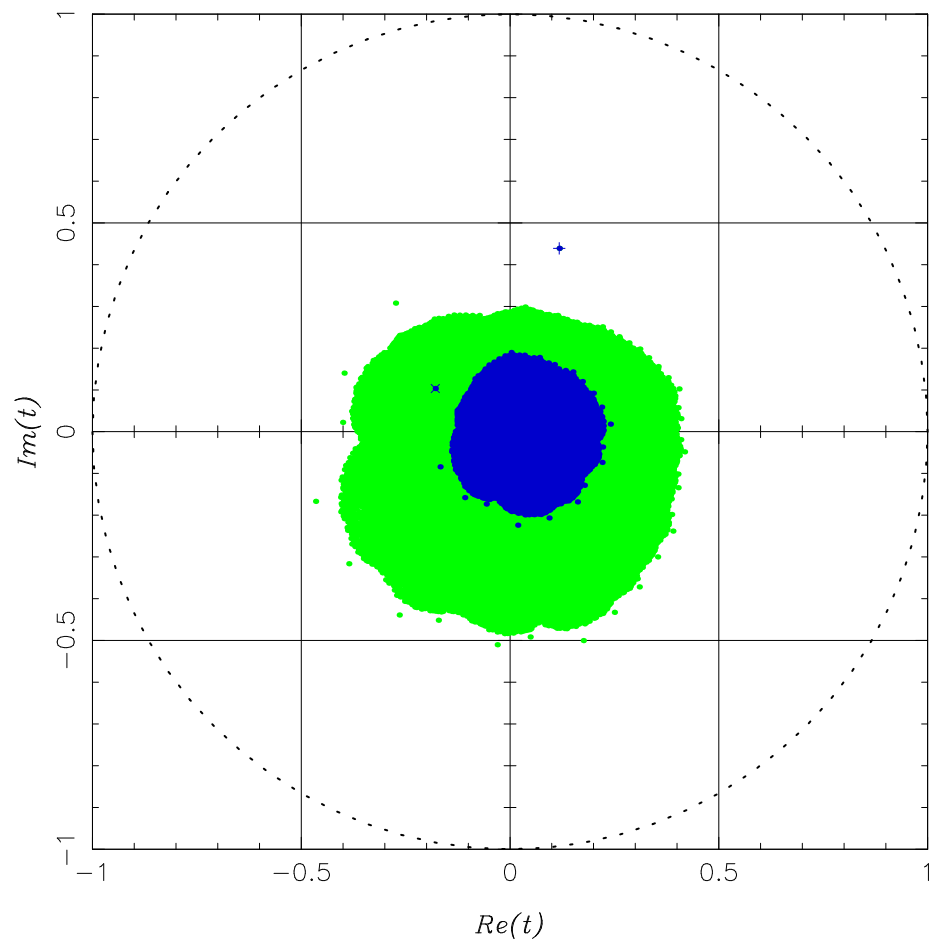

*Plot for  $q = 0.248 + 2.067 i$  ( $R = 2.200$ ,  $k = 110$ )*

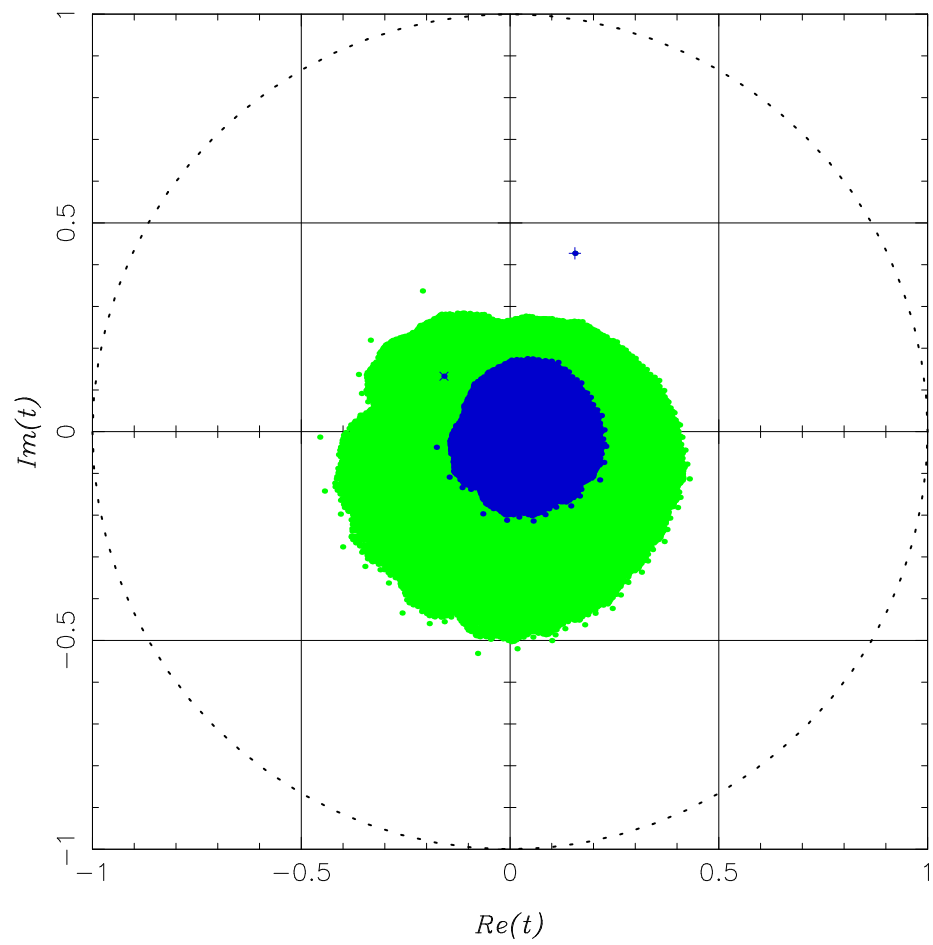



*Plot for  $q = 0.070 + 1.994 i$  ( $R = 2.200$ ,  $k = 115$ )*

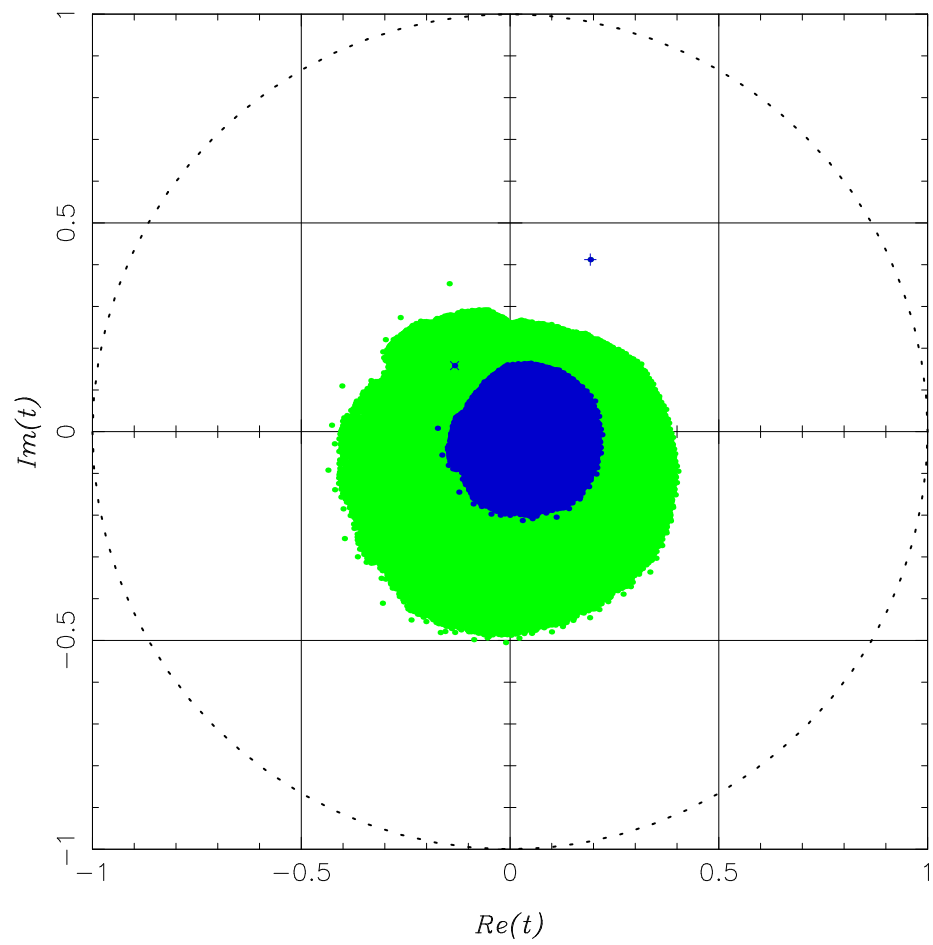

*Plot for  $q = -0.100 + 1.905 i$  ( $R = 2.200$ ,  $k = 120$ )*

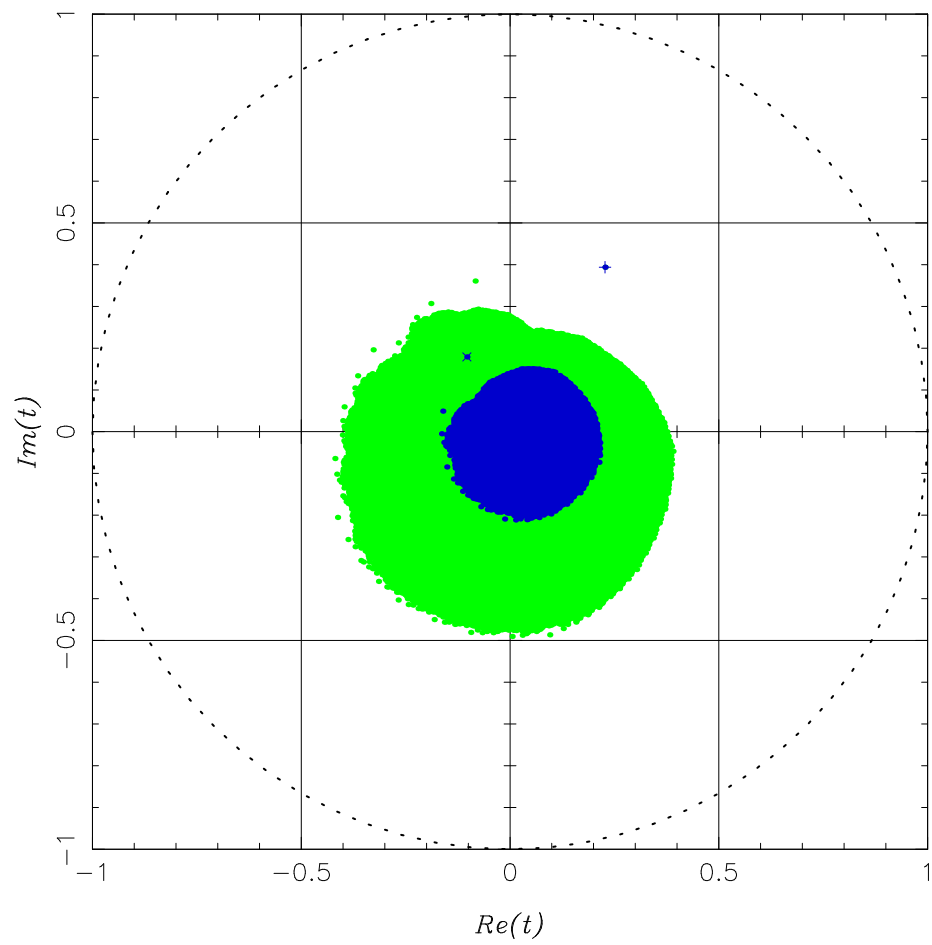

Plot for  $q = -0.262 + 1.802 i$  ( $R = 2.200$ ,  $k = 125$ )

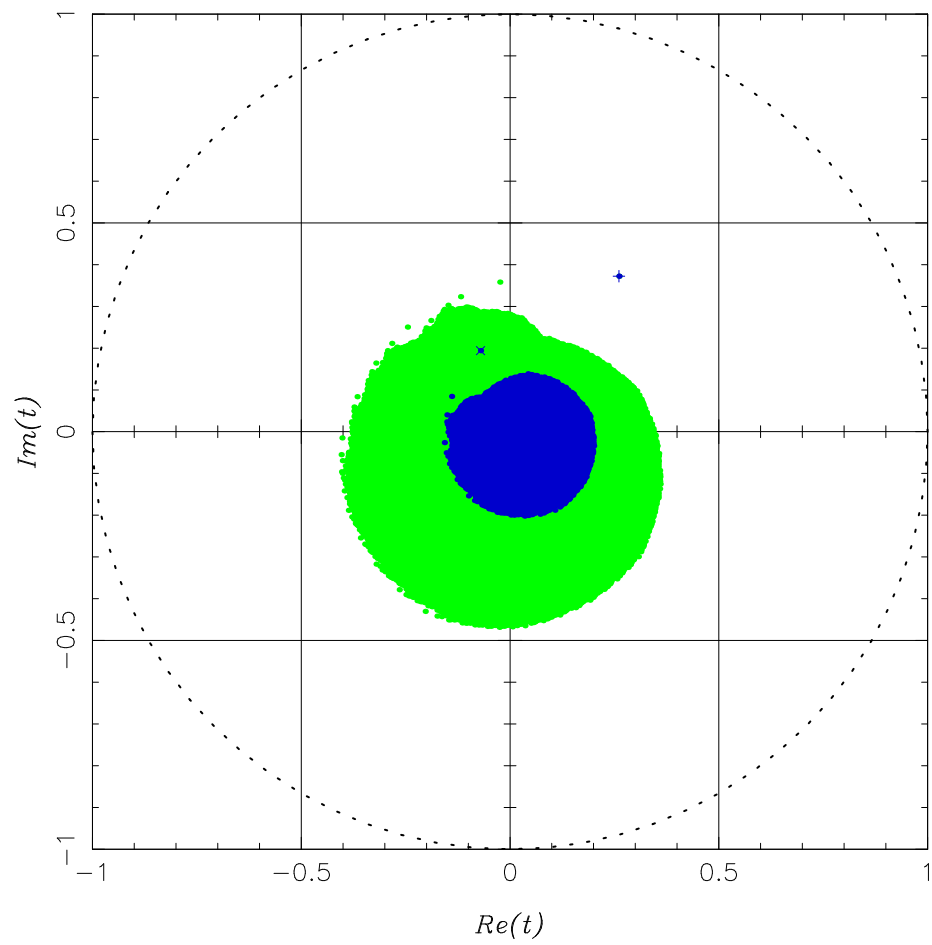

Plot for  $q = -0.414 + 1.685 i$  ( $R = 2.200$ ,  $k = 130$ )

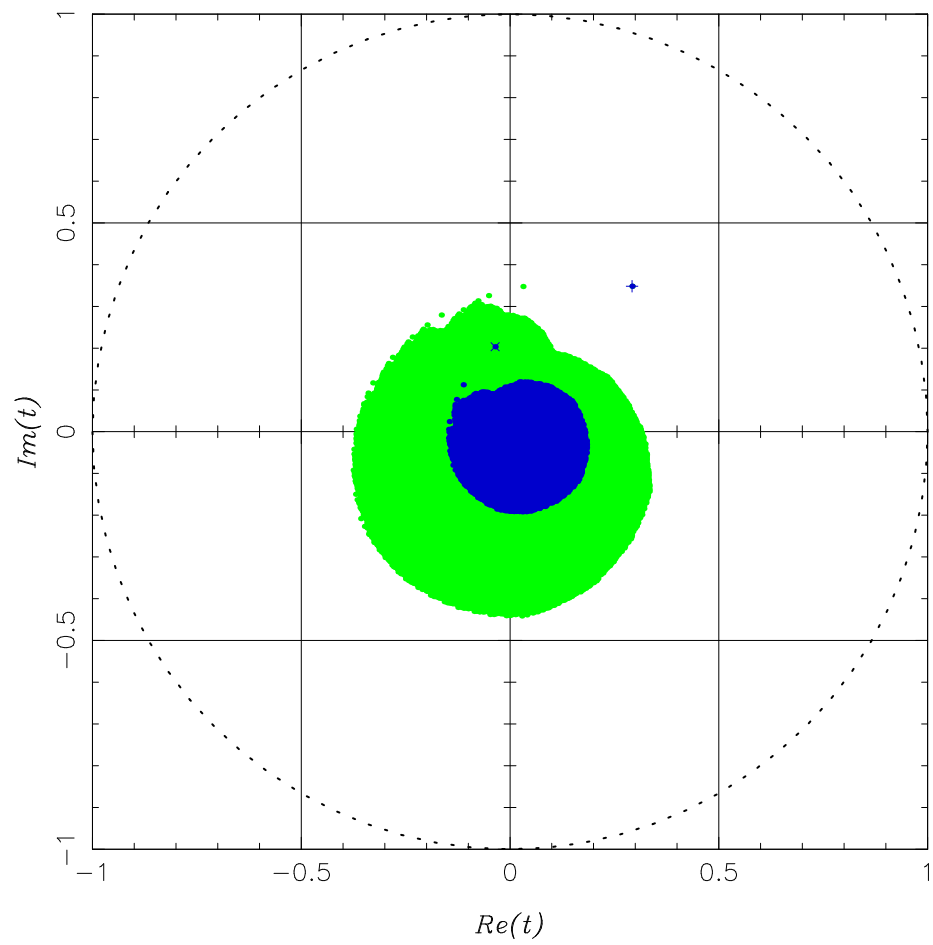

Plot for  $q = -0.556 + 1.556 i$  ( $R = 2.200$ ,  $k = 135$ )

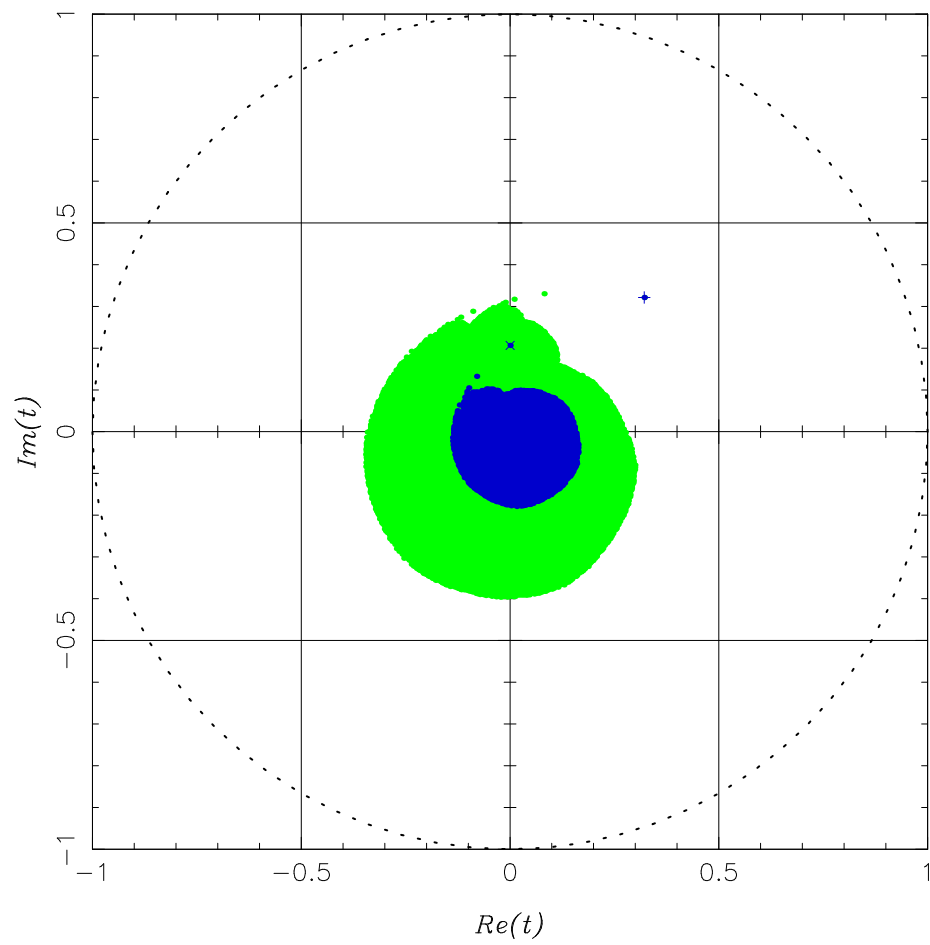

Plot for  $q = -0.685 + 1.414 i$  ( $R = 2.200$ ,  $k = 140$ )

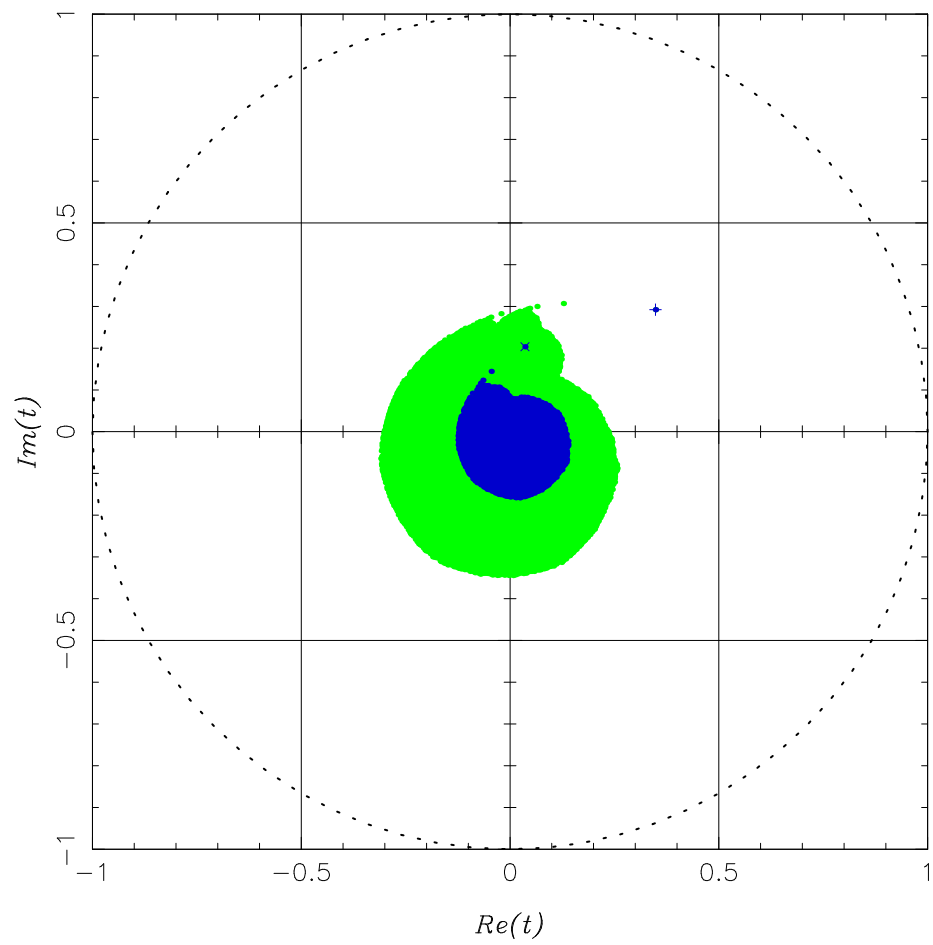

Plot for  $q = -0.802 + 1.262 i$  ( $R = 2.200$ ,  $k = 145$ )

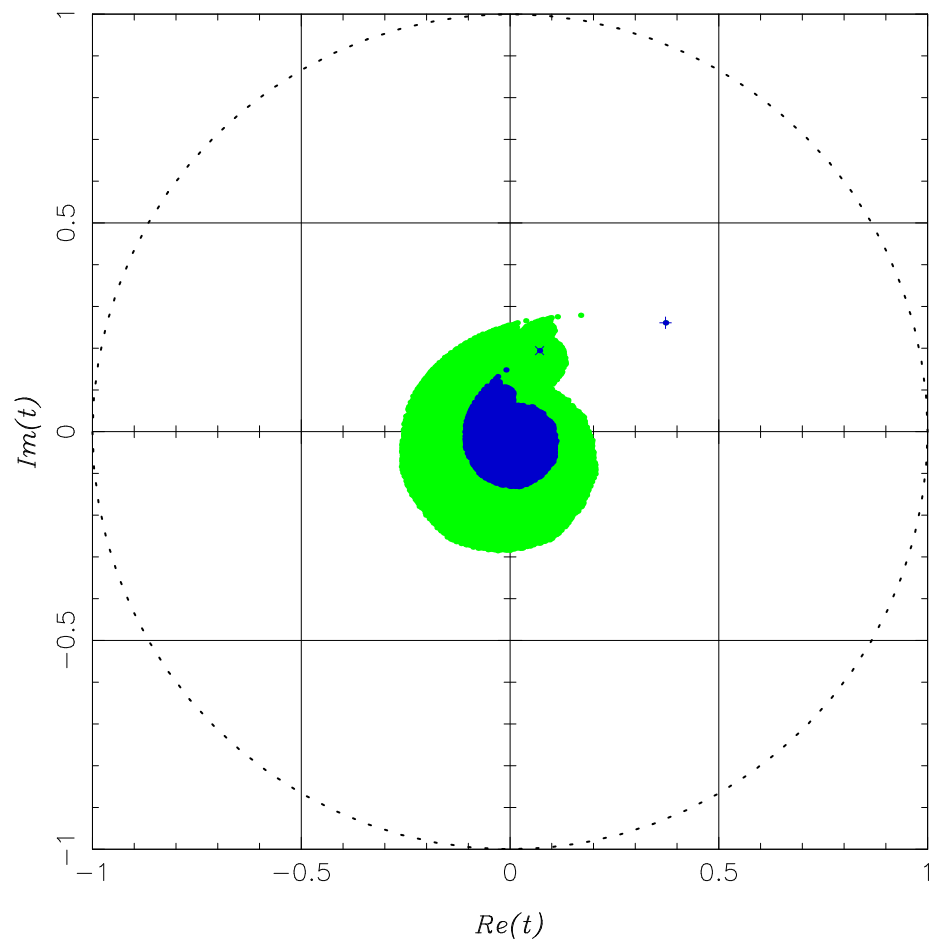

Plot for  $q = -0.905 + 1.100\ i$  ( $R = 2.200$ ,  $k = 150$ )

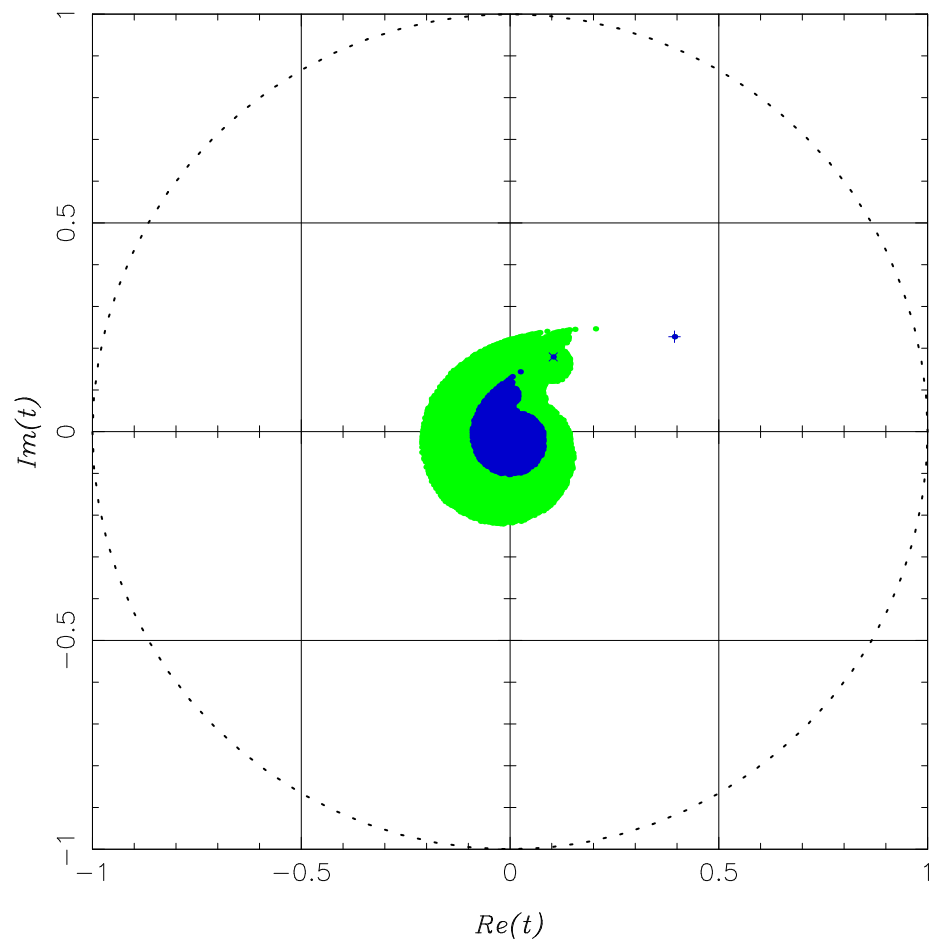



Plot for  $q = -0.994 + 0.930 i$  ( $R = 2.200$ ,  $k = 155$ )

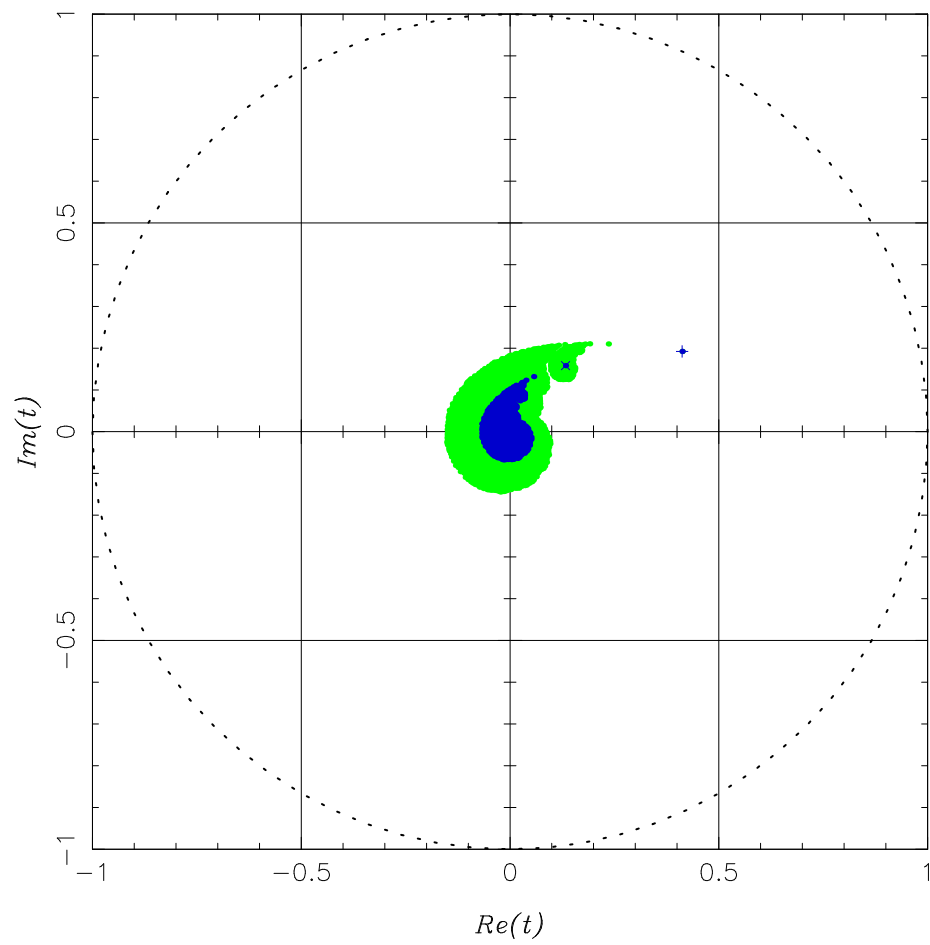

*Plot for  $q = -1.067 + 0.752 i$  ( $R = 2.200$ ,  $k = 160$ )*

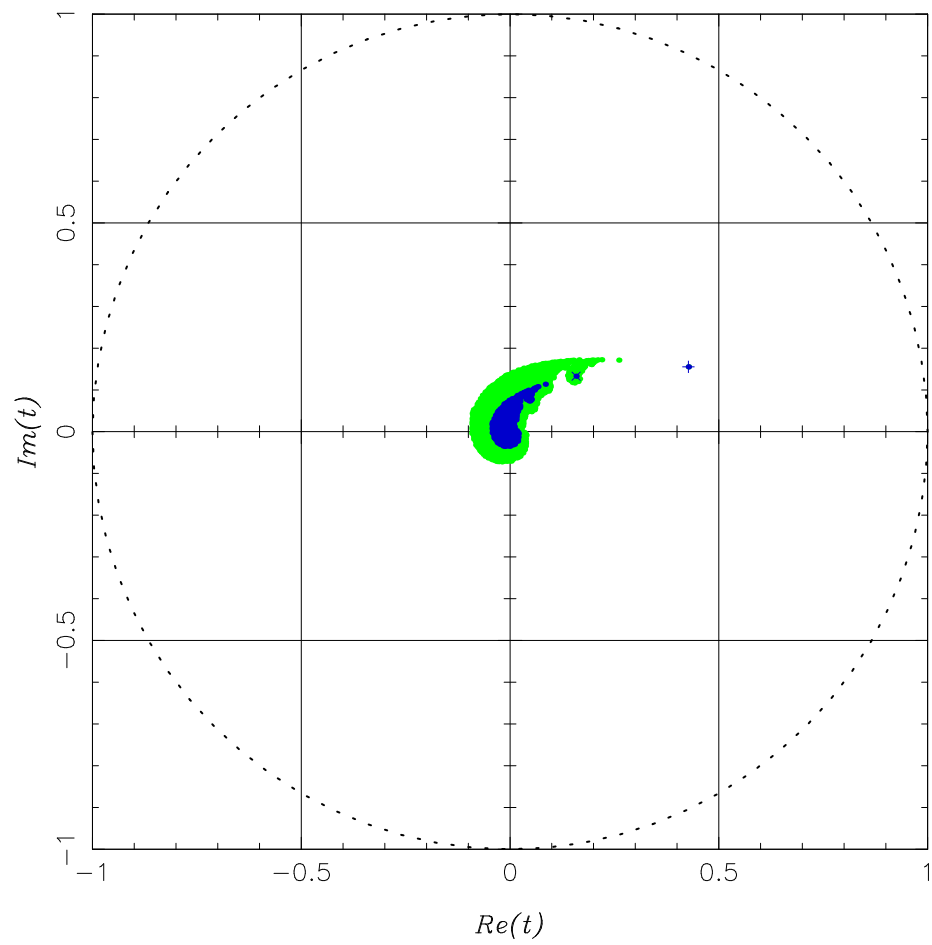

*Plot for  $q = -1.125 + 0.569 i$  ( $R = 2.200$ ,  $k = 165$ )*

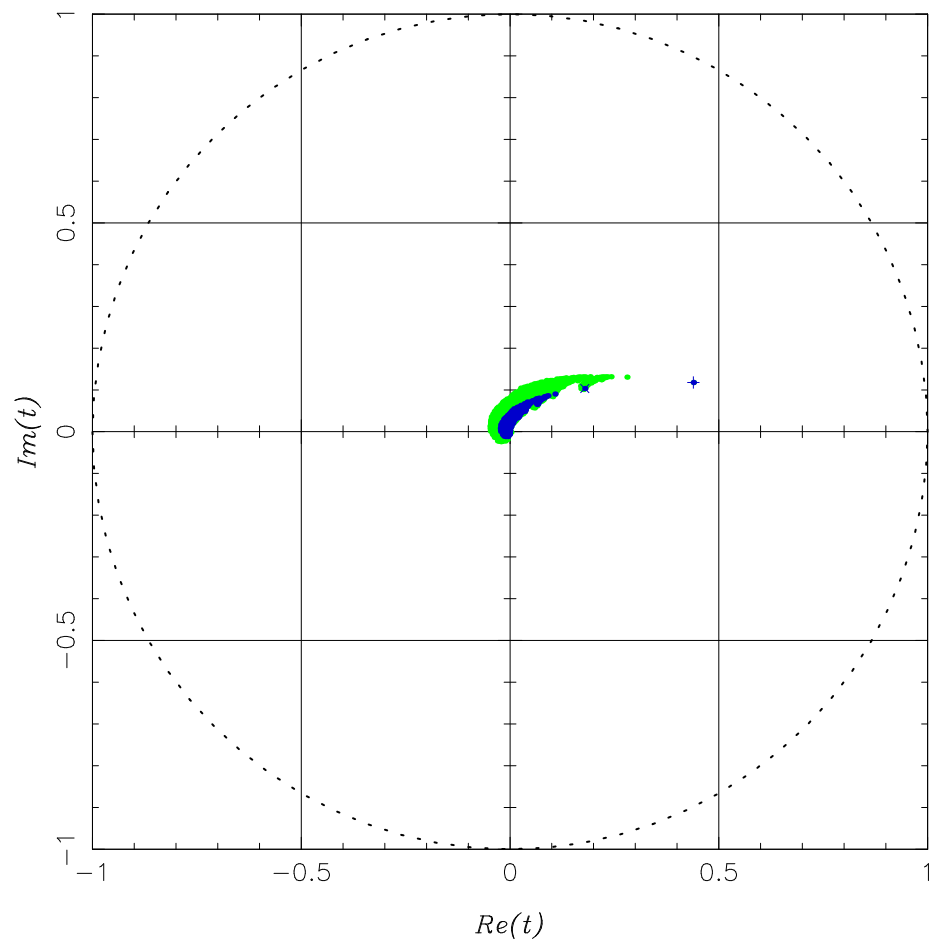

Plot for  $q = -1.167 + 0.382 i$  ( $R = 2.200$ ,  $k = 170$ )

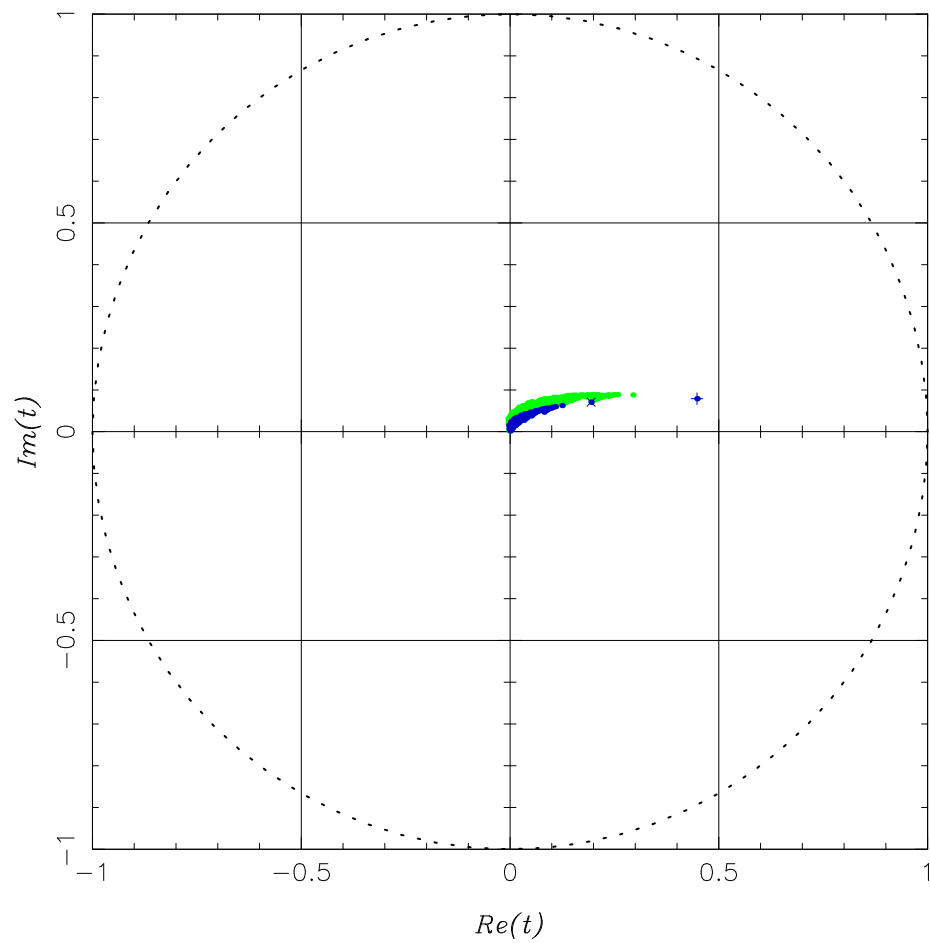

Plot for  $q = -1.192 + 0.192 i$  ( $R = 2.200$ ,  $k = 175$ )

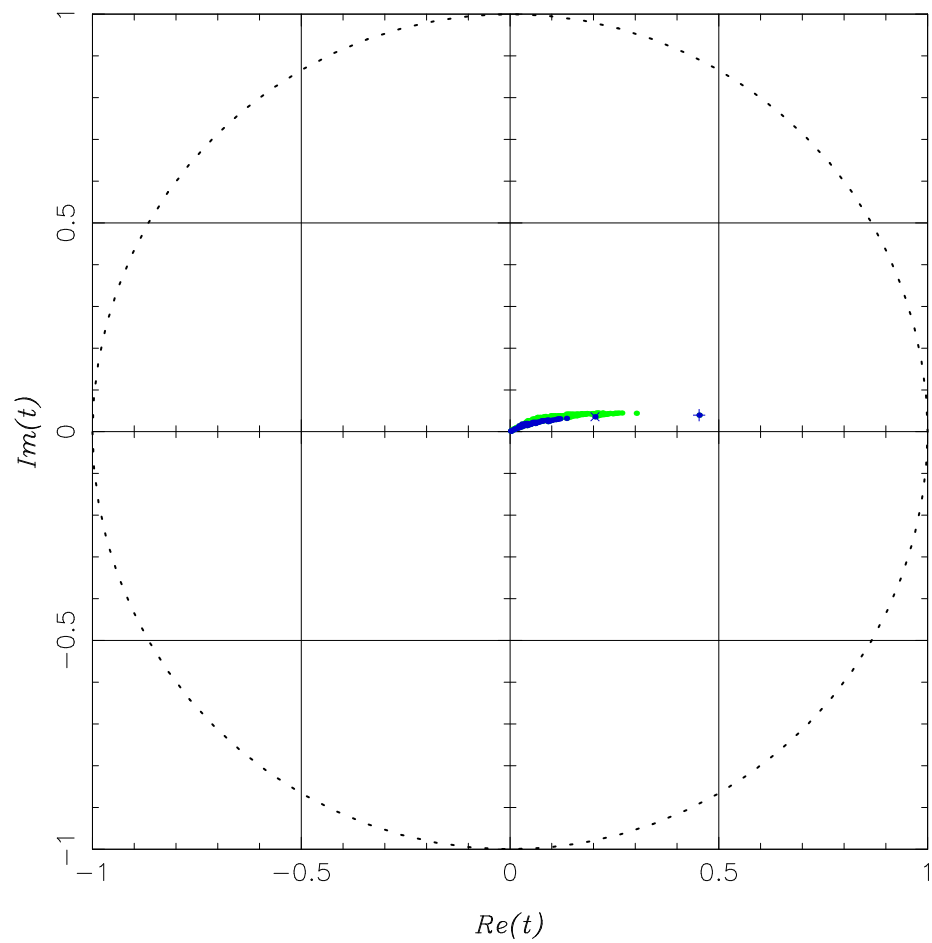

Plot for  $q = -1.200 + 0.000\ i$  ( $R = 2.200$ ,  $k = 180$ )

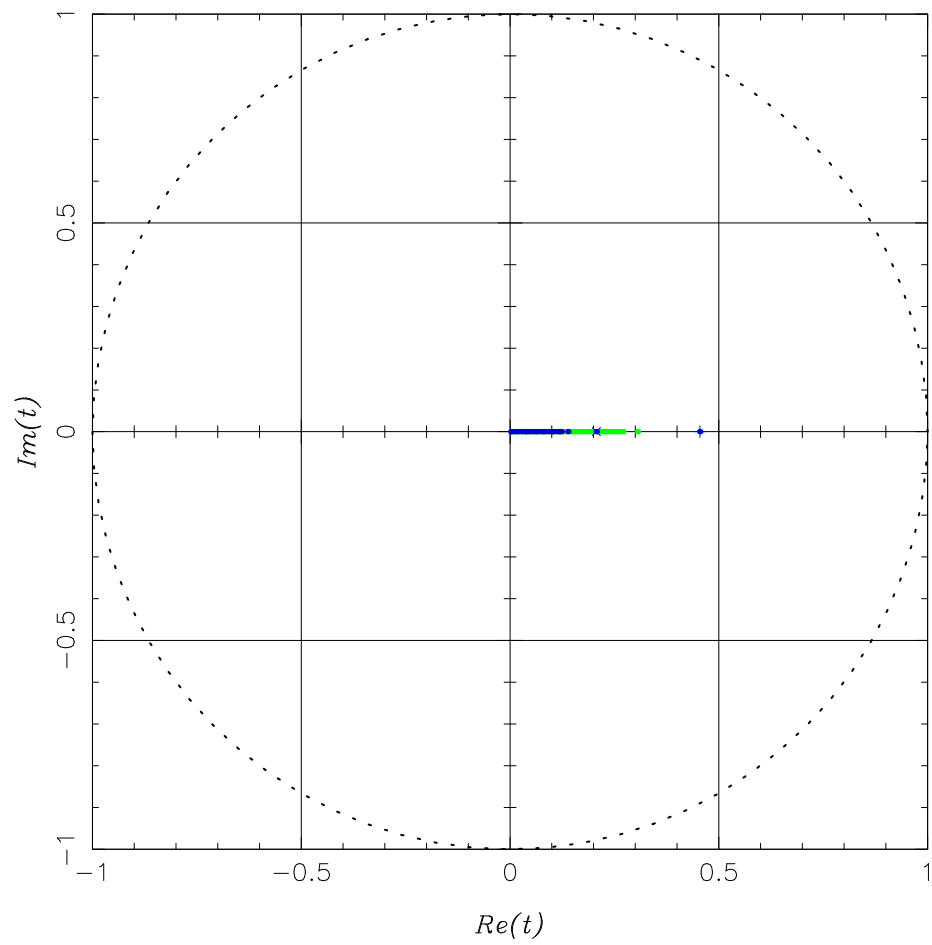

Supplement: Supplementary file 1 [file S1S2_2.2.pdf]
