# Supplementary material for: Linear bound in terms of maxmaxflow for the chromatic roots of series-parallel graphs
Source: arXiv:1307.1721 ancillary file (2013-07-05)

## Approximate shapes of $S_1$ and $S_2$ for $R = 2.4$

This document contains supporting plots for the paper “*Linear bound in terms of maxmaxflow for the chromatic roots of series-parallel graphs*” by Gordon Royle and Alan Sokal.

Each of the following pages contains a single plot showing the approximations for the sets  $S_1$  and  $S_2$  for a particular value of  $q$ . The chosen values of  $q$  all lie on the circle  $|q - 1| = 2.4$  and are spaced equally around the circle in increments of 5 degree. Thus for  $k = 0, 5, 10, \dots, 180$ , there are plots for each  $q$  of the form  $q = 1 + 2.4e^{2\pi i(k/360)}$ .

Each plot shows in light-green the approximation for  $S_2$  and in dark-blue the approximation for  $S_1$ . The important points  $t_0 = 1/(1-q)$  and  $t_0^2$  are marked by a + and a  $\times$  respectively. If the true regions  $S_1$  and  $S_2$  are contained completely within the circle  $|t| = 1$  then this certifies that  $q$  is not a chromatic root for any series-parallel graph of maxmaxflow  $\Lambda = 3$ .

*Plot for  $q = 3.400 + 0.000\ i$  ( $R = 2.400$ ,  $k = 000$ )*

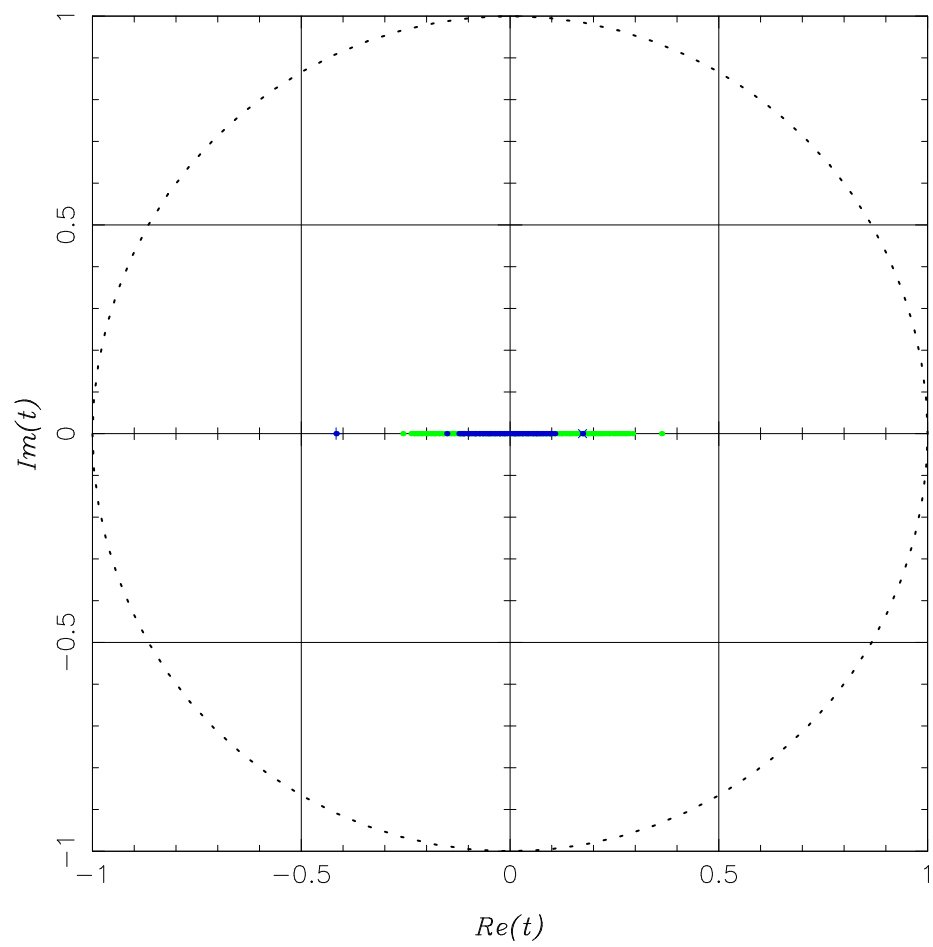

*Plot for  $q = 3.391 + 0.209 i$  ( $R = 2.400$ ,  $k = 005$ )*

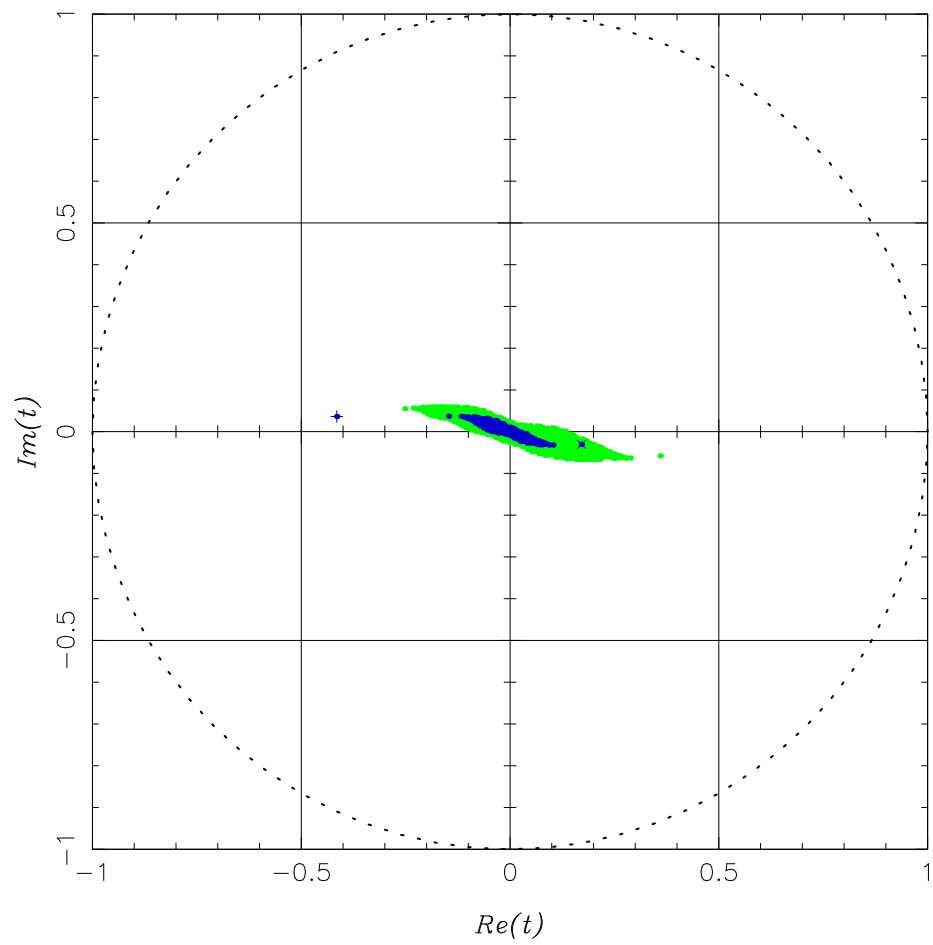

*Plot for  $q = 3.364 + 0.417 i$  ( $R = 2.400$ ,  $k = 010$ )*

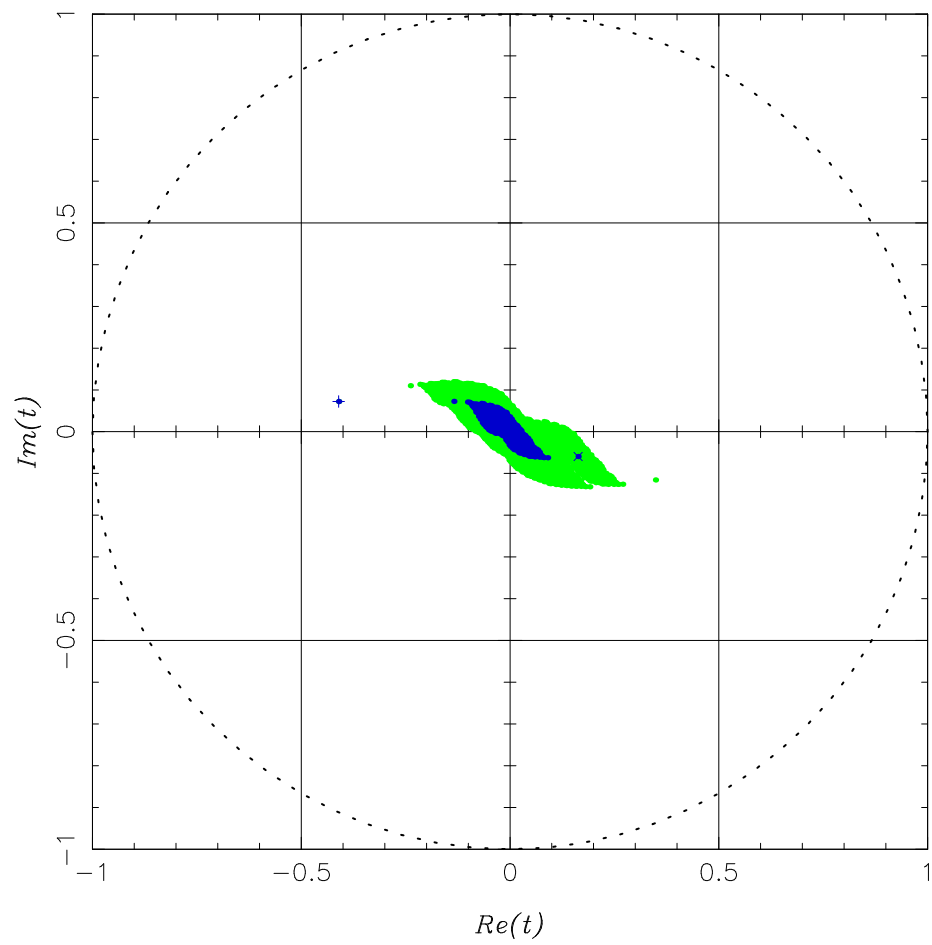

*Plot for  $q = 3.318 + 0.621 i$  ( $R = 2.400$ ,  $k = 015$ )*

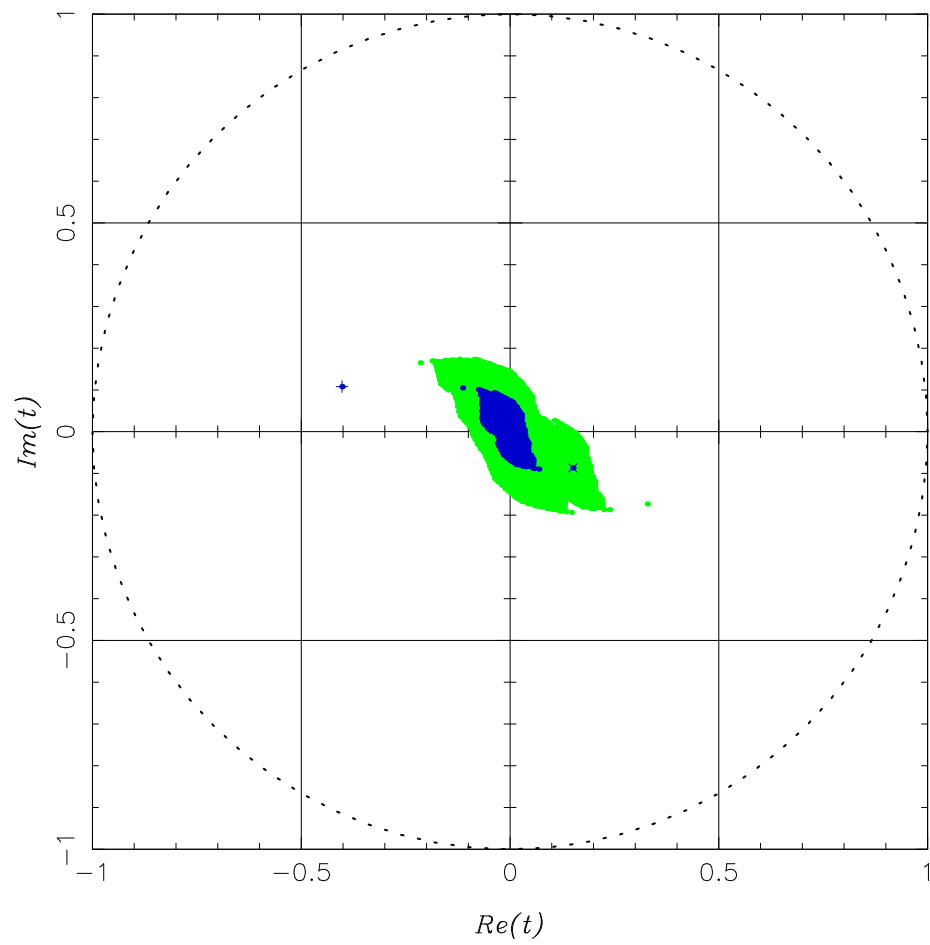

*Plot for  $q = 3.255 + 0.821 i$  ( $R = 2.400$ ,  $k = 020$ )*

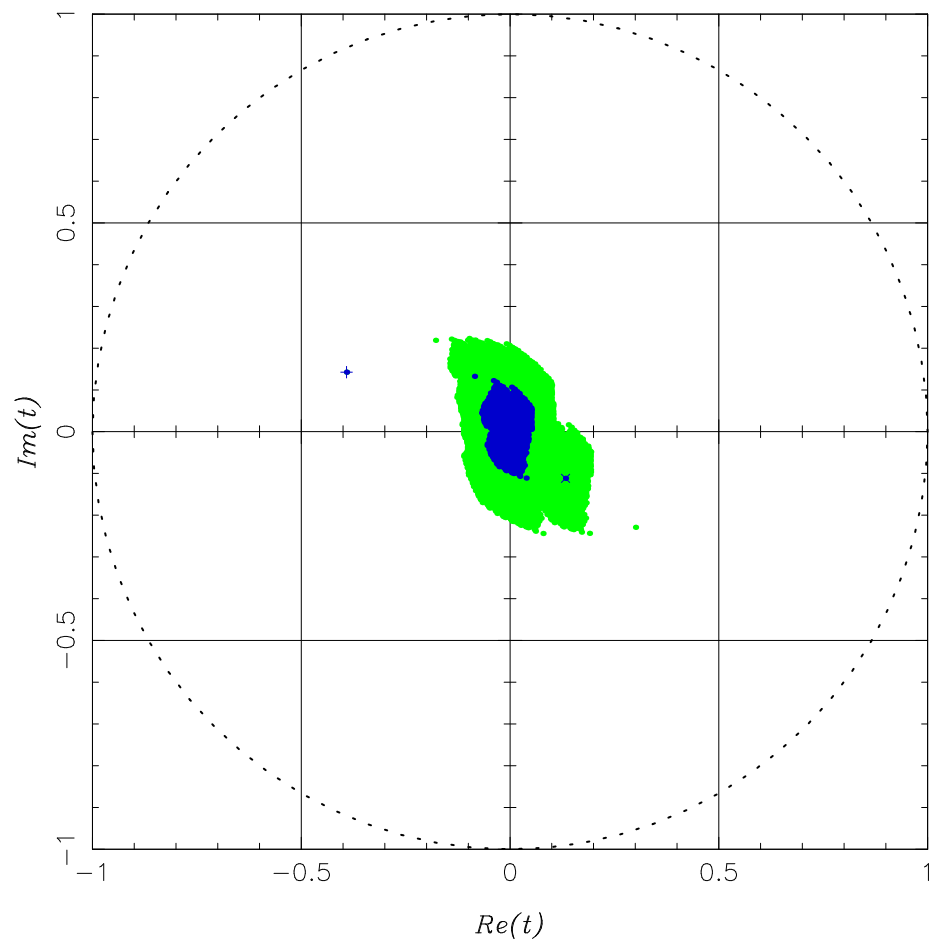

*Plot for  $q = 3.175 + 1.014 i$  ( $R = 2.400$ ,  $k = 025$ )*

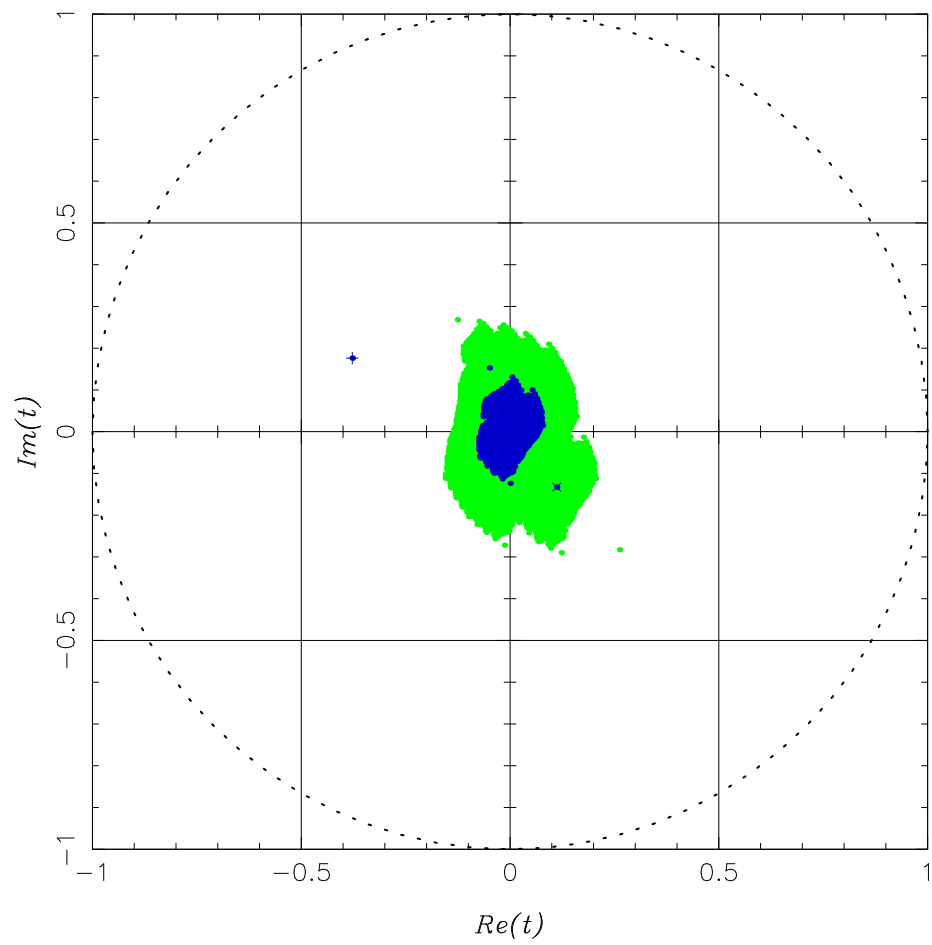

*Plot for  $q = 3.078 + 1.200\ i$  ( $R = 2.400$ ,  $k = 030$ )*

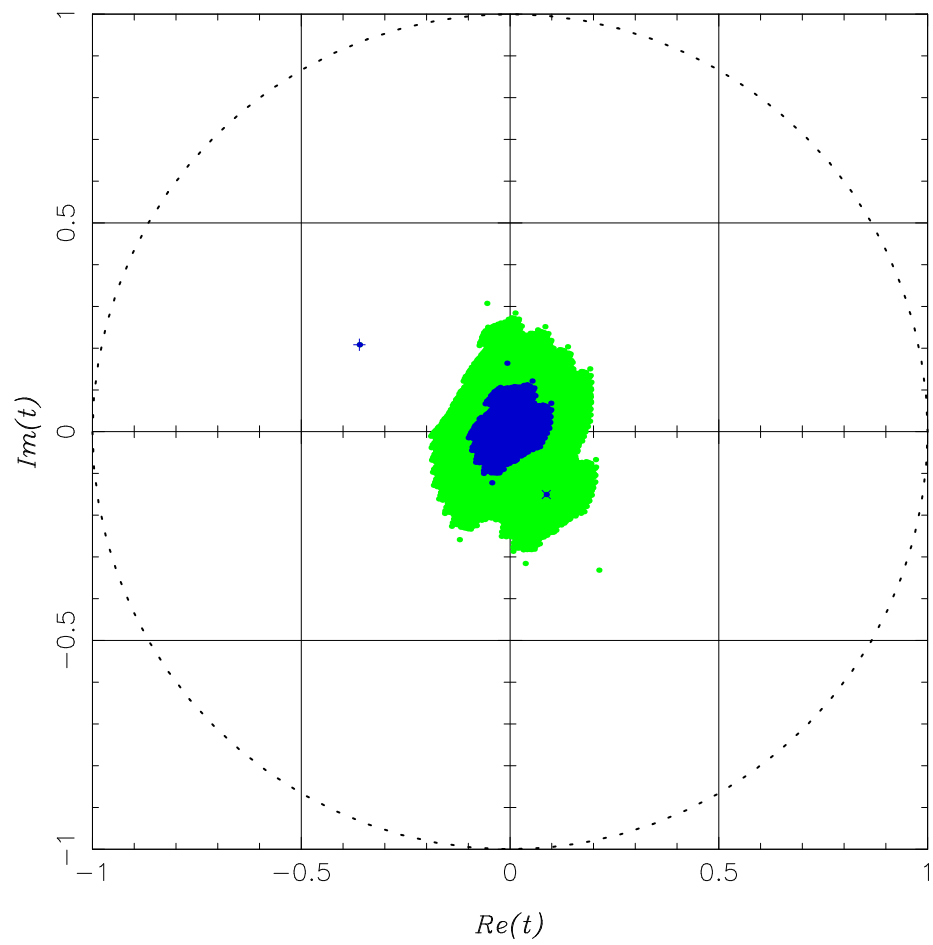



*Plot for  $q = 2.966 + 1.377 i$  ( $R = 2.400$ ,  $k = 035$ )*

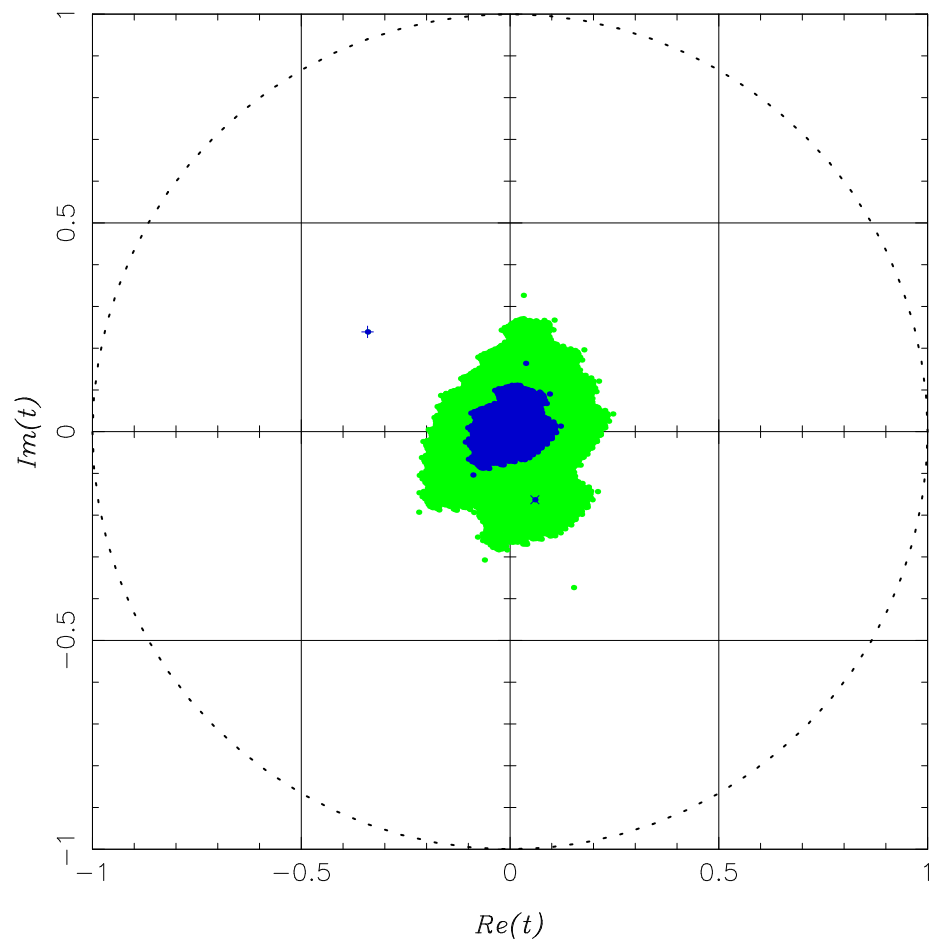

*Plot for  $q = 2.839 + 1.543 i$  ( $R = 2.400$ ,  $k = 040$ )*

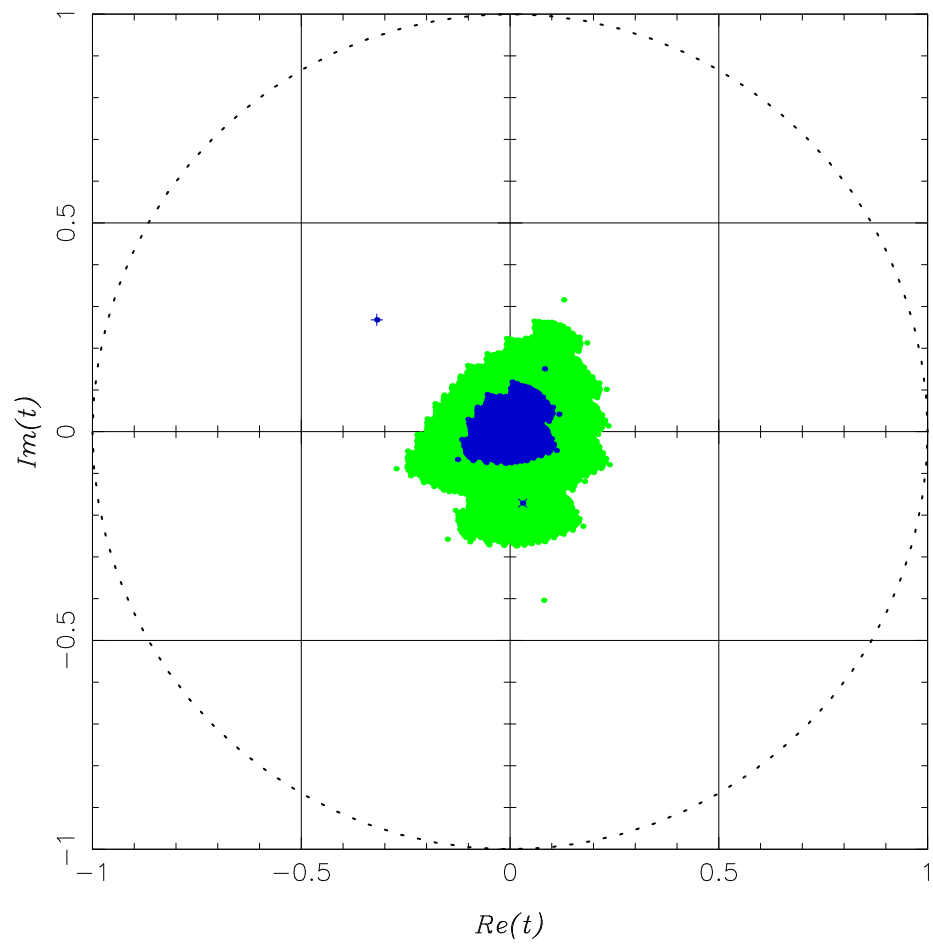

*Plot for  $q = 2.697 + 1.697 i$  ( $R = 2.400$ ,  $k = 045$ )*

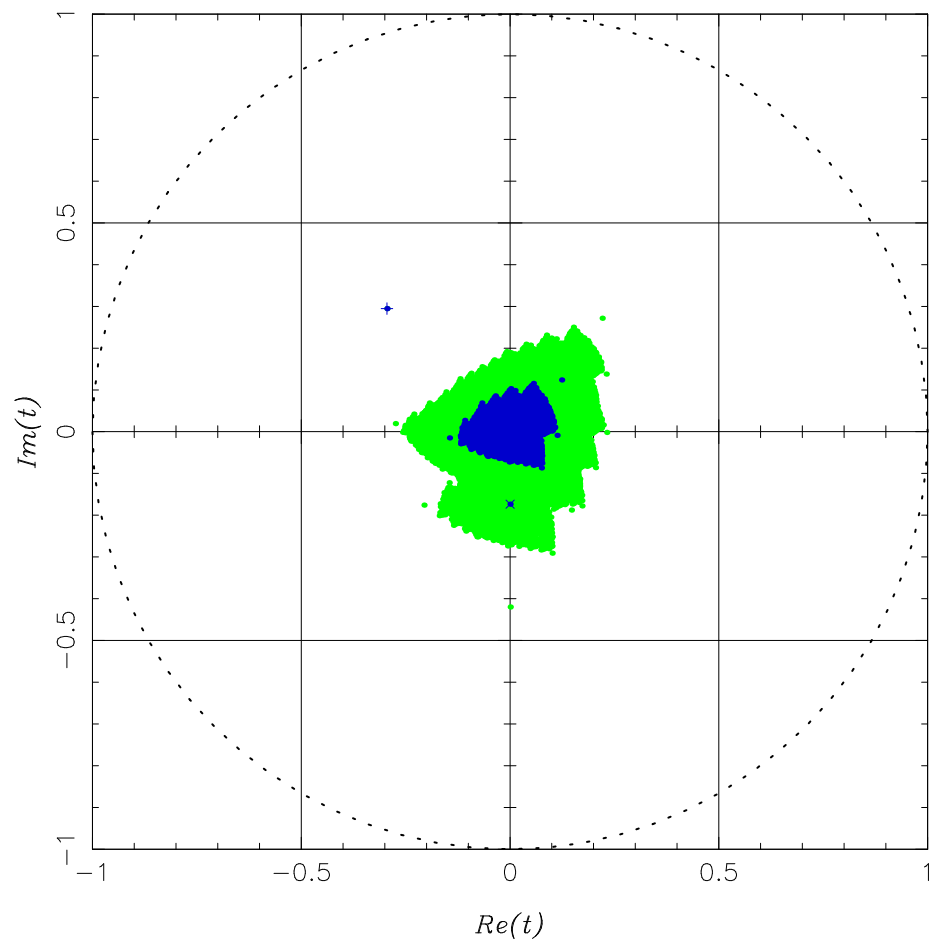

*Plot for  $q = 2.543 + 1.839 i$  ( $R = 2.400$ ,  $k = 050$ )*

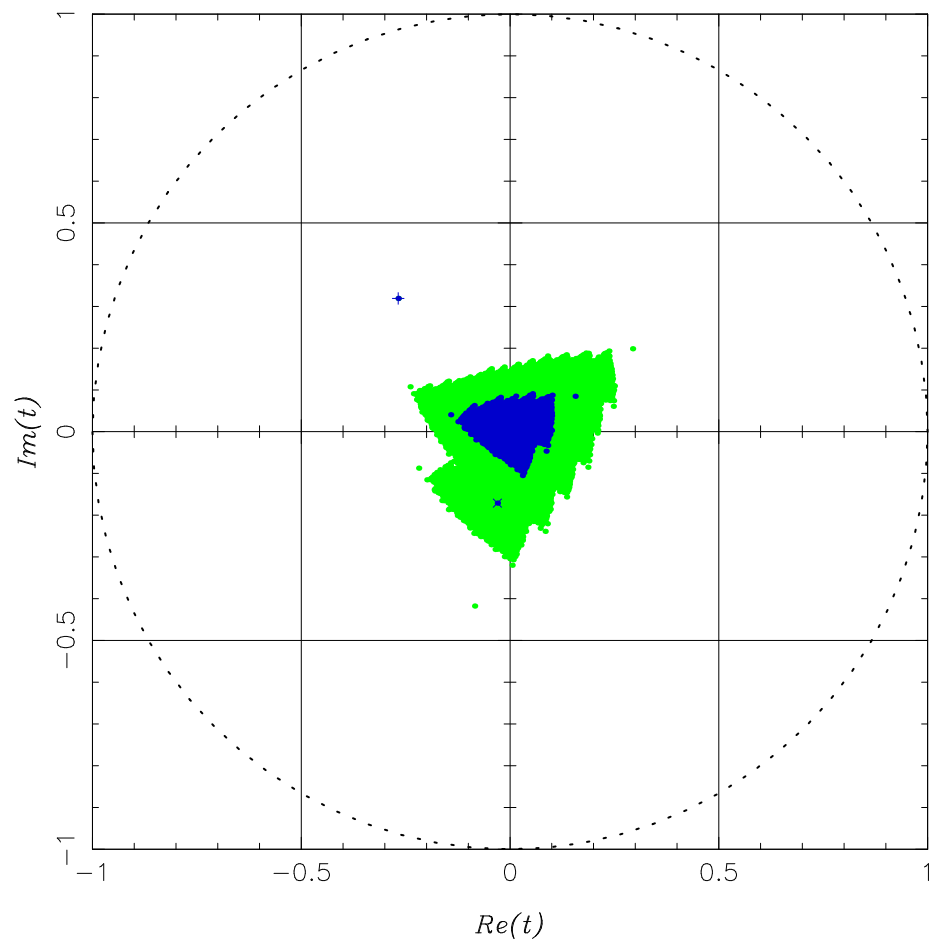

*Plot for  $q = 2.377 + 1.966 i$  ( $R = 2.400$ ,  $k = 055$ )*

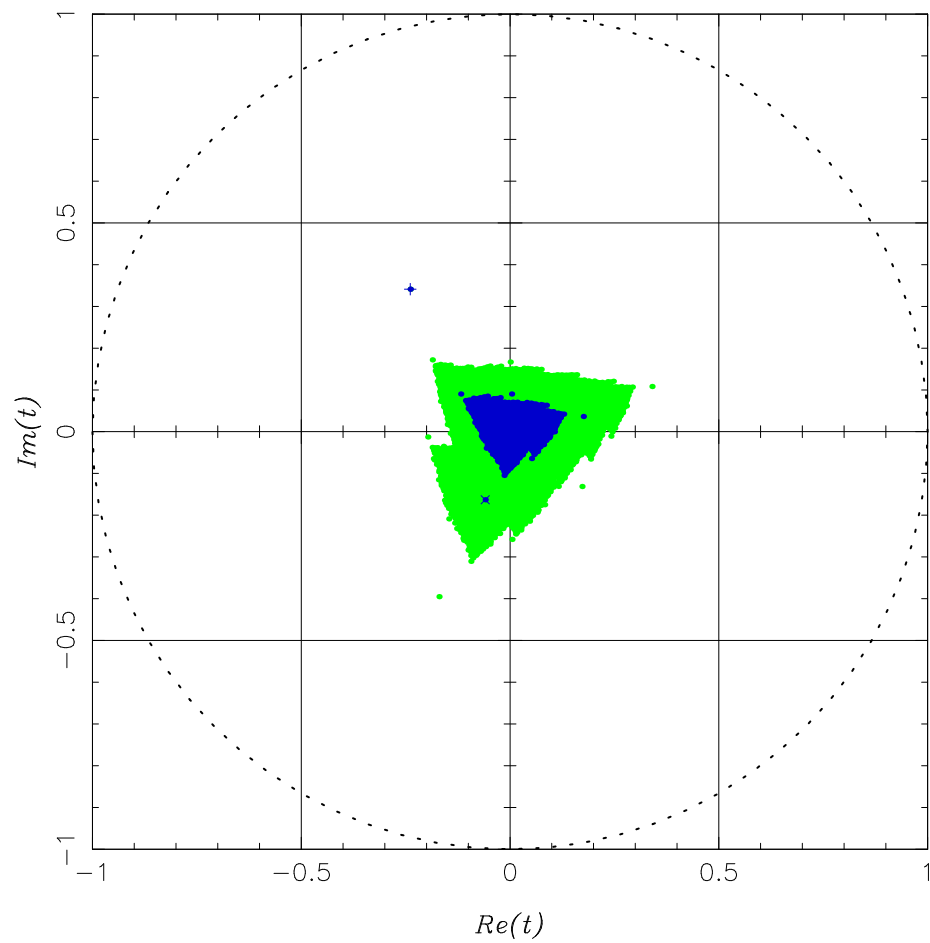

*Plot for  $q = 2.200 + 2.078 i$  ( $R = 2.400$ ,  $k = 060$ )*

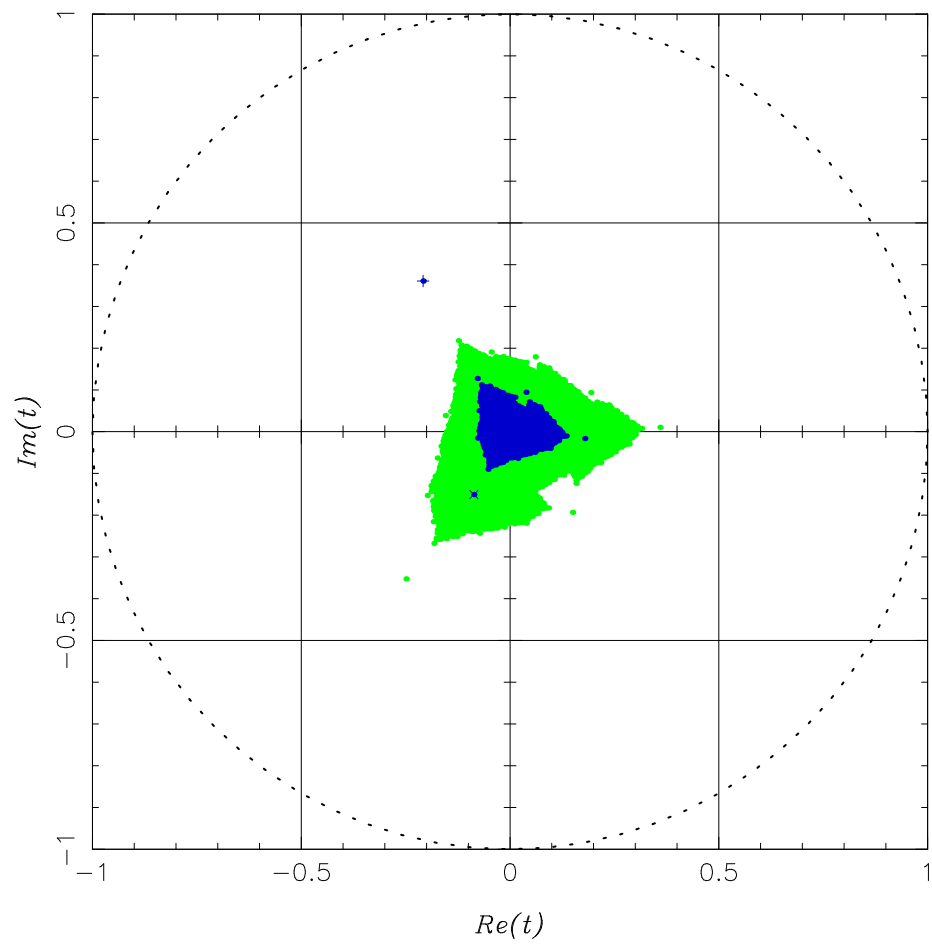

*Plot for  $q = 2.014 + 2.175 i$  ( $R = 2.400$ ,  $k = 065$ )*

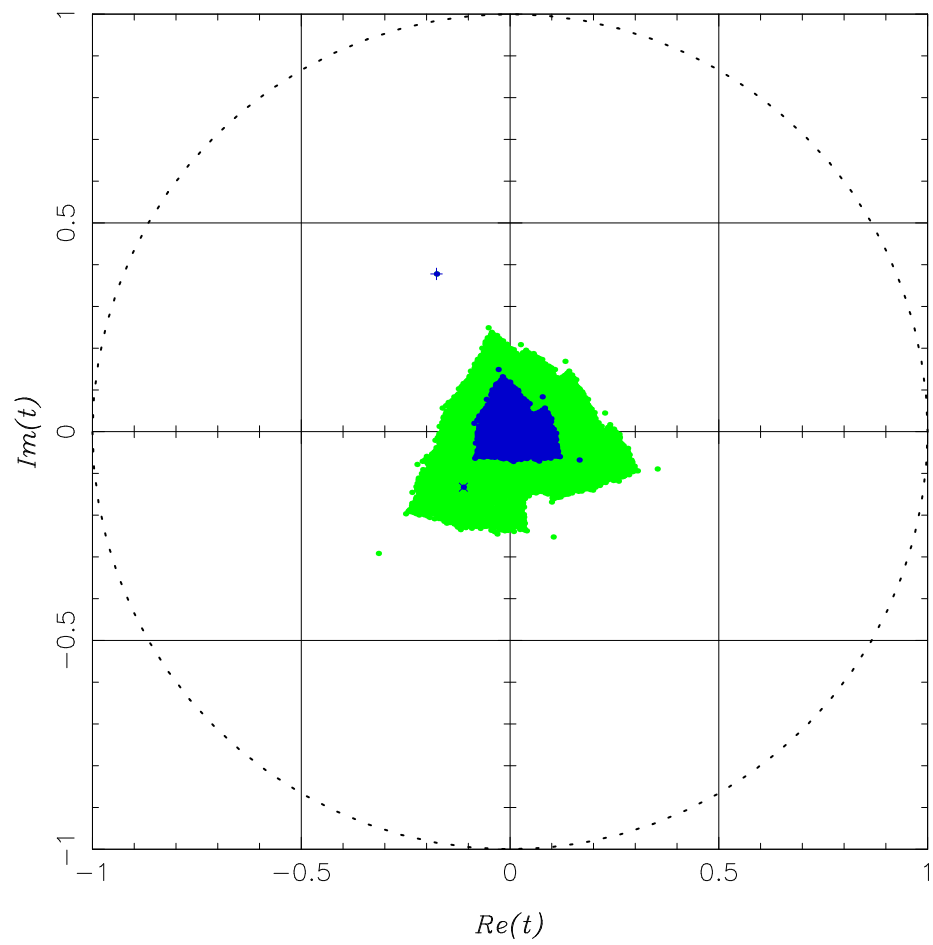

*Plot for  $q = 1.821 + 2.255 i$  ( $R = 2.400$ ,  $k = 070$ )*

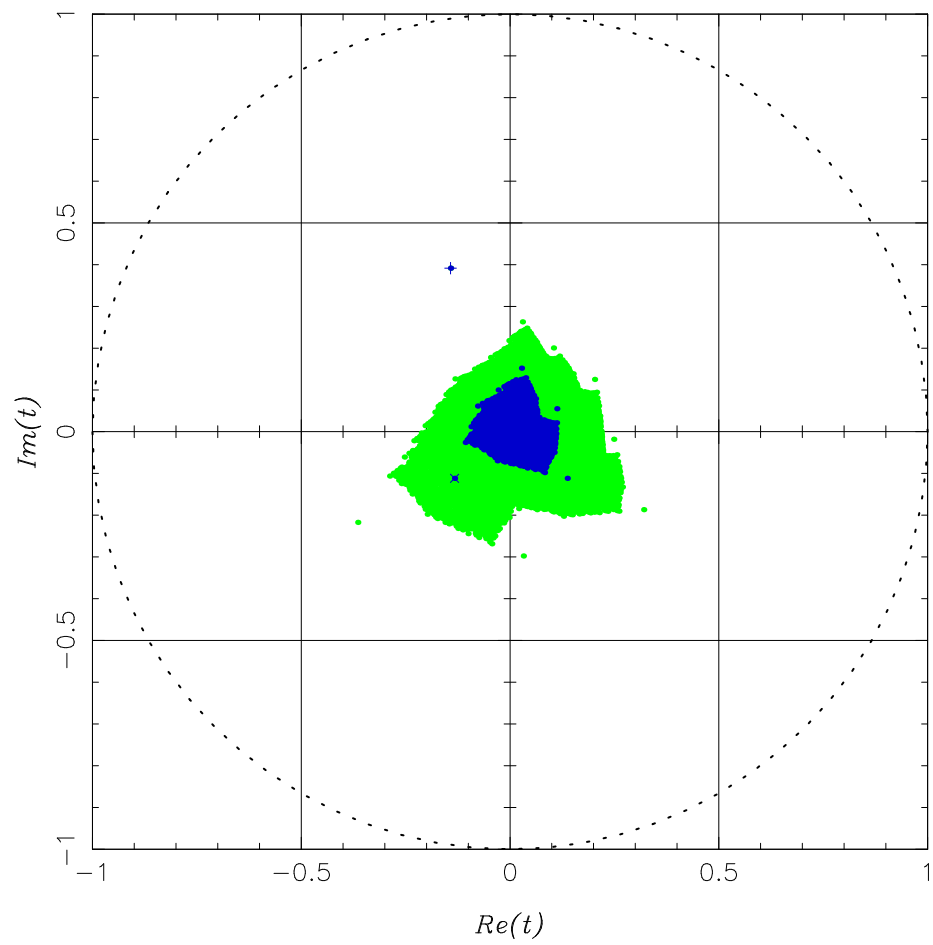



*Plot for  $q = 1.621 + 2.318 i$  ( $R = 2.400$ ,  $k = 075$ )*

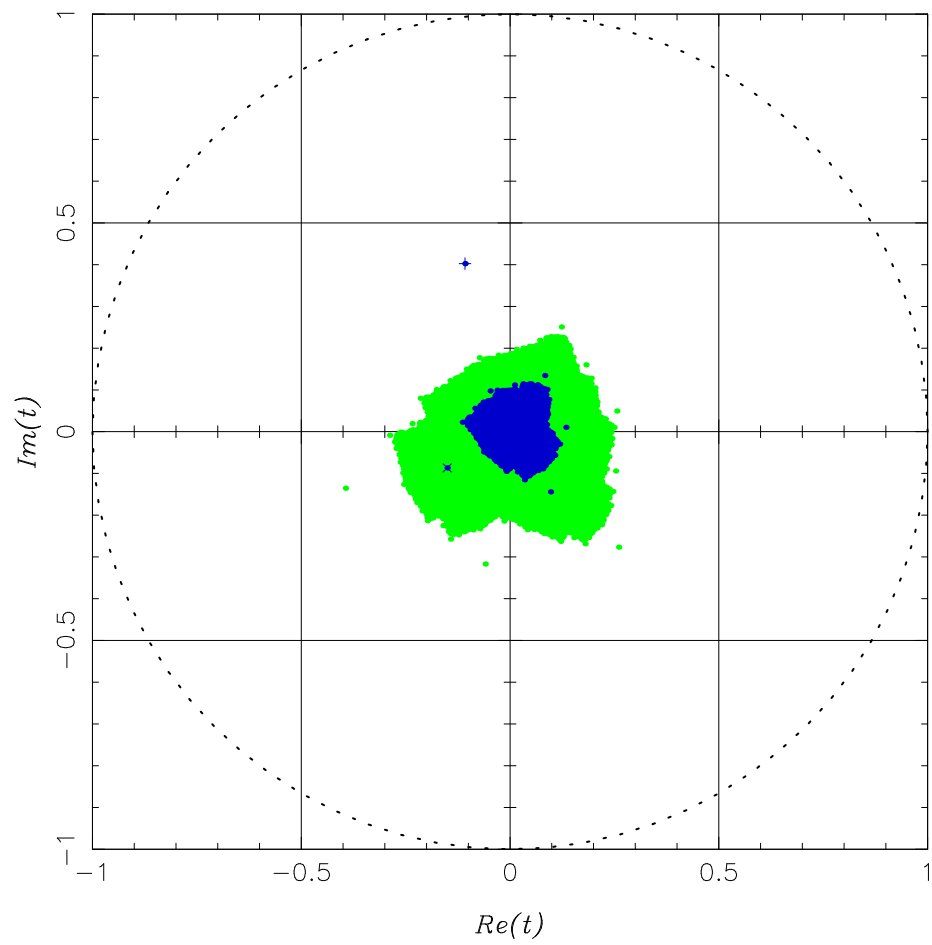

*Plot for  $q = 1.417 + 2.364 i$  ( $R = 2.400$ ,  $k = 080$ )*

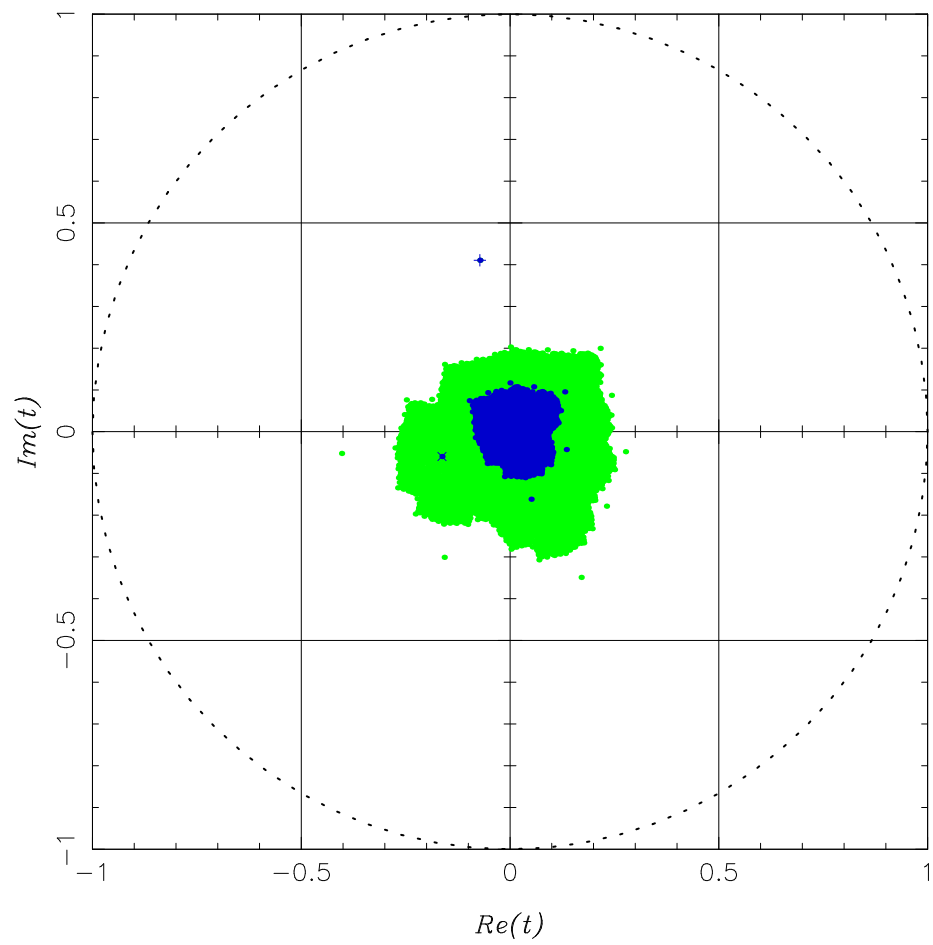

*Plot for  $q = 1.209 + 2.391 i$  ( $R = 2.400$ ,  $k = 085$ )*

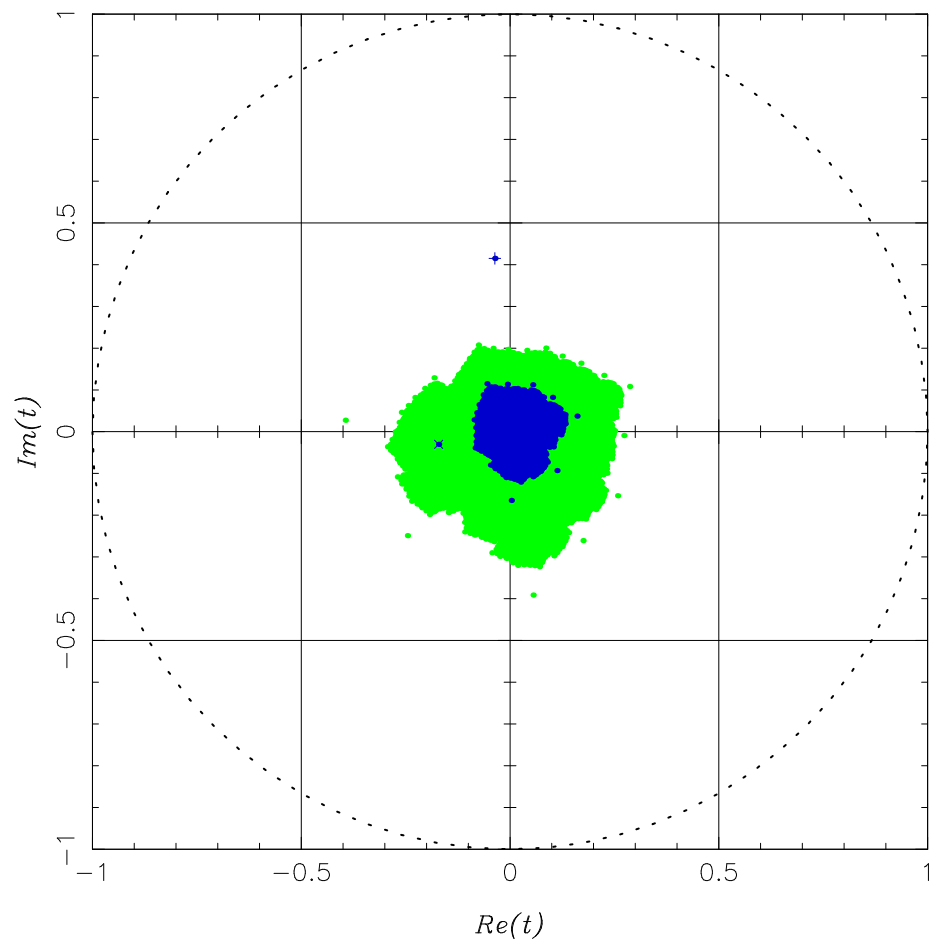

*Plot for  $q = 1.000 + 2.400\ i$  ( $R = 2.400$ ,  $k = 090$ )*

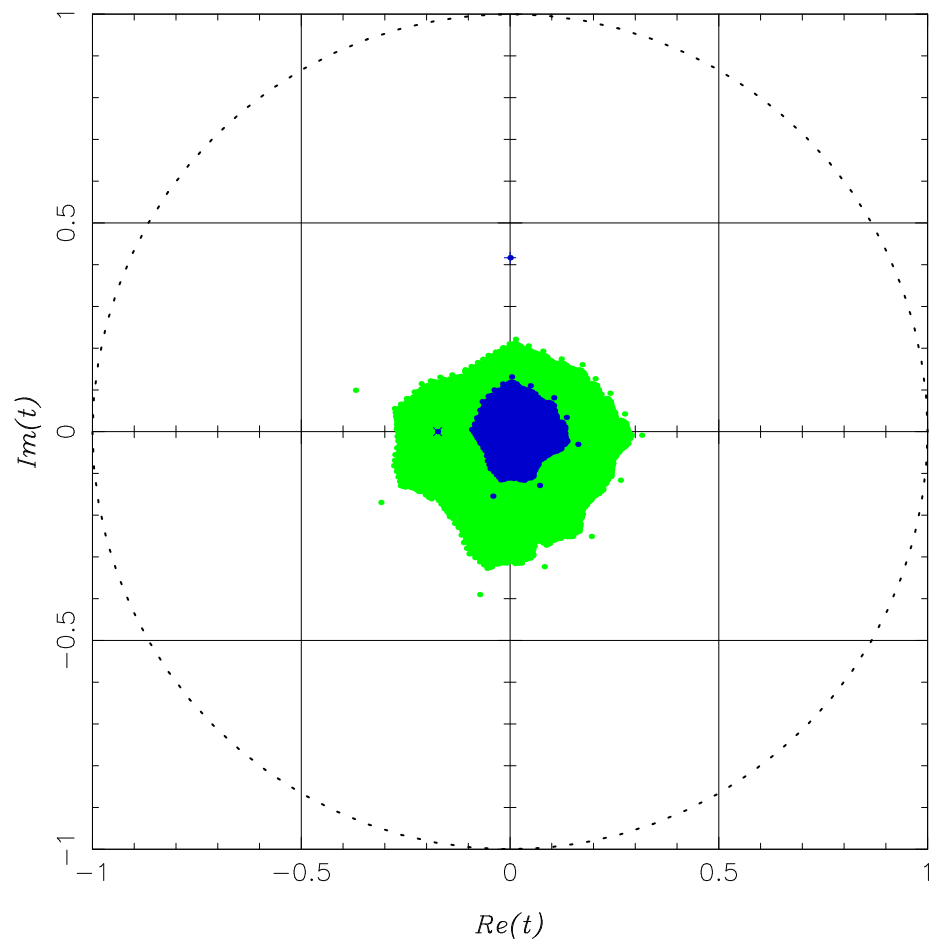

*Plot for  $q = 0.791 + 2.391 i$  ( $R = 2.400$ ,  $k = 095$ )*

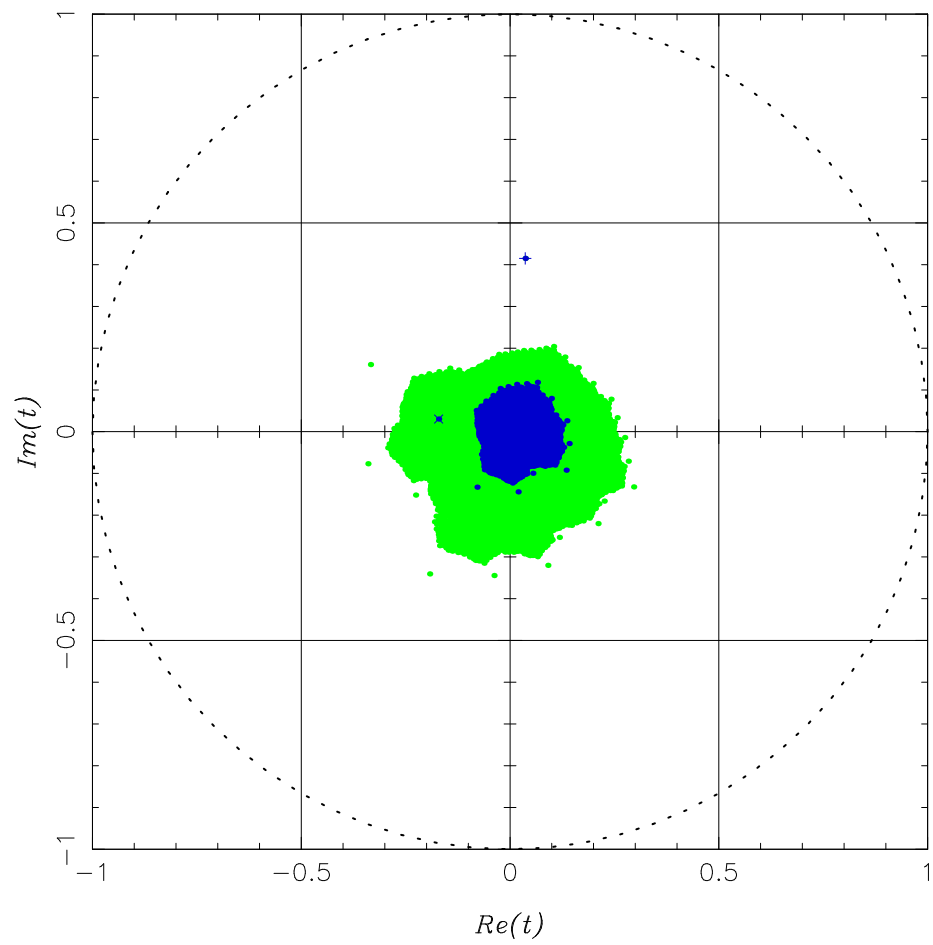

*Plot for  $q = 0.583 + 2.364 i$  ( $R = 2.400$ ,  $k = 100$ )*

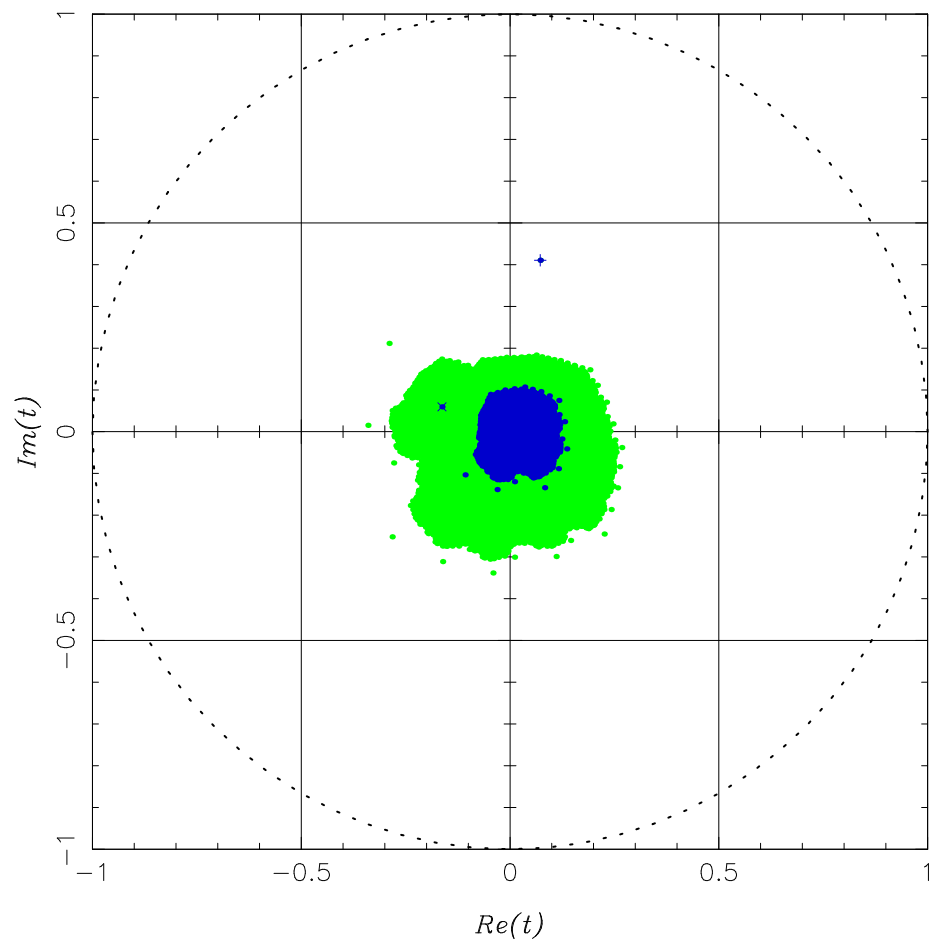

*Plot for  $q = 0.379 + 2.318 i$  ( $R = 2.400$ ,  $k = 105$ )*

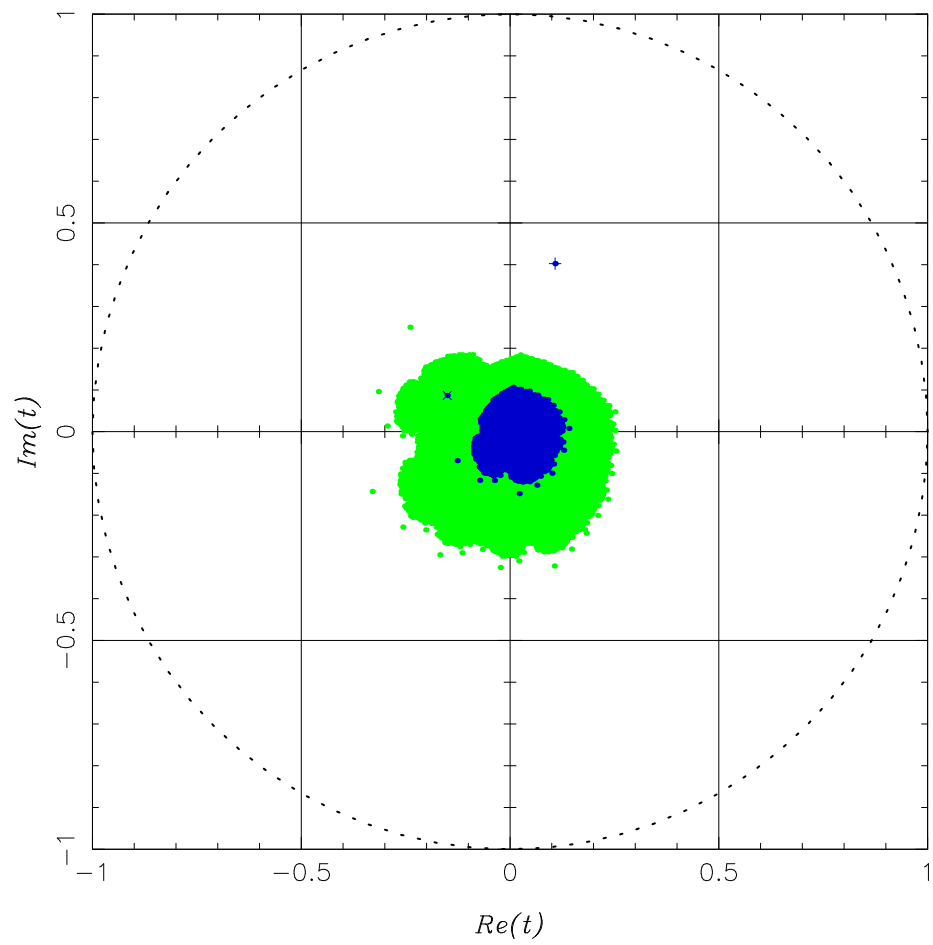

*Plot for  $q = 0.179 + 2.255 i$  ( $R = 2.400$ ,  $k = 110$ )*

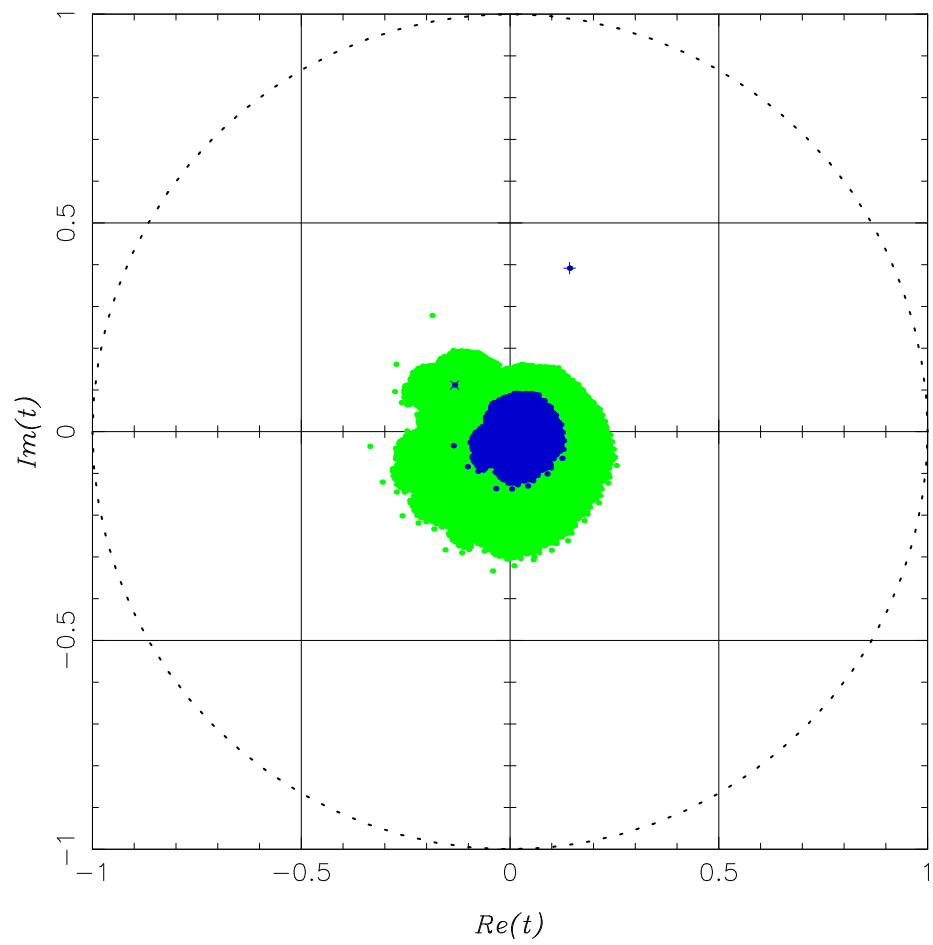



*Plot for  $q = -0.014 + 2.175 i$  ( $R = 2.400$ ,  $k = 115$ )*

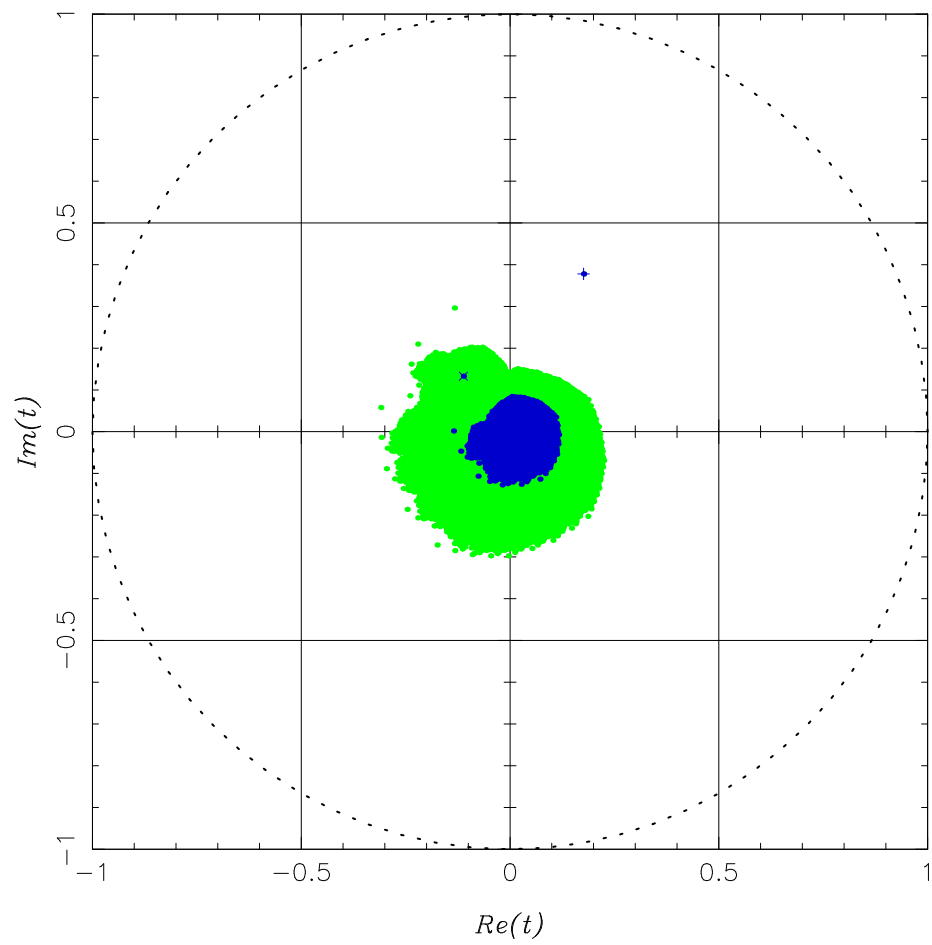

*Plot for  $q = -0.200 + 2.078 i$  ( $R = 2.400$ ,  $k = 120$ )*

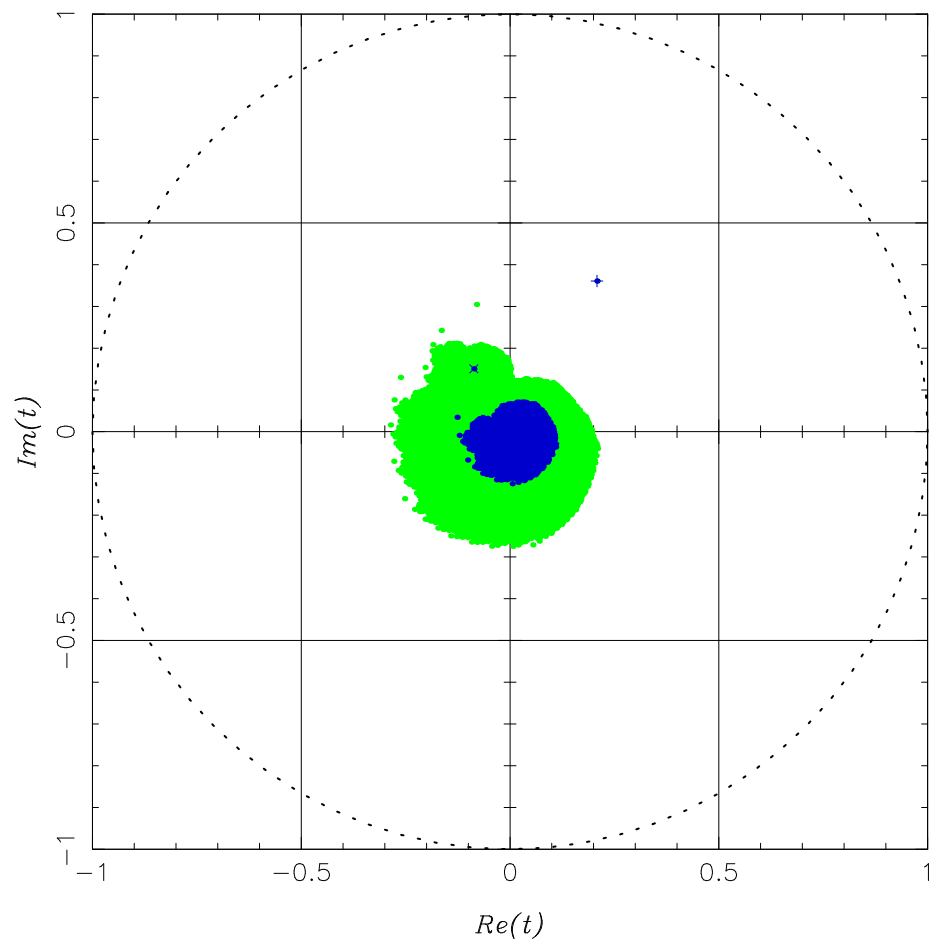

Plot for  $q = -0.377 + 1.966 i$  ( $R = 2.400$ ,  $k = 125$ )

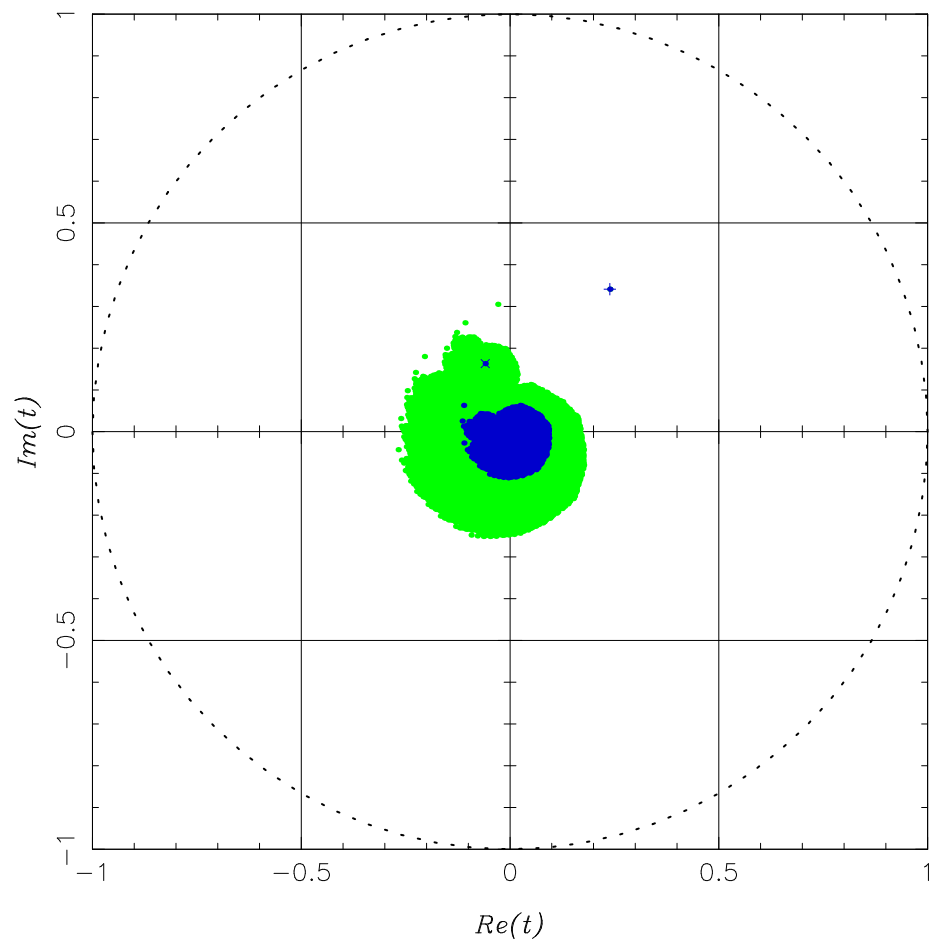

Plot for  $q = -0.543 + 1.839 i$  ( $R = 2.400$ ,  $k = 130$ )

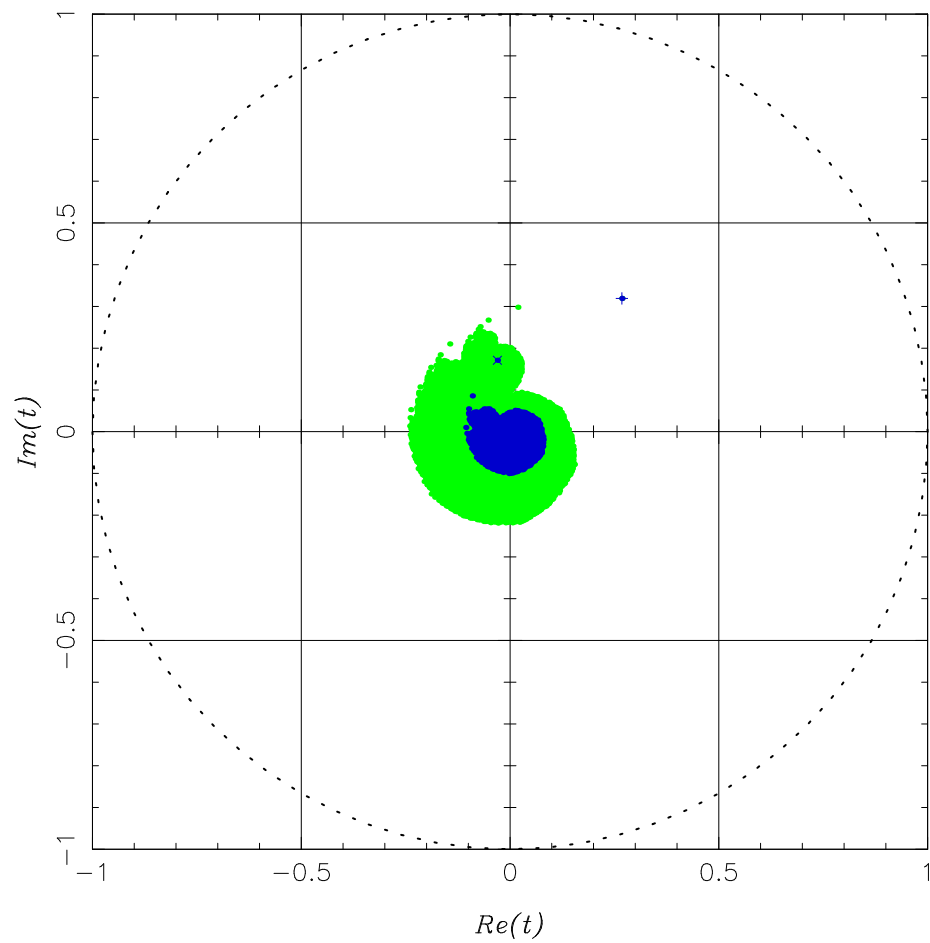

Plot for  $q = -0.697 + 1.697 i$  ( $R = 2.400$ ,  $k = 135$ )

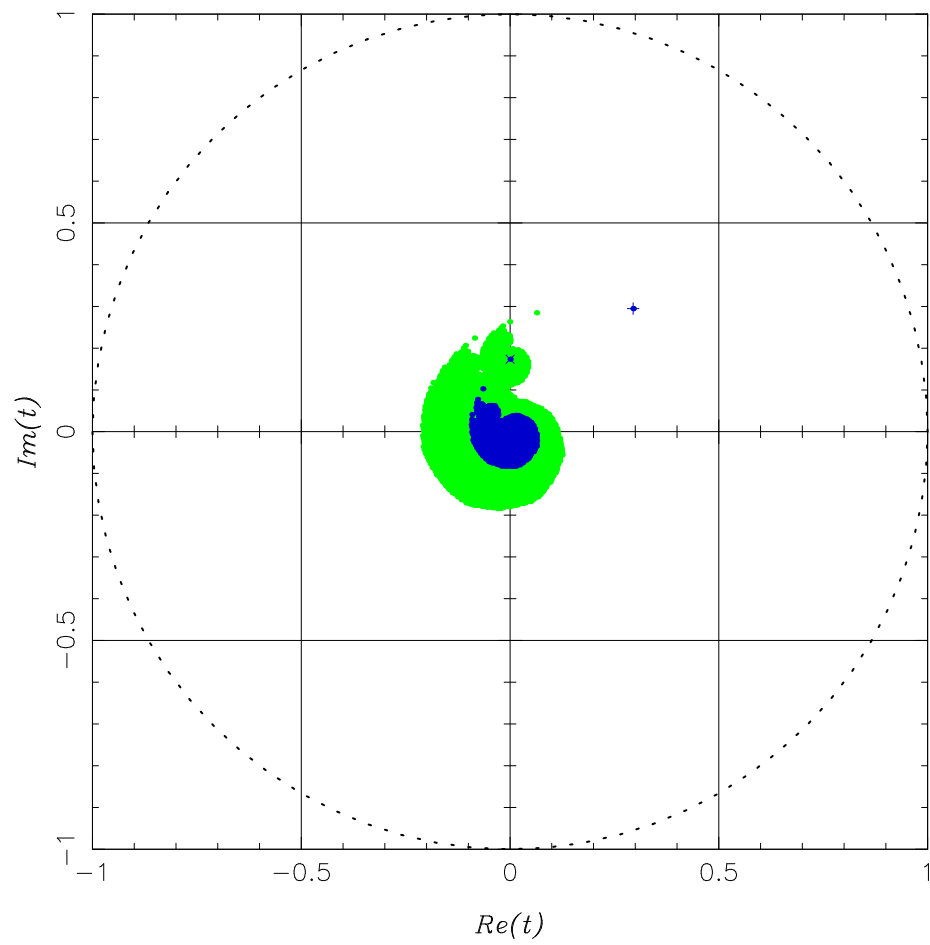

Plot for  $q = -0.839 + 1.543 i$  ( $R = 2.400$ ,  $k = 140$ )

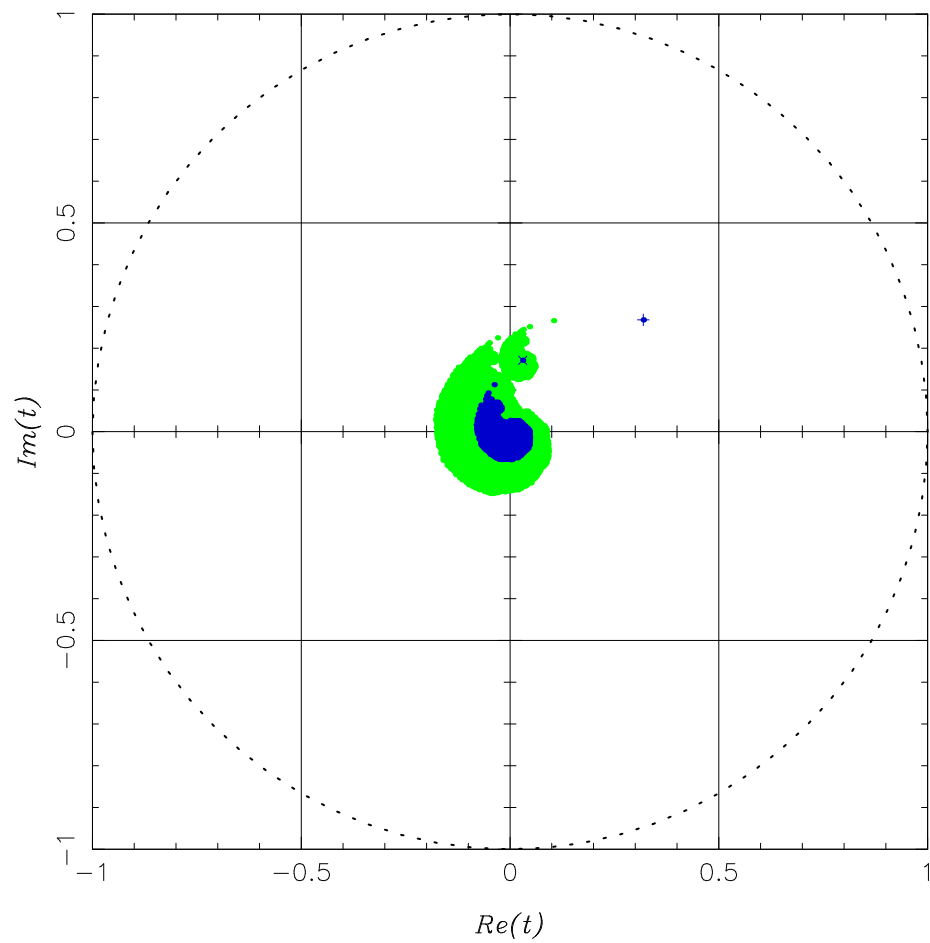

Plot for  $q = -0.966 + 1.377 i$  ( $R = 2.400$ ,  $k = 145$ )

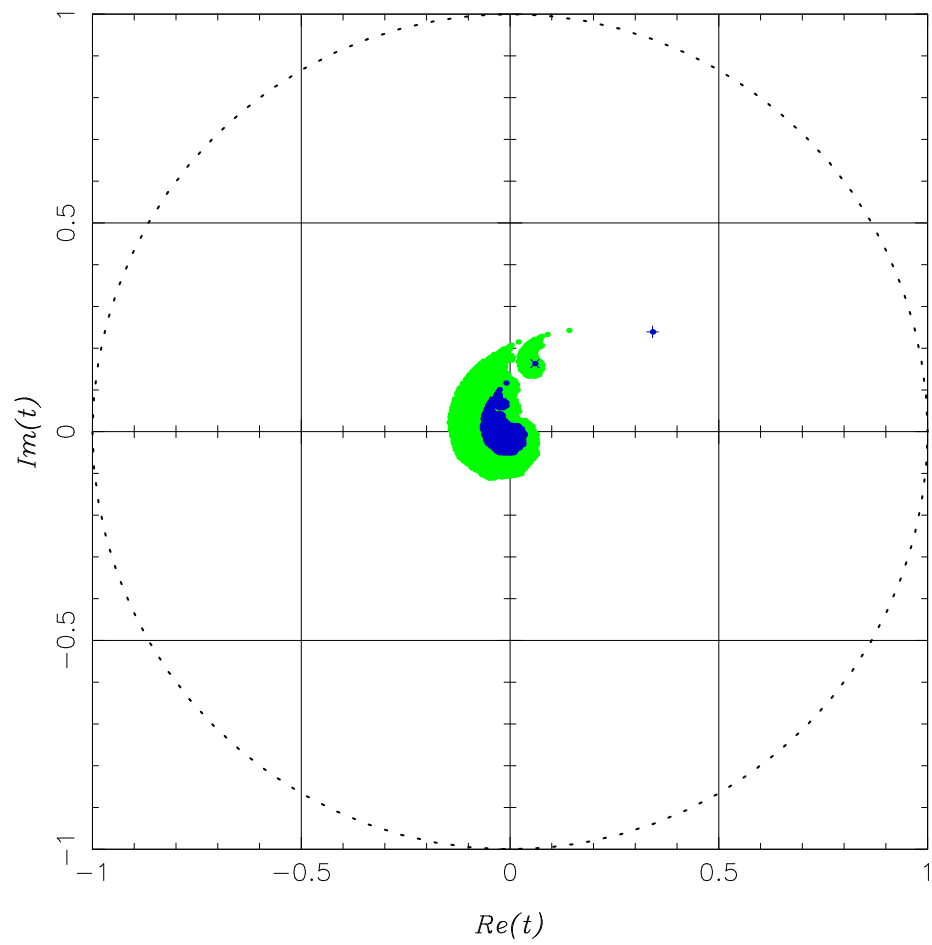

Plot for  $q = -1.078 + 1.200 i$  ( $R = 2.400$ ,  $k = 150$ )

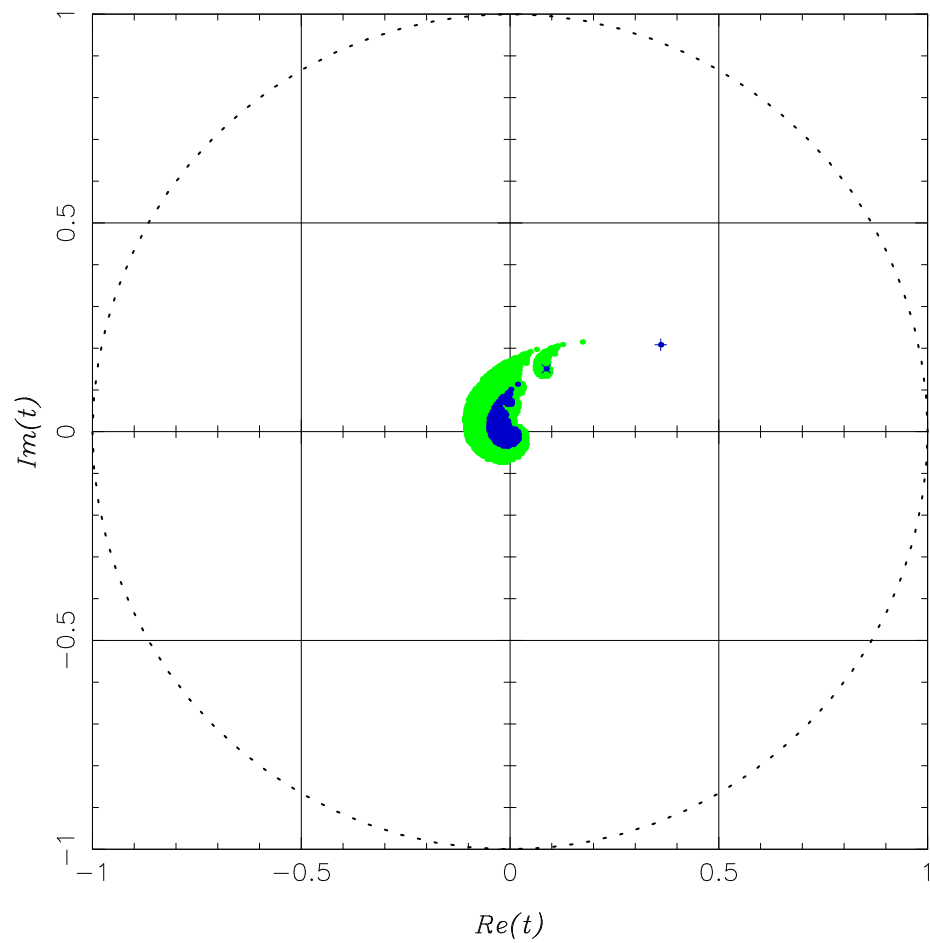



Plot for  $q = -1.175 + 1.014 i$  ( $R = 2.400$ ,  $k = 155$ )

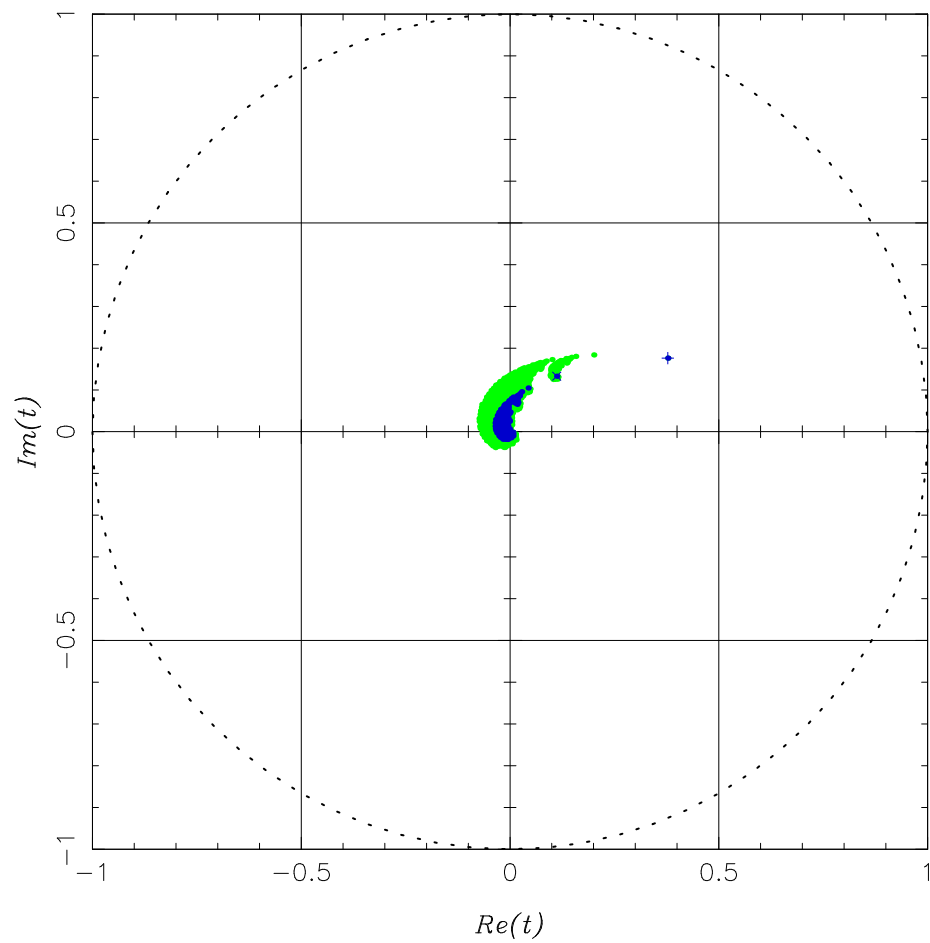

Plot for  $q = -1.255 + 0.821 i$  ( $R = 2.400$ ,  $k = 160$ )

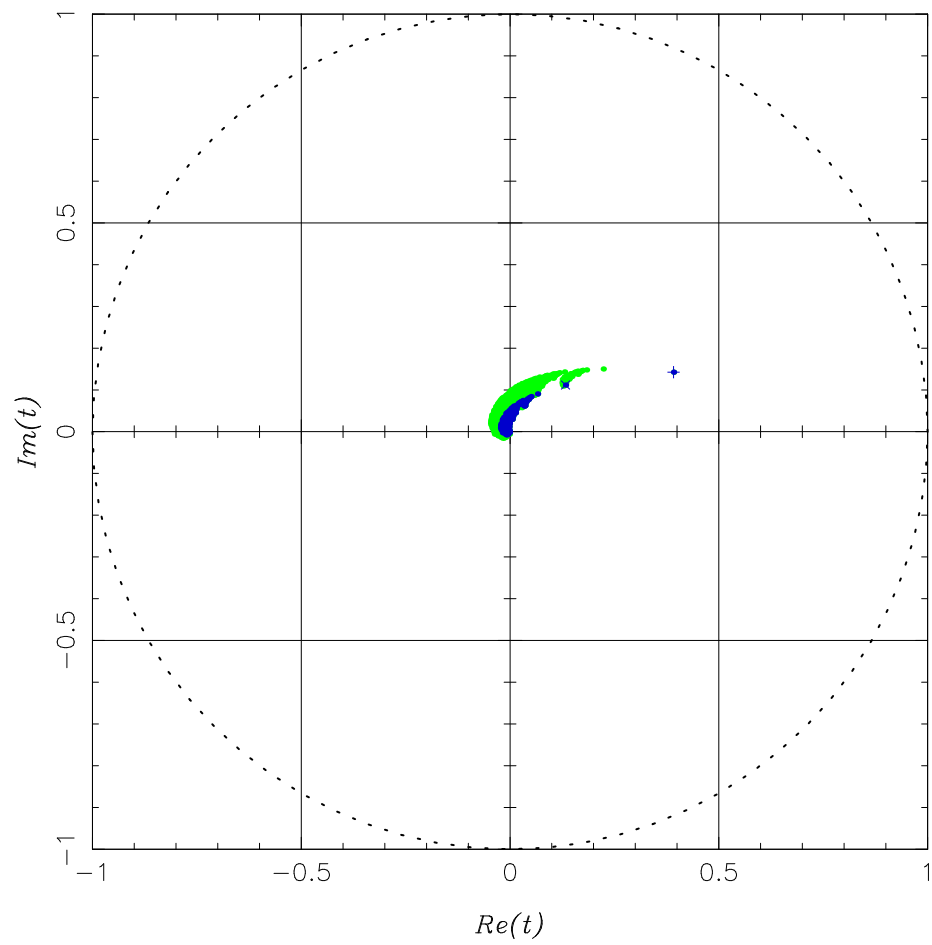

Plot for  $q = -1.318 + 0.621 i$  ( $R = 2.400$ ,  $k = 165$ )

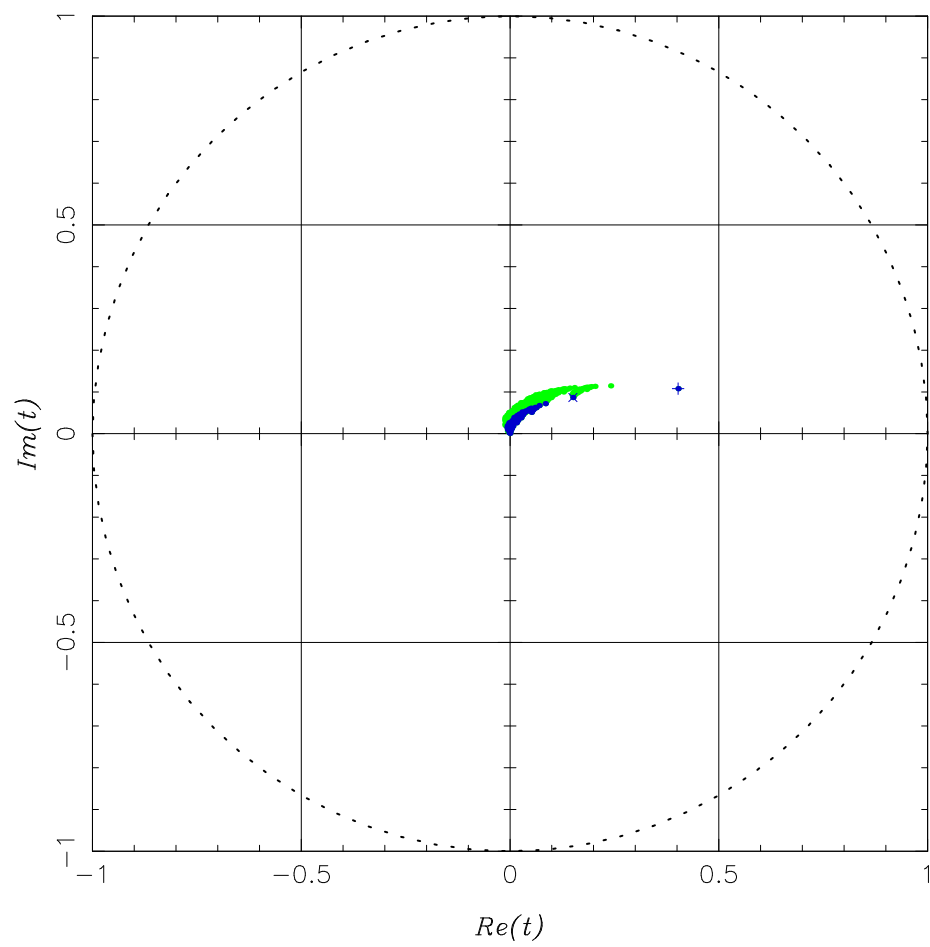

Plot for  $q = -1.364 + 0.417 i$  ( $R = 2.400$ ,  $k = 170$ )

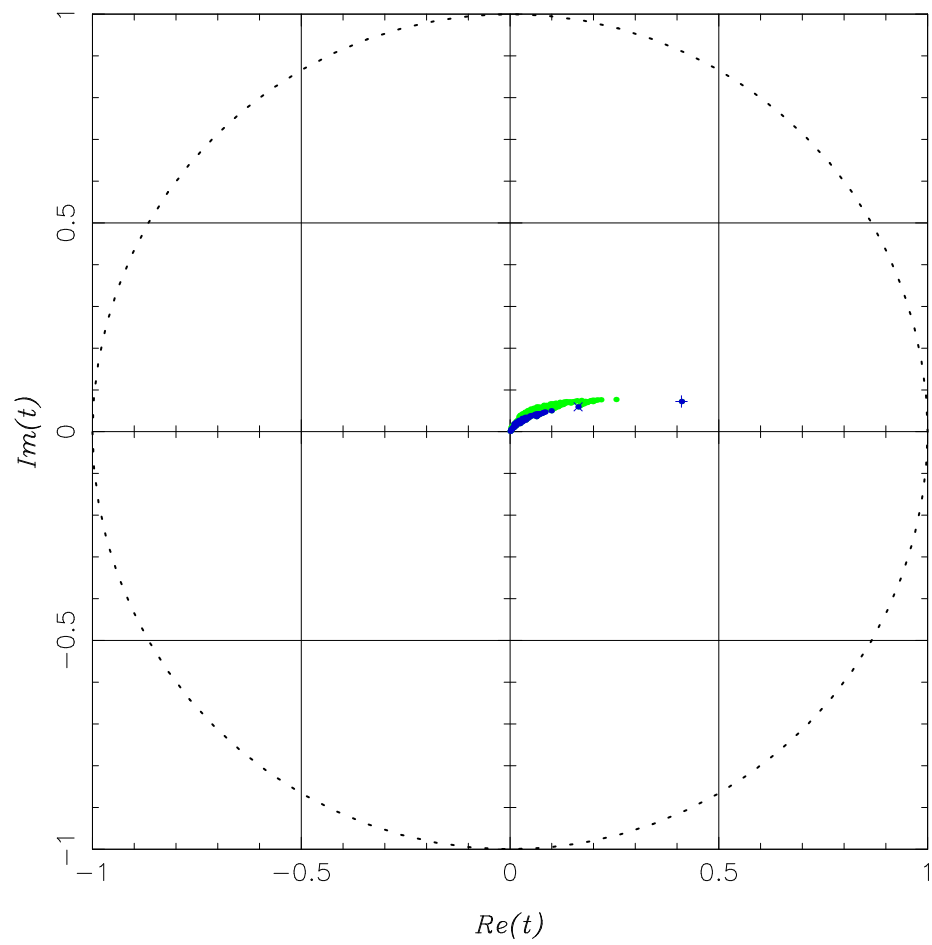

Plot for  $q = -1.391 + 0.209 i$  ( $R = 2.400$ ,  $k = 175$ )

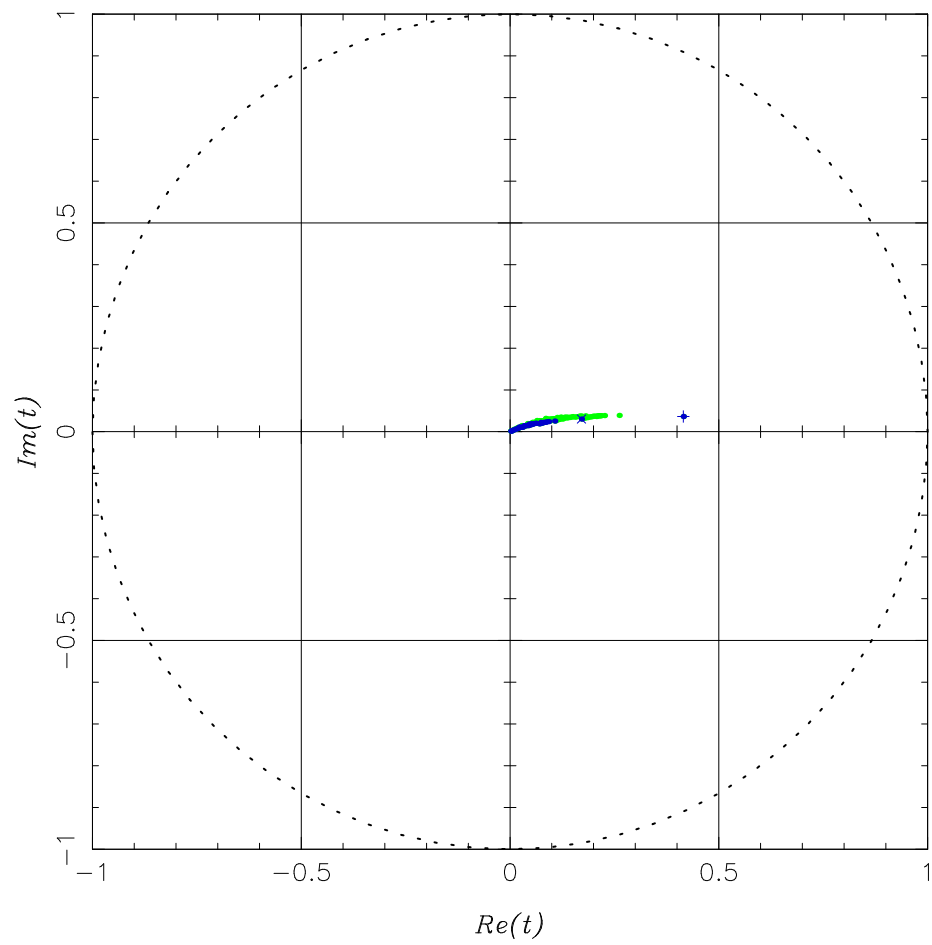

Plot for  $q = -1.400 + 0.000\ i$  ( $R = 2.400$ ,  $k = 180$ )

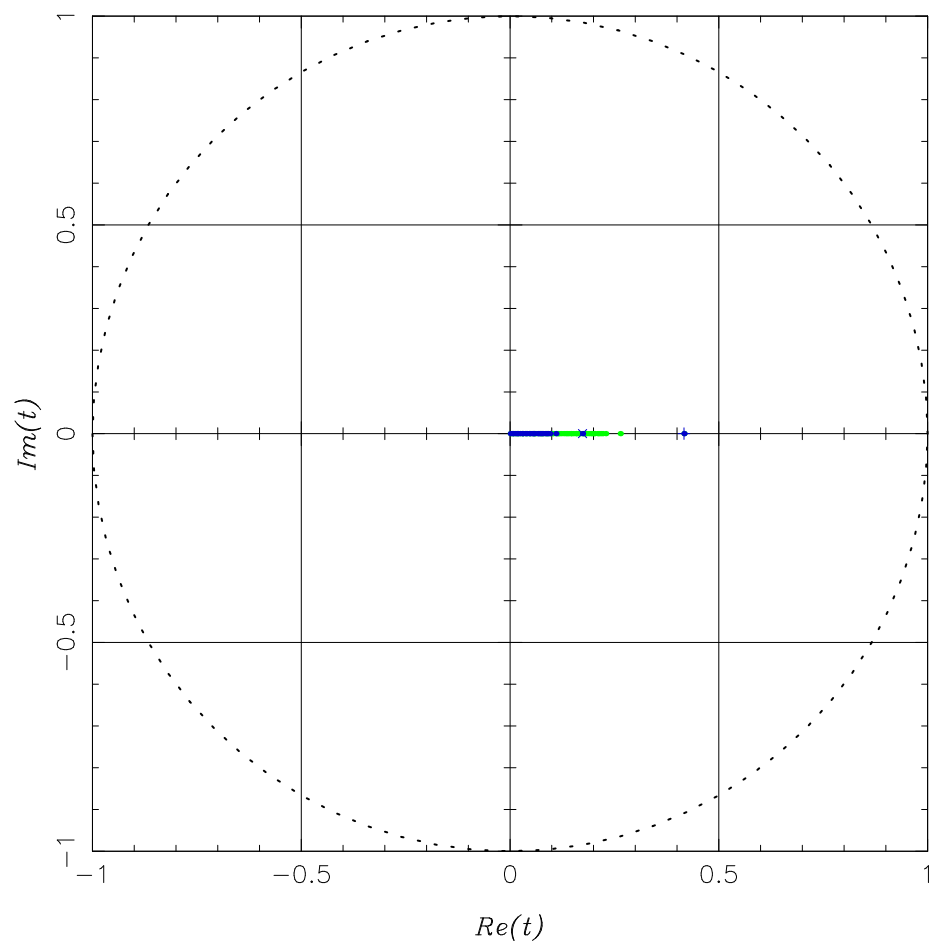

Supplement: Supplementary file 2 [file S1S2_2.4.pdf]
