# Supplementary material for: Linear bound in terms of maxmaxflow for the chromatic roots of series-parallel graphs
Source: arXiv:1307.1721 ancillary file (2013-07-05)

## Approximate shapes of $S_1$ and $S_2$ for $R = 3.0$

This document contains supporting plots for the paper “*Linear bound in terms of maxmaxflow for the chromatic roots of series-parallel graphs*” by Gordon Royle and Alan Sokal.

Each of the following pages contains a single plot showing the approximations for the sets  $S_1$  and  $S_2$  for a particular value of  $q$ . The chosen values of  $q$  all lie on the circle  $|q - 1| = 3.0$  and are spaced equally around the circle in increments of 5 degree. Thus for  $k = 0, 5, 10, \dots, 180$ , there are plots for each  $q$  of the form  $q = 1 + 3.0e^{2\pi i(k/360)}$ .

Each plot shows in light-green the approximation for  $S_2$  and in dark-blue the approximation for  $S_1$ . The important points  $t_0 = 1/(1-q)$  and  $t_0^2$  are marked by a + and a  $\times$  respectively. If the true regions  $S_1$  and  $S_2$  are contained completely within the circle  $|t| = 1$  then this certifies that  $q$  is not a chromatic root for any series-parallel graph of maxmaxflow  $\Lambda = 3$ .

*Plot for  $q = 4.000 + 0.000\ i$  ( $R = 3.000$ ,  $k = 000$ )*

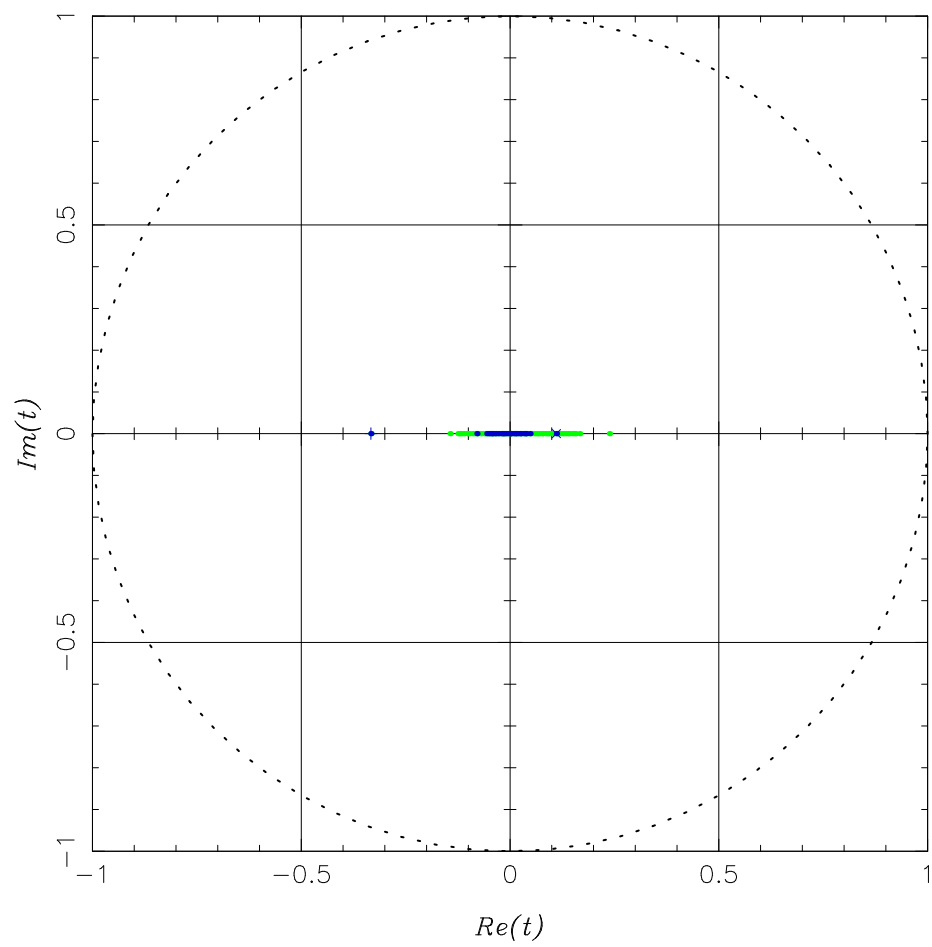

*Plot for  $q = 3.989 + 0.261 i$  ( $R = 3.000$ ,  $k = 005$ )*

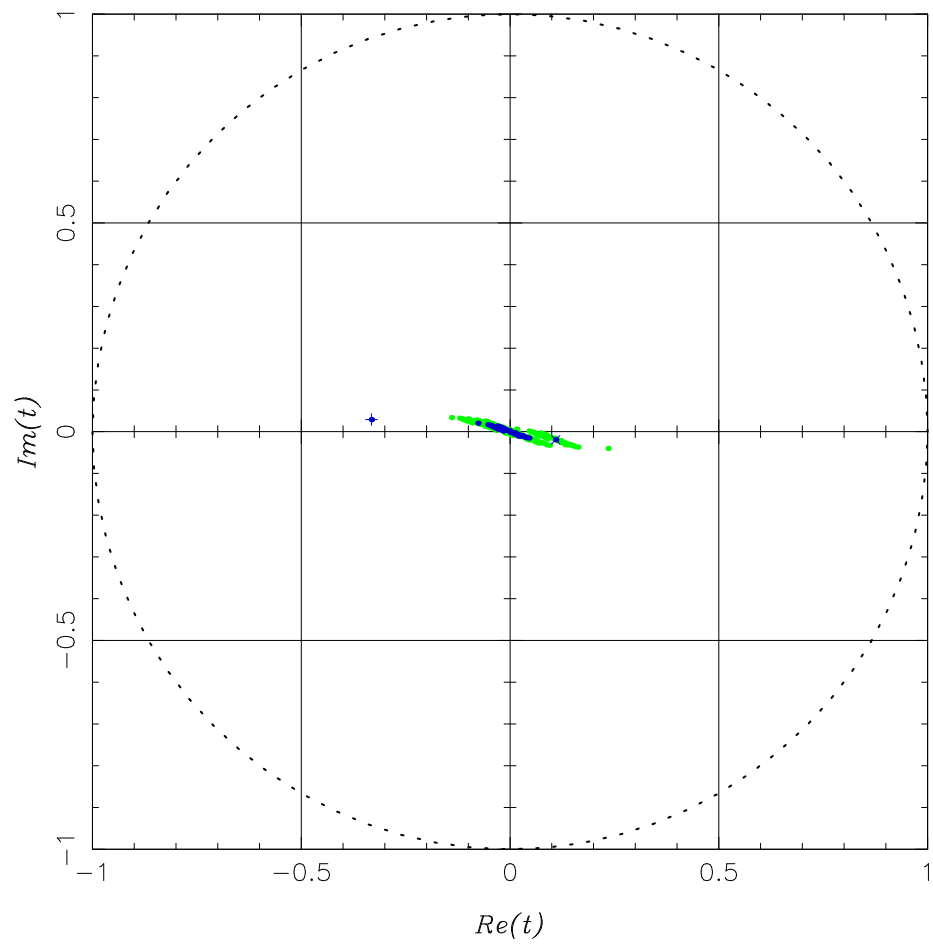

*Plot for  $q = 3.954 + 0.521 i$  ( $R = 3.000$ ,  $k = 010$ )*

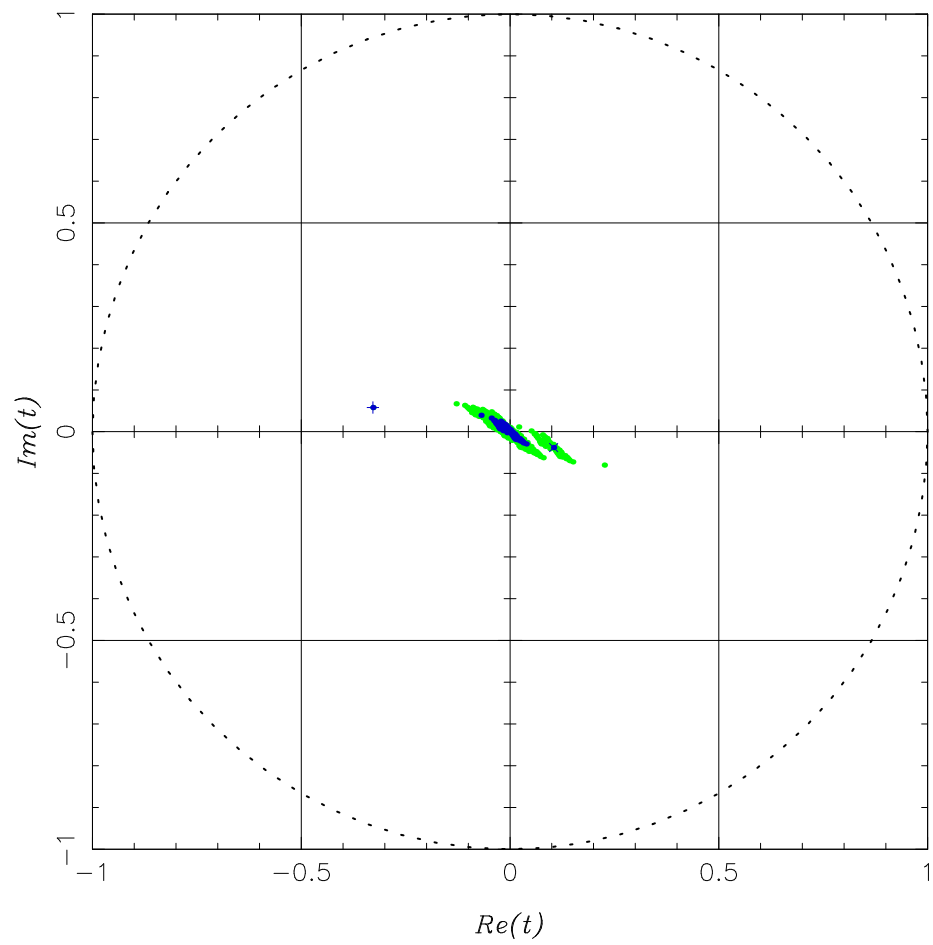

*Plot for  $q = 3.898 + 0.776 i$  ( $R = 3.000$ ,  $k = 015$ )*

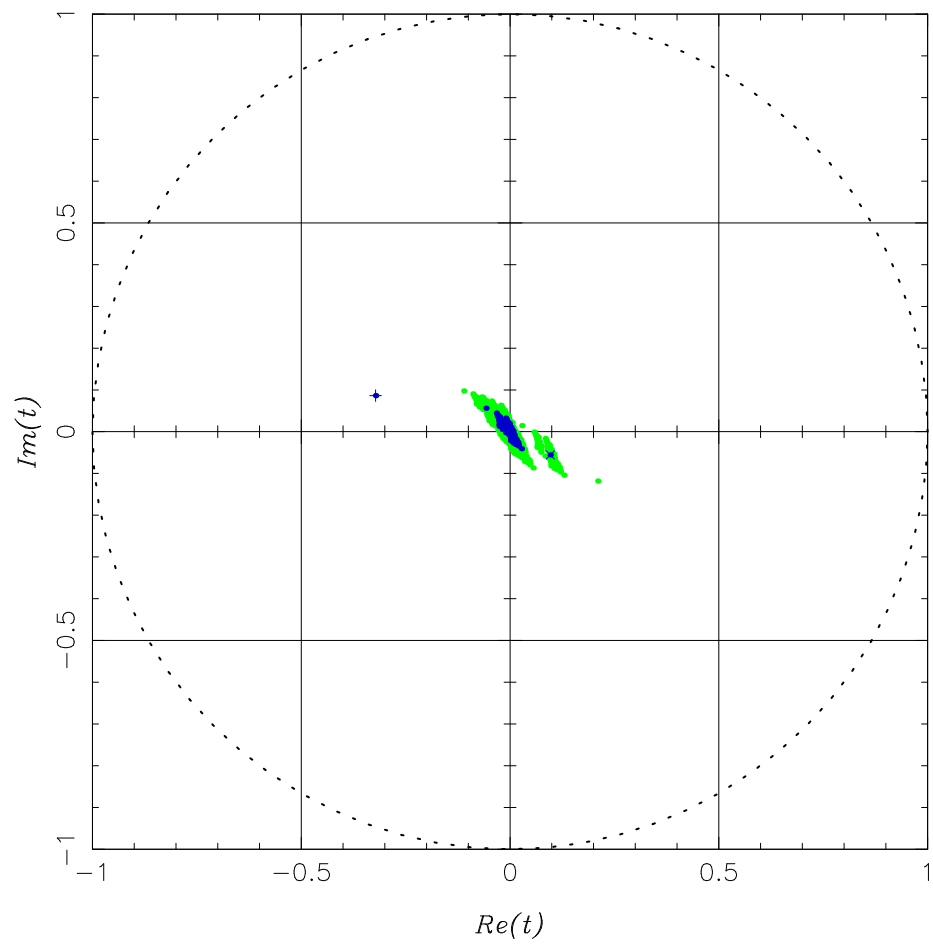

*Plot for  $q = 3.819 + 1.026 i$  ( $R = 3.000$ ,  $k = 020$ )*

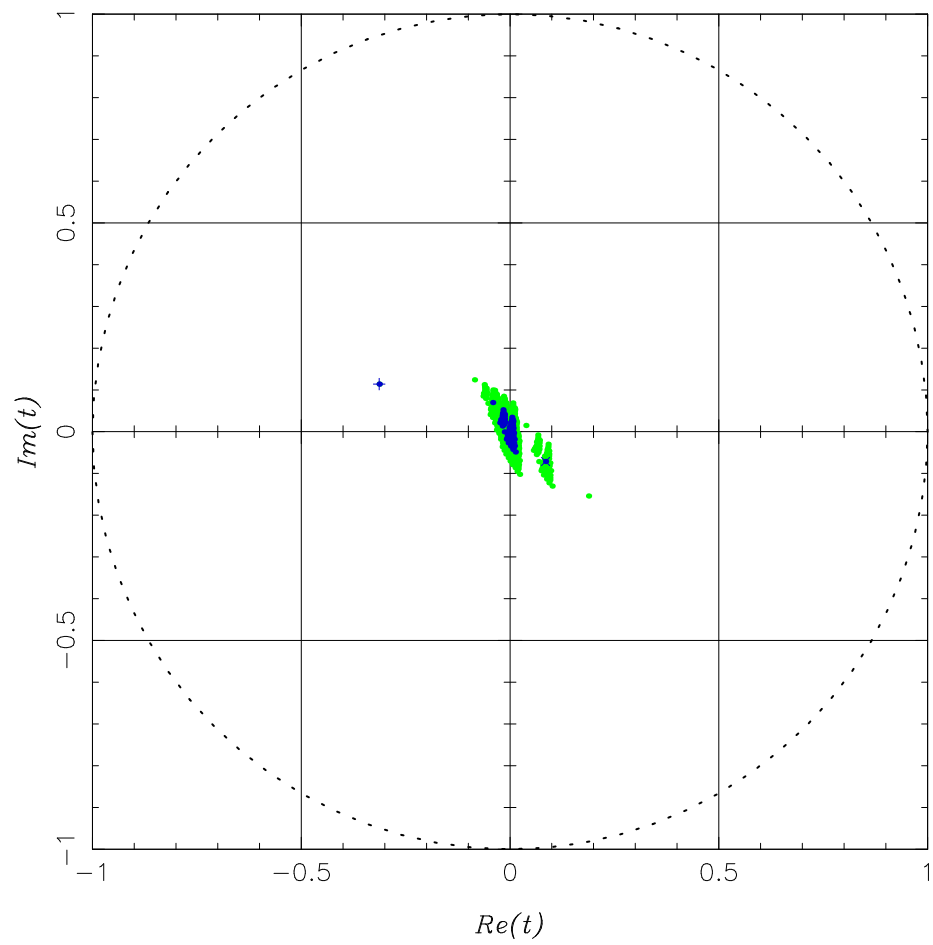

*Plot for  $q = 3.719 + 1.268 i$  ( $R = 3.000$ ,  $k = 025$ )*

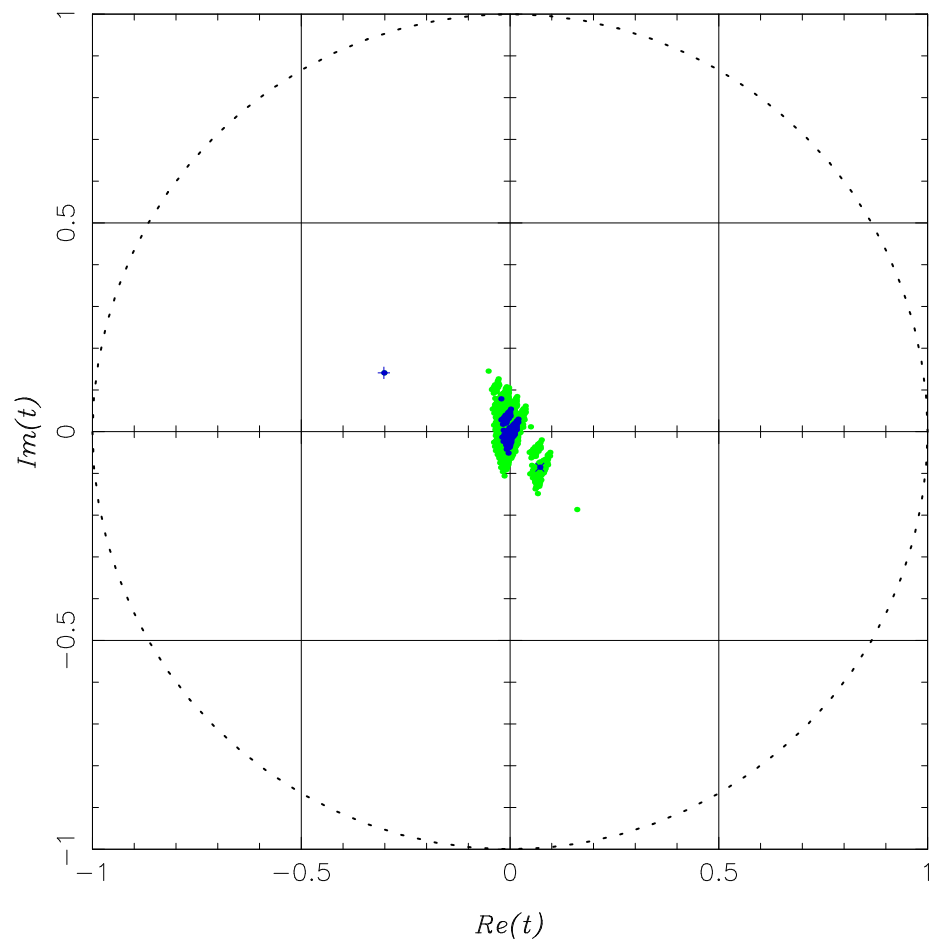

*Plot for  $q = 3.598 + 1.500\ i$  ( $R = 3.000$ ,  $k = 030$ )*

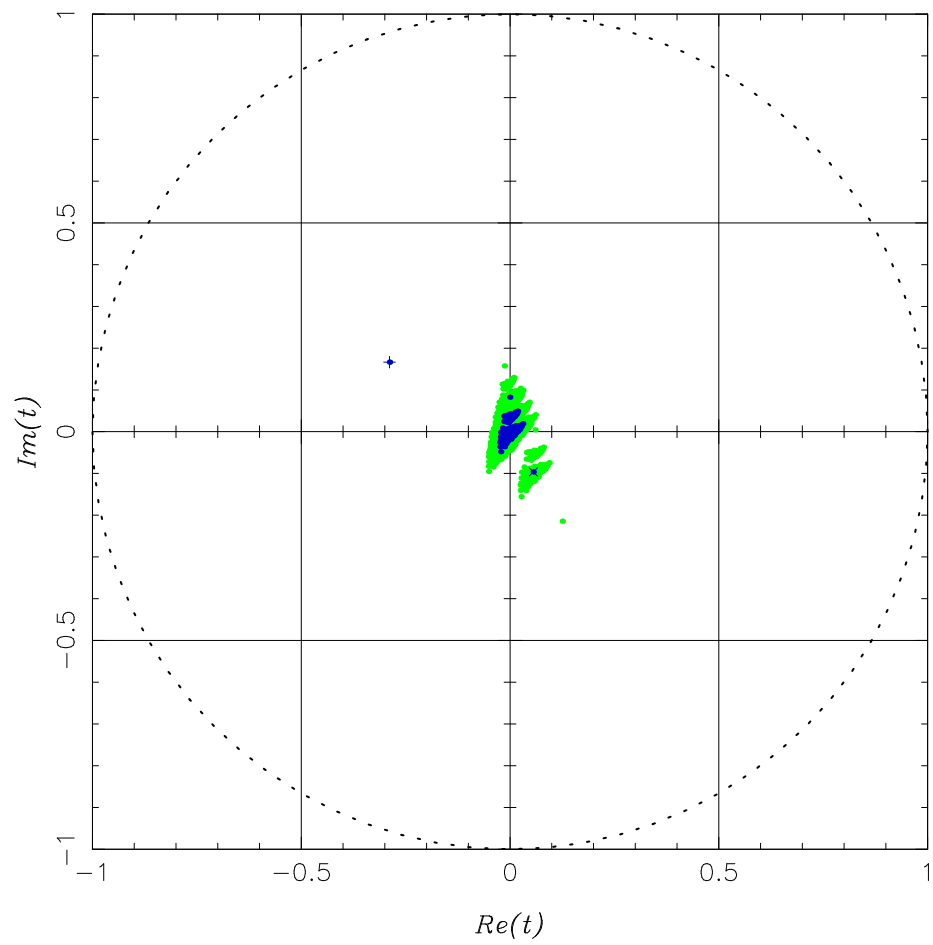



*Plot for  $q = 3.457 + 1.721 i$  ( $R = 3.000$ ,  $k = 035$ )*

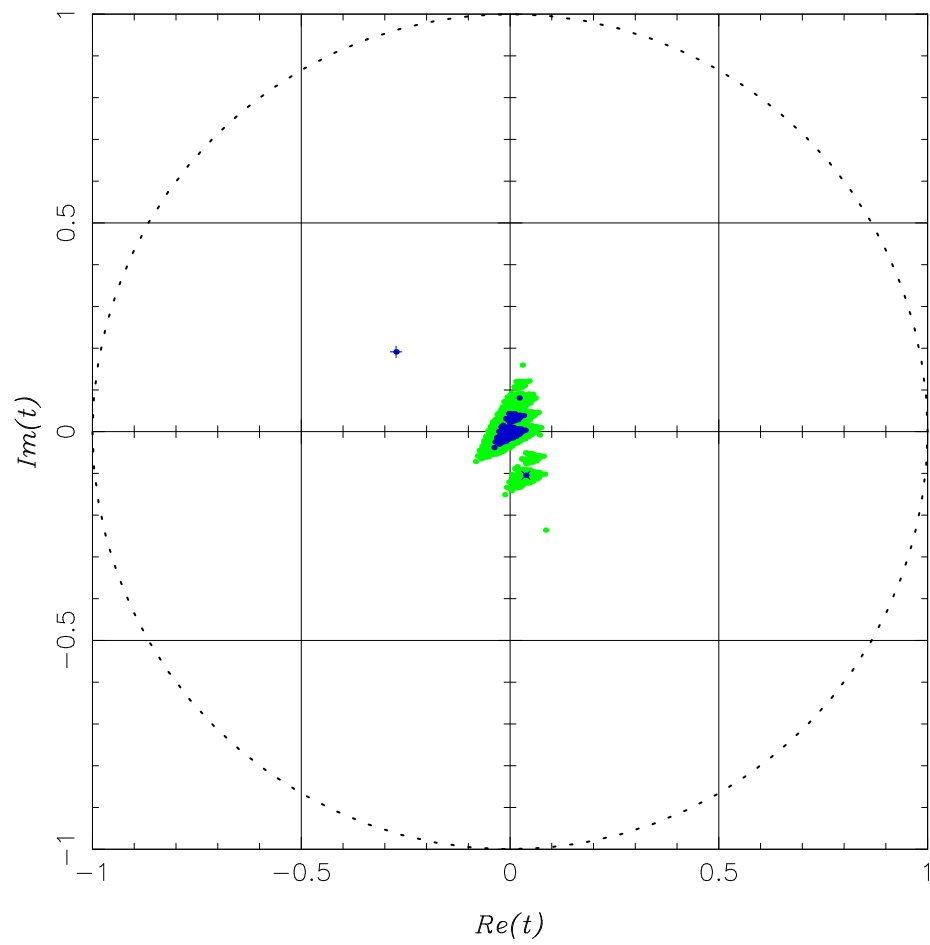

*Plot for  $q = 3.298 + 1.928 i$  ( $R = 3.000$ ,  $k = 040$ )*

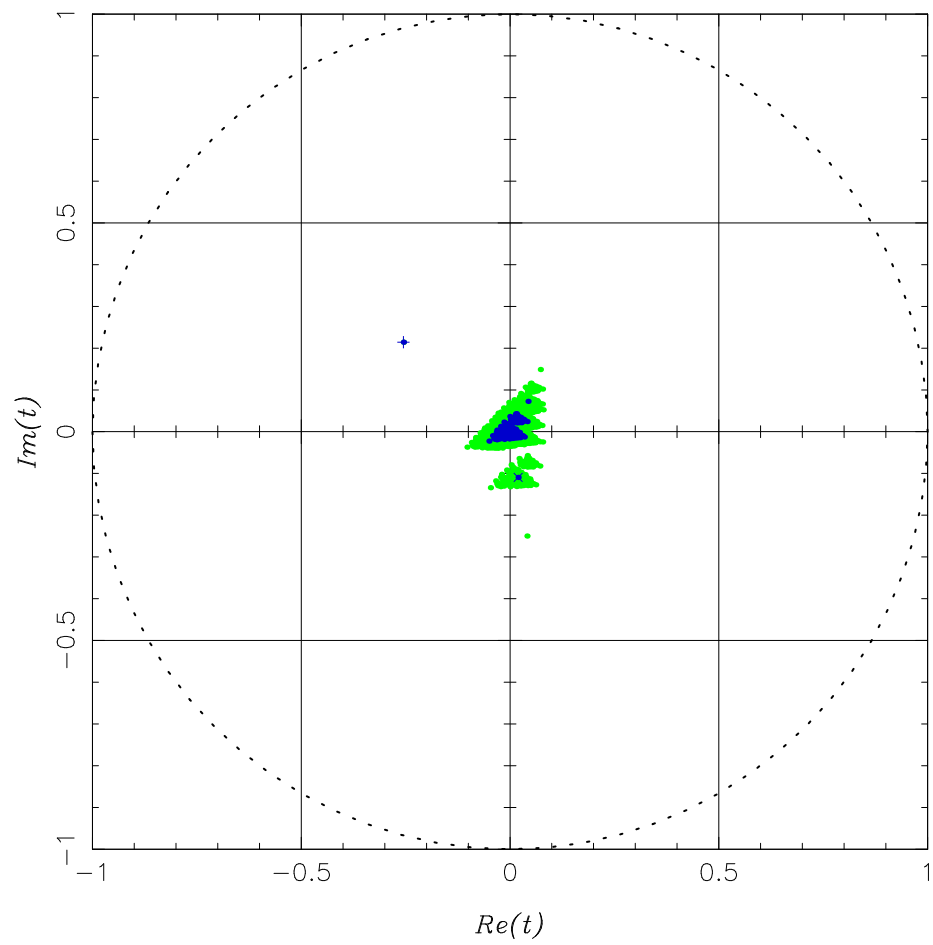

*Plot for  $q = 3.121 + 2.121 i$  ( $R = 3.000$ ,  $k = 045$ )*

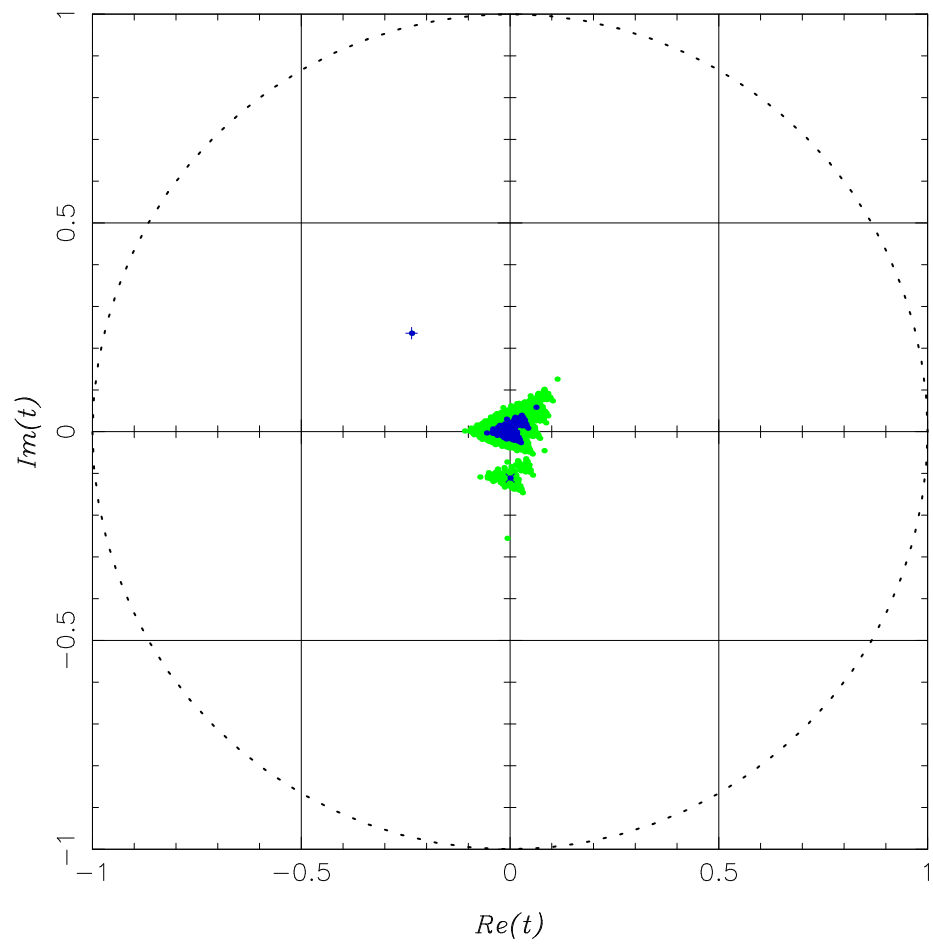

*Plot for  $q = 2.928 + 2.298 i$  ( $R = 3.000$ ,  $k = 050$ )*

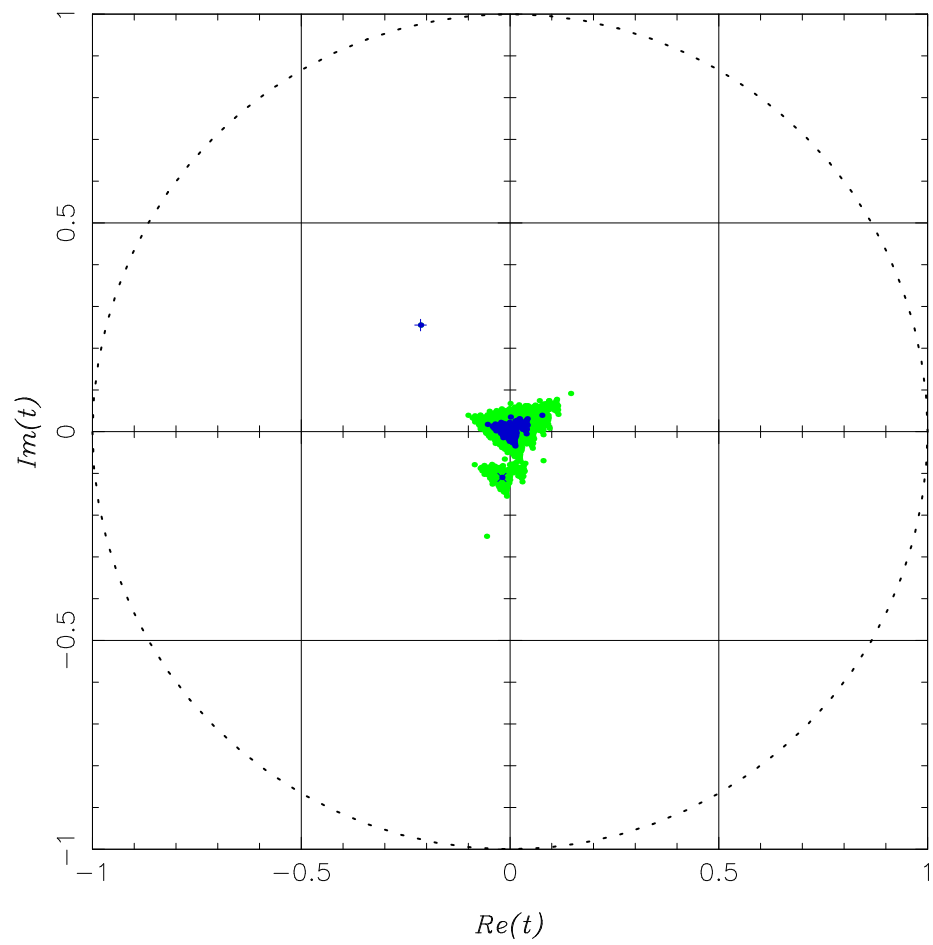

*Plot for  $q = 2.721 + 2.457 i$  ( $R = 3.000$ ,  $k = 055$ )*

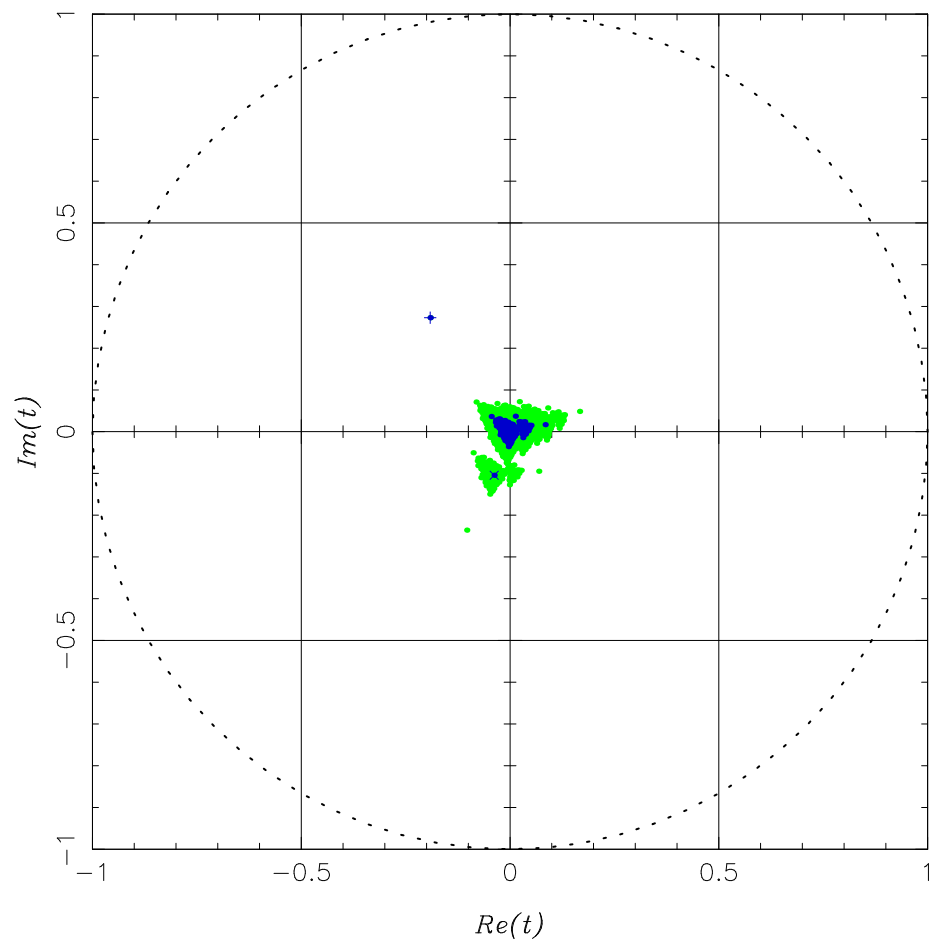

*Plot for  $q = 2.500 + 2.598 i$  ( $R = 3.000$ ,  $k = 060$ )*

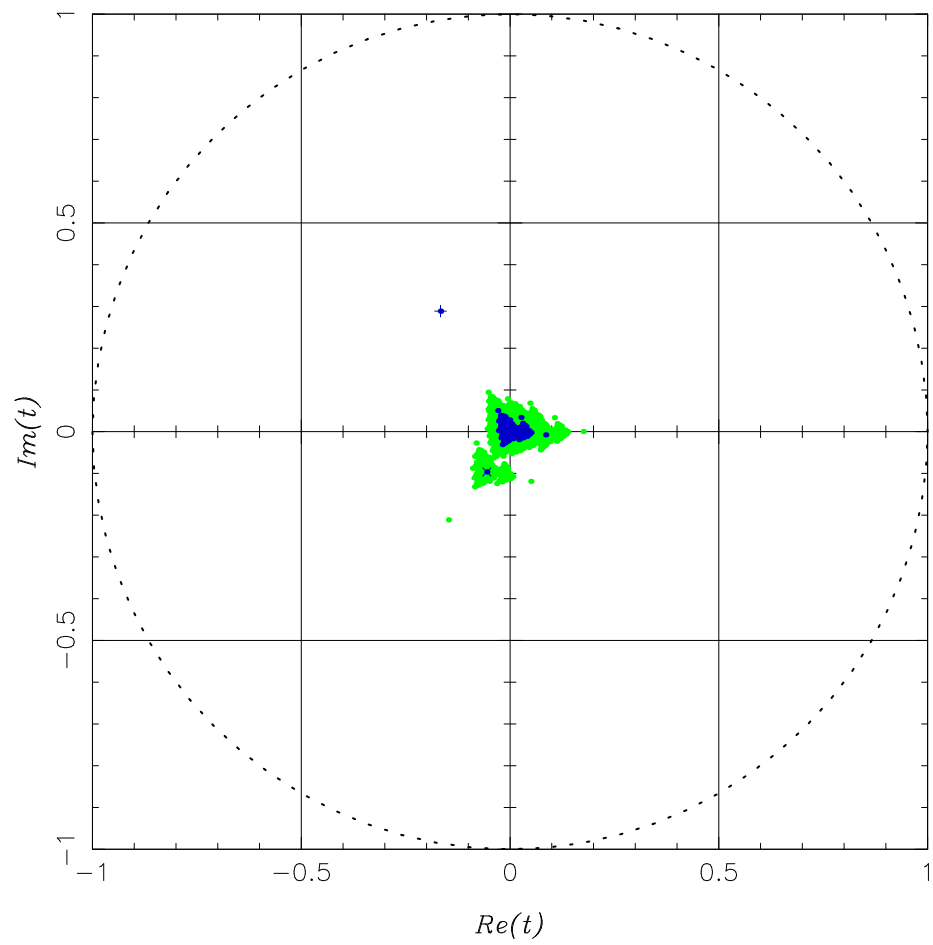

*Plot for  $q = 2.268 + 2.719 i$  ( $R = 3.000$ ,  $k = 065$ )*

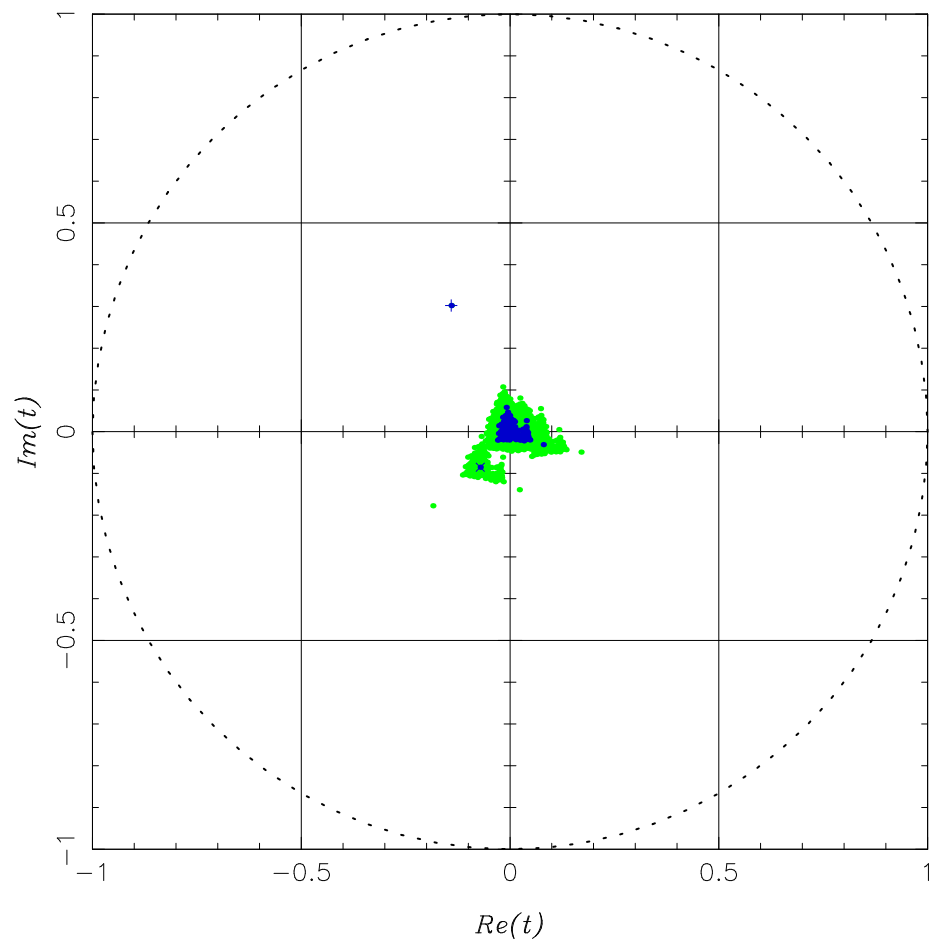

*Plot for  $q = 2.026 + 2.819 i$  ( $R = 3.000$ ,  $k = 070$ )*

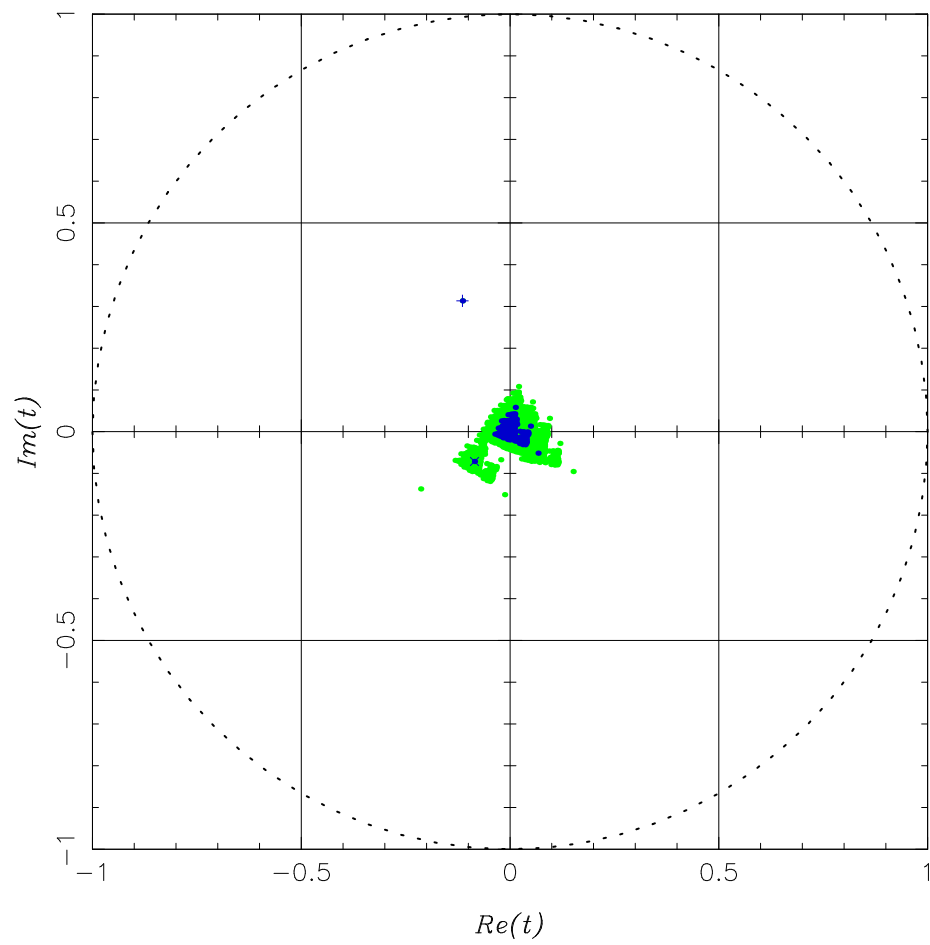



*Plot for  $q = 1.776 + 2.898 i$  ( $R = 3.000$ ,  $k = 075$ )*

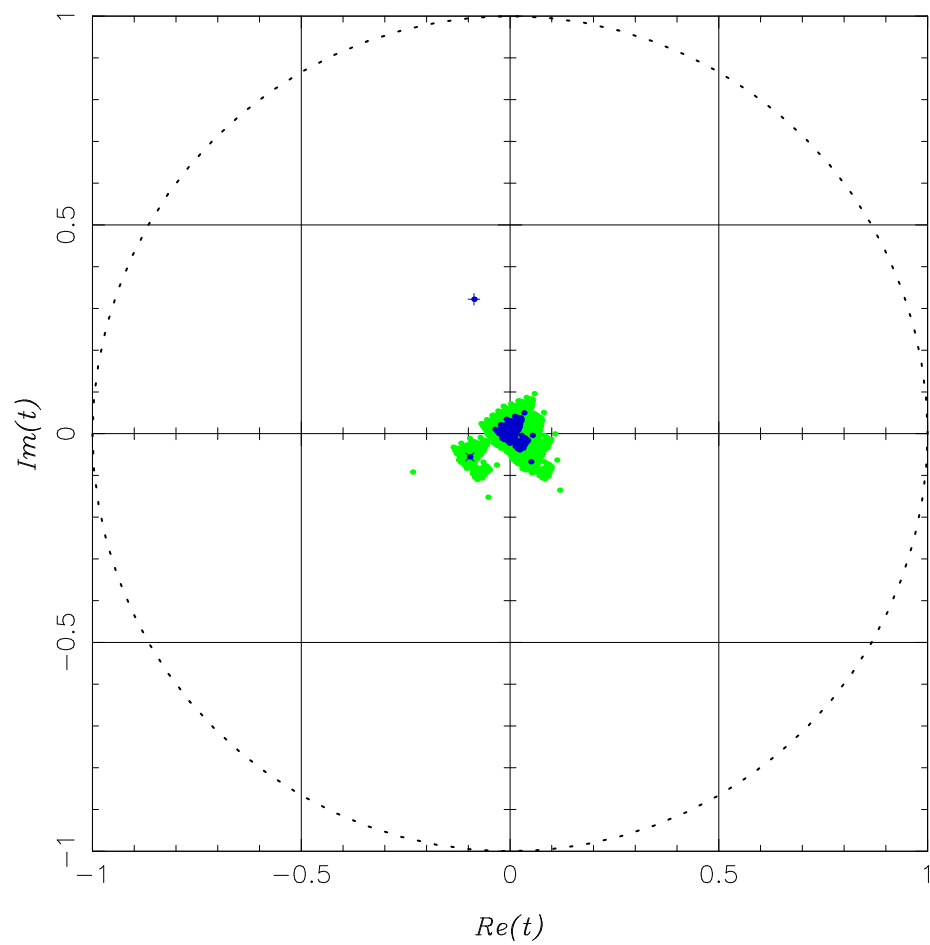

*Plot for  $q = 1.521 + 2.954 i$  ( $R = 3.000$ ,  $k = 080$ )*

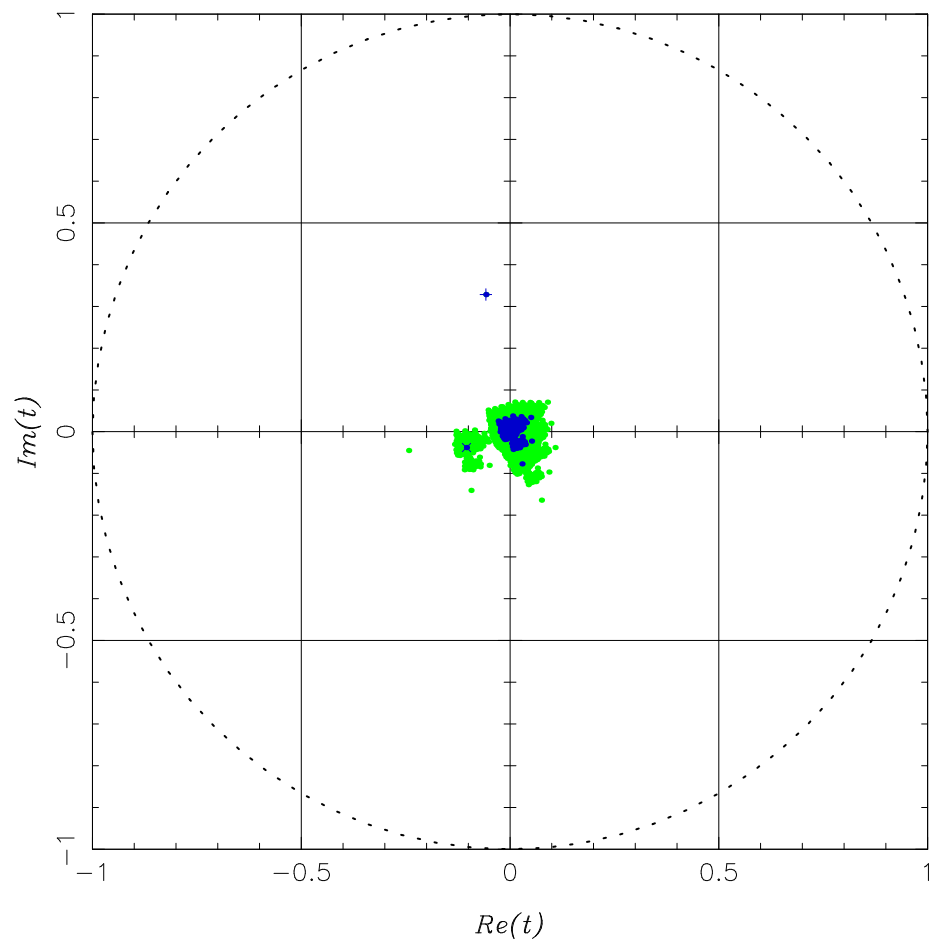

*Plot for  $q = 1.261 + 2.989 i$  ( $R = 3.000$ ,  $k = 085$ )*

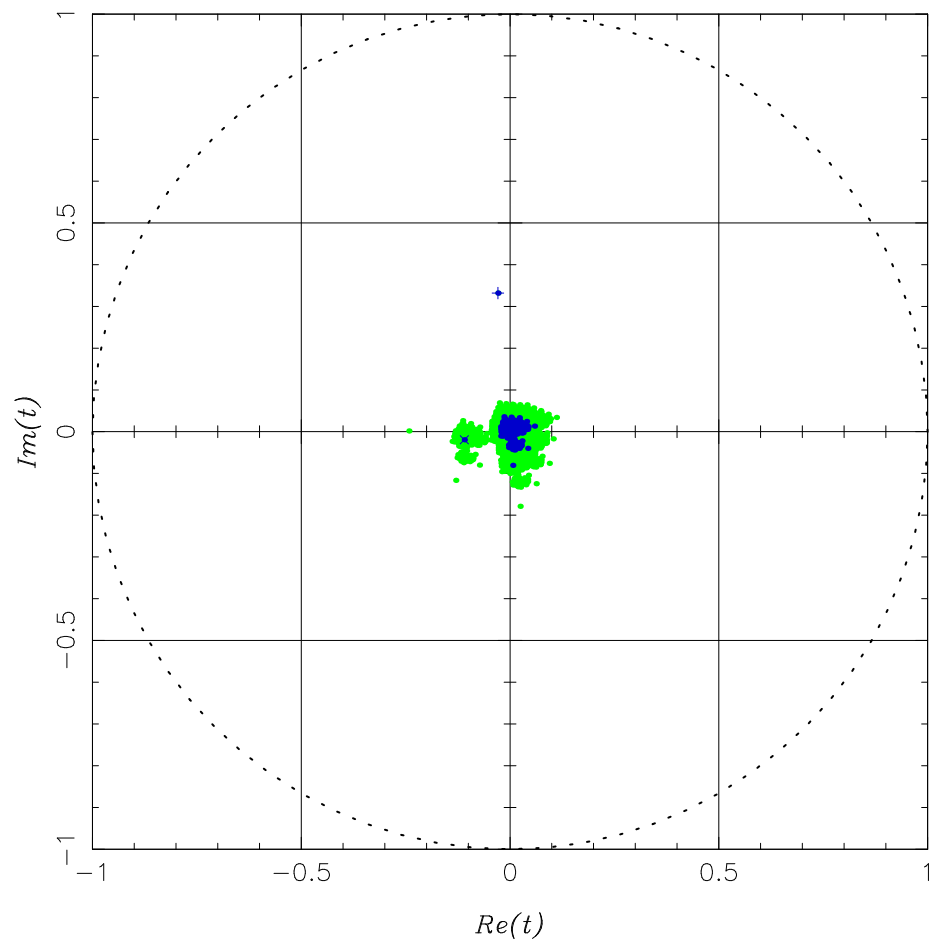

*Plot for  $q = 1.000 + 3.000\ i$  ( $R = 3.000$ ,  $k = 090$ )*

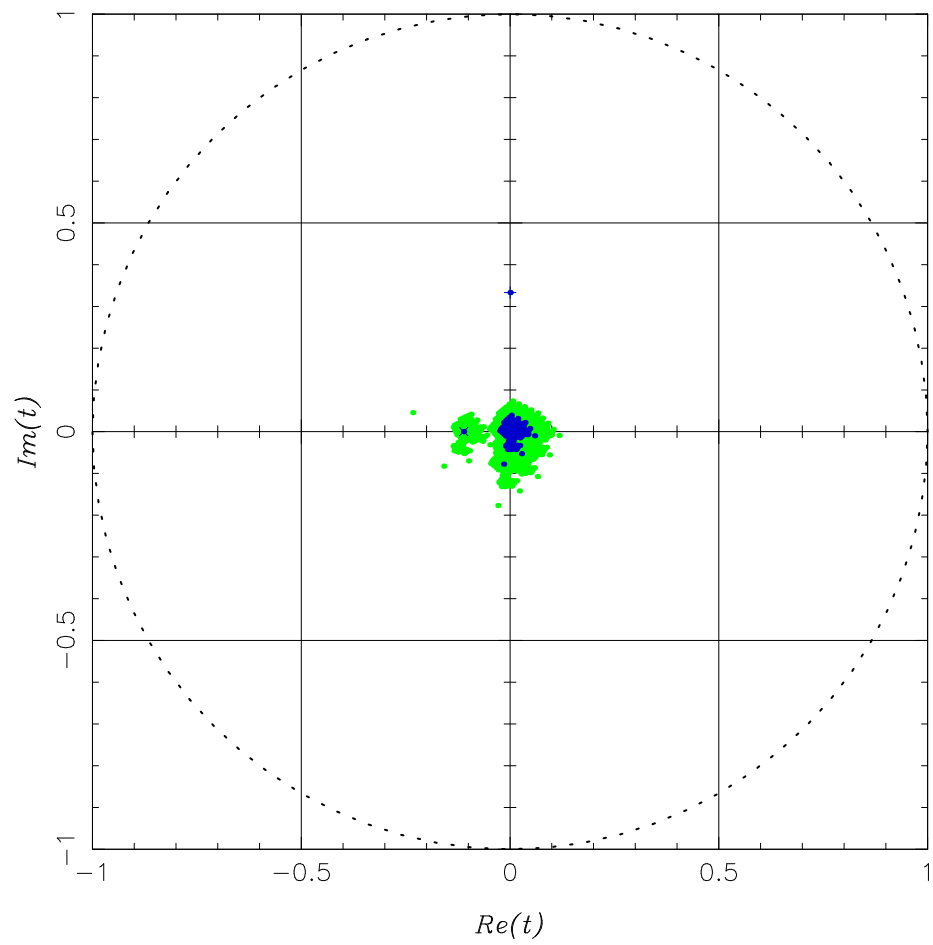

*Plot for  $q = 0.739 + 2.989 i$  ( $R = 3.000$ ,  $k = 095$ )*

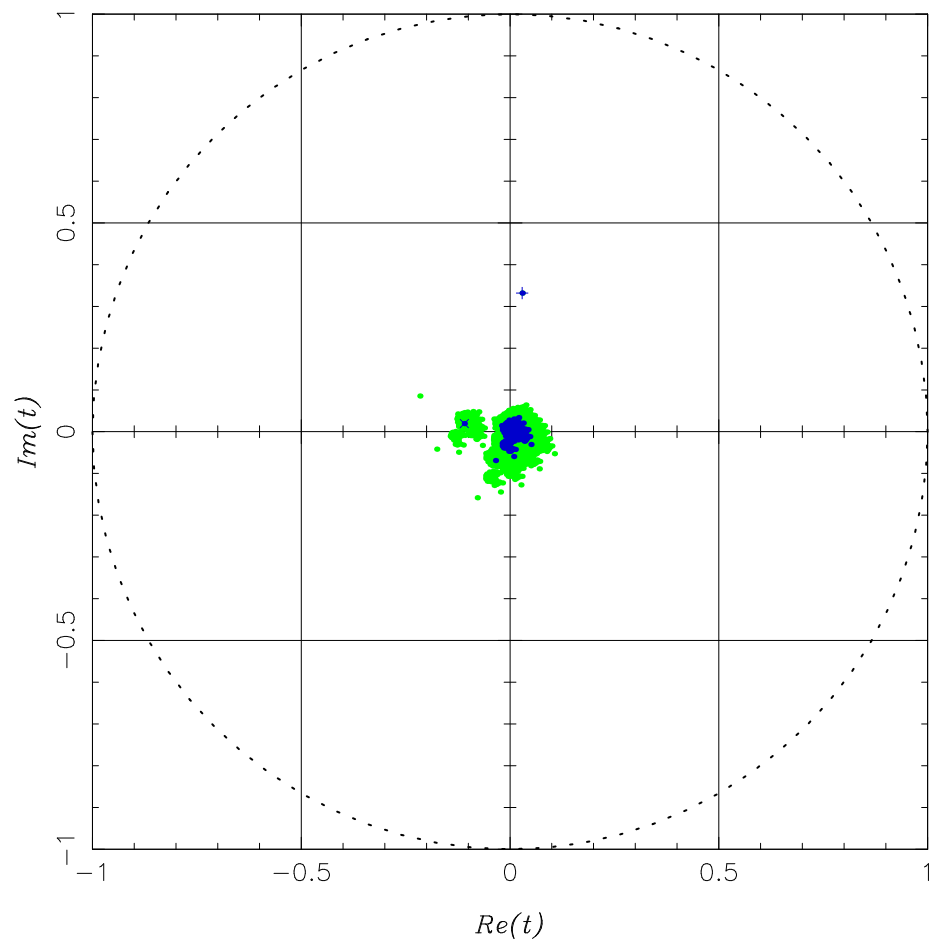

*Plot for  $q = 0.479 + 2.954 i$  ( $R = 3.000$ ,  $k = 100$ )*

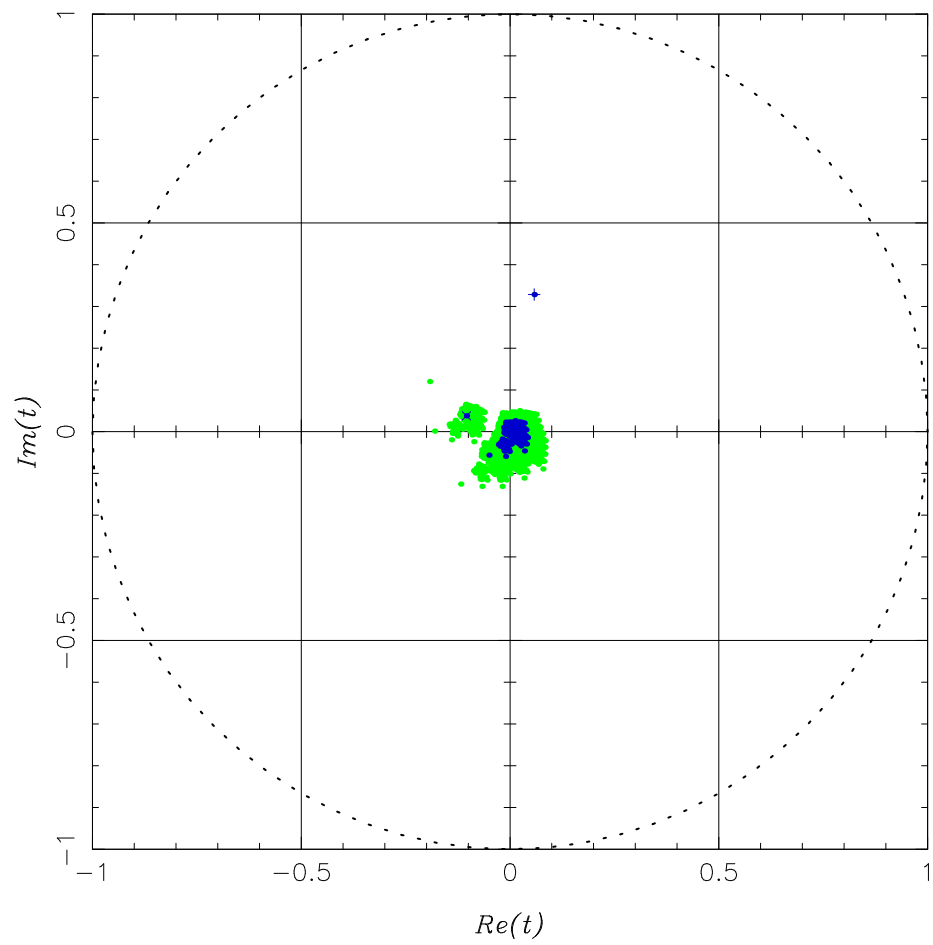

*Plot for  $q = 0.224 + 2.898 i$  ( $R = 3.000$ ,  $k = 105$ )*

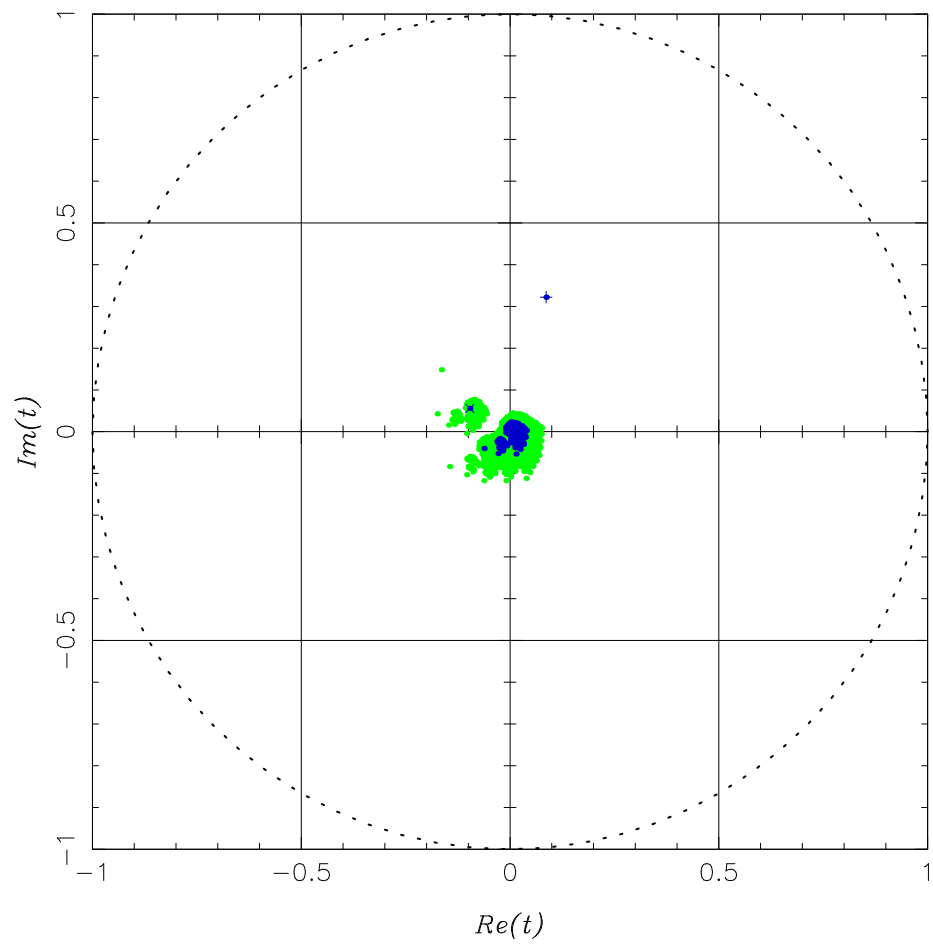

Plot for  $q = -0.026 + 2.819 i$  ( $R = 3.000$ ,  $k = 110$ )

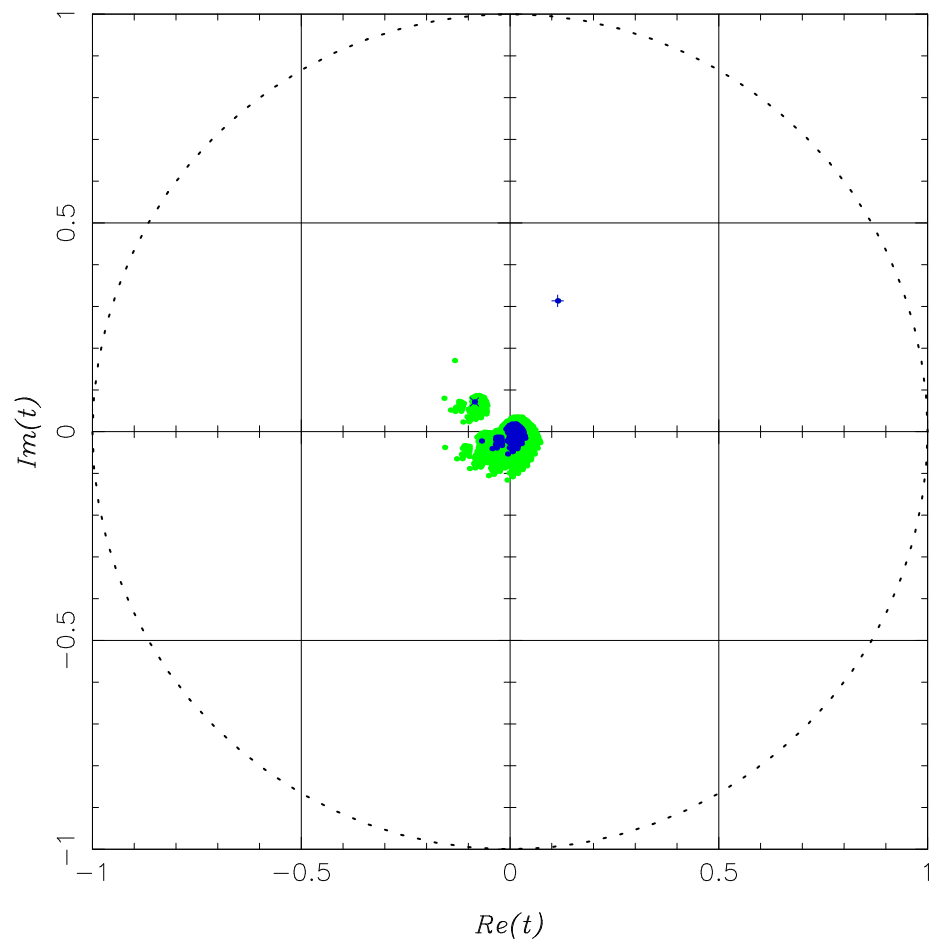



Plot for  $q = -0.268 + 2.719 i$  ( $R = 3.000$ ,  $k = 115$ )

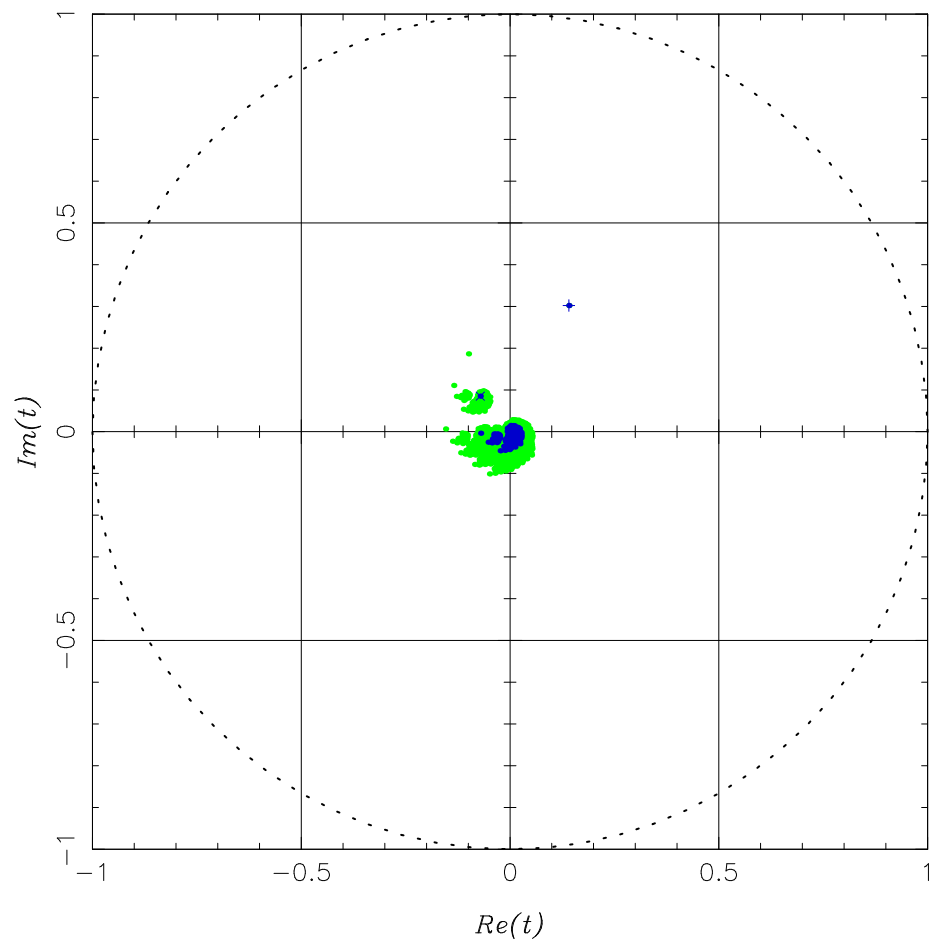

Plot for  $q = -0.500 + 2.598 i$  ( $R = 3.000$ ,  $k = 120$ )

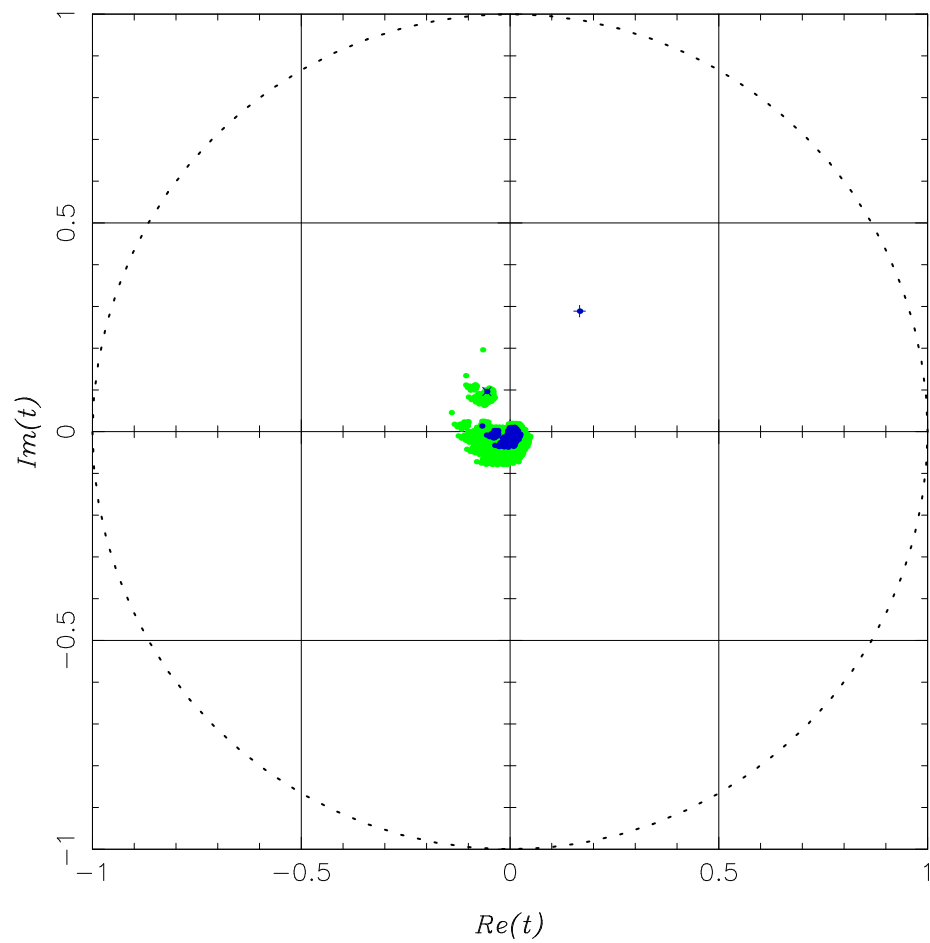

*Plot for  $q = -0.721 + 2.457 i$  ( $R = 3.000$ ,  $k = 125$ )*

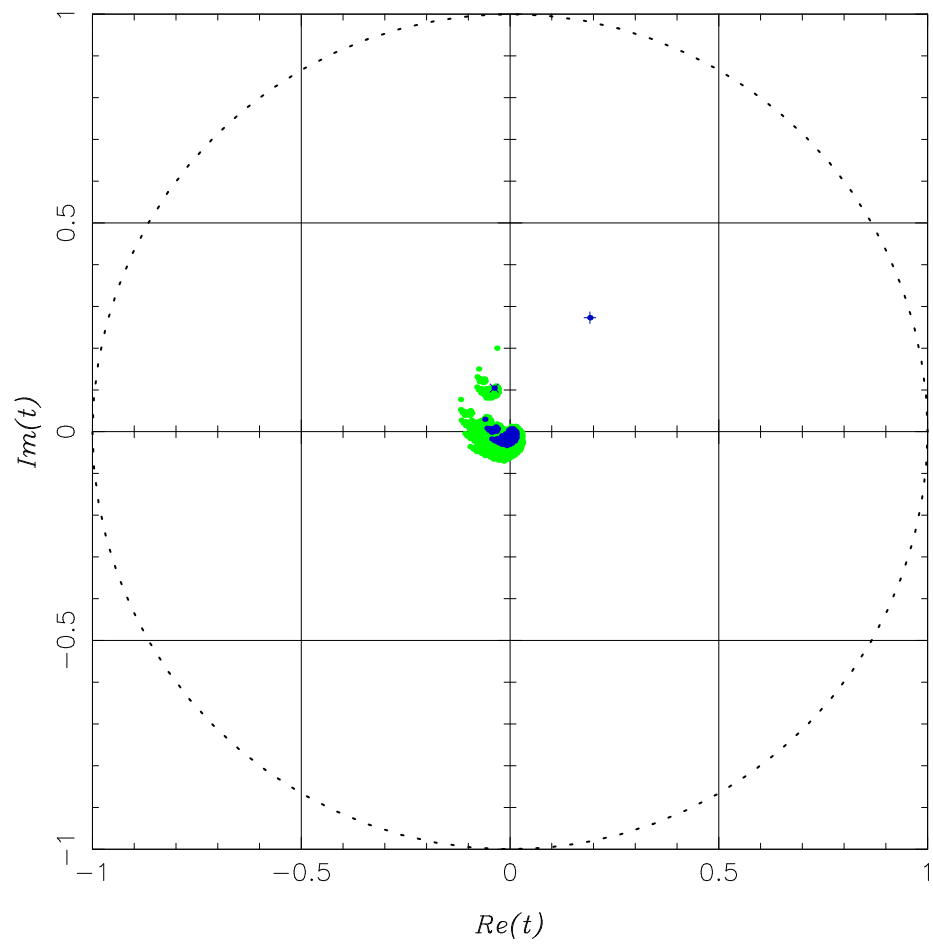

*Plot for  $q = -0.928 + 2.298 i$  ( $R = 3.000$ ,  $k = 130$ )*

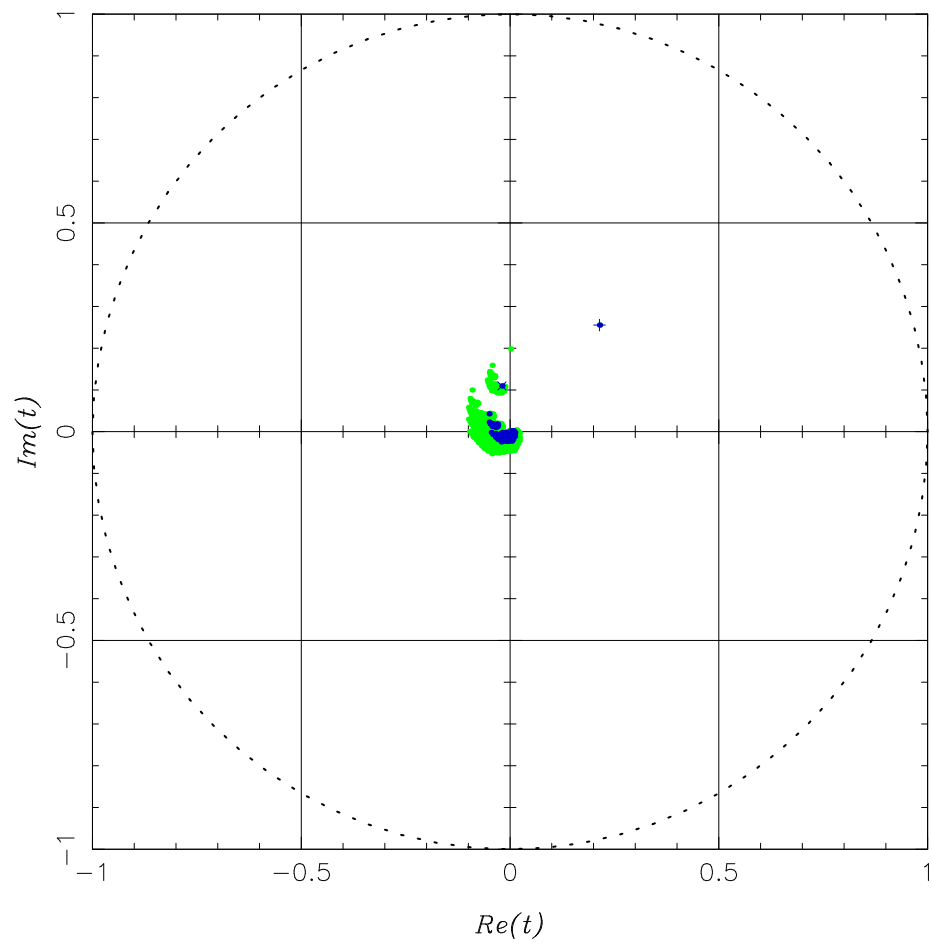

Plot for  $q = -1.121 + 2.121 i$  ( $R = 3.000$ ,  $k = 135$ )

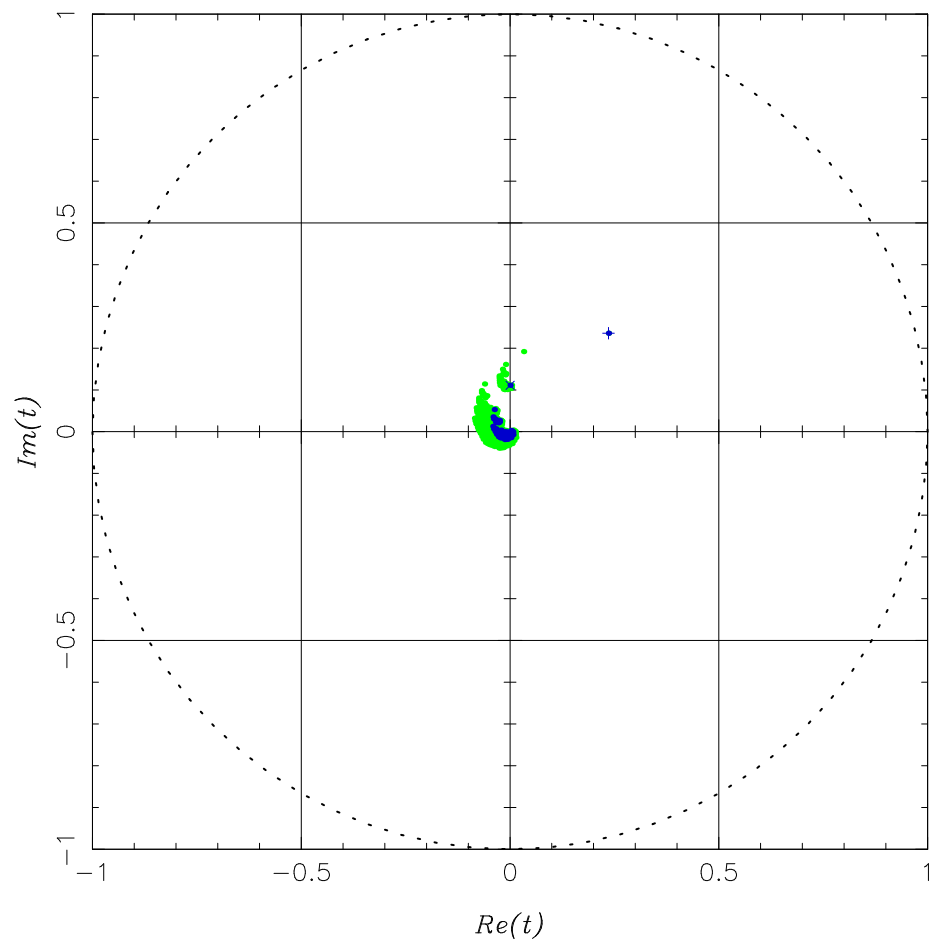

Plot for  $q = -1.298 + 1.928 i$  ( $R = 3.000$ ,  $k = 140$ )

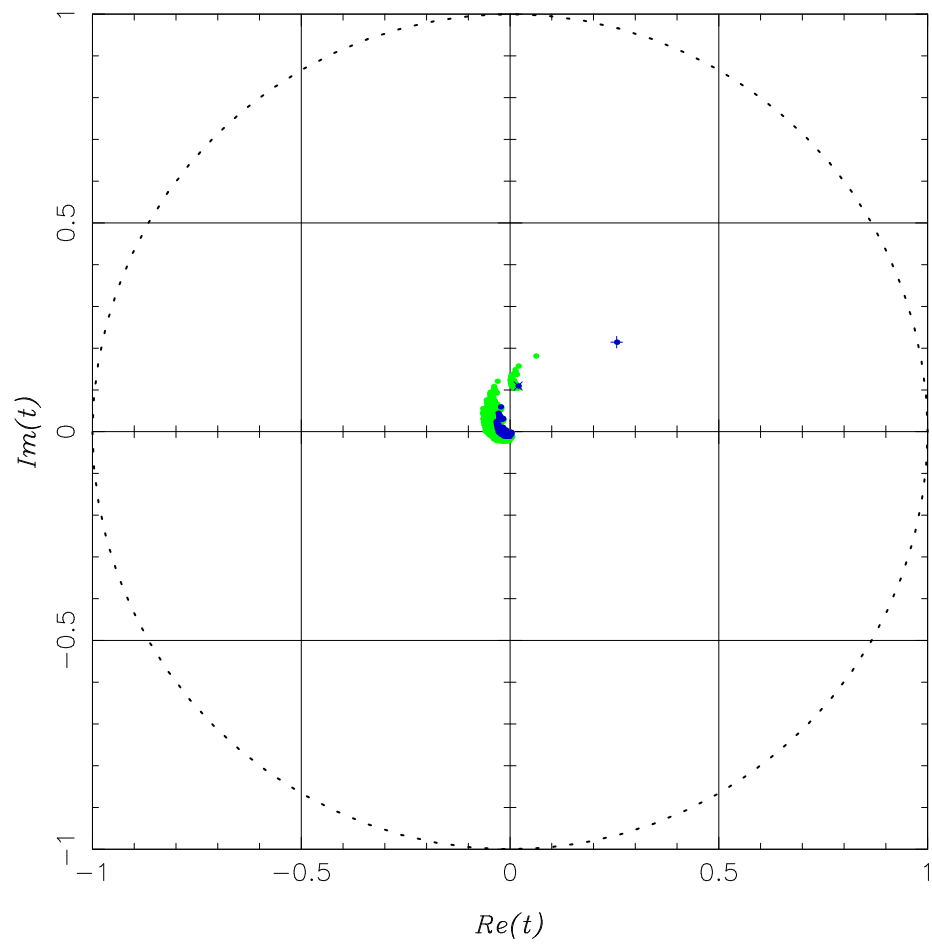

Plot for  $q = -1.457 + 1.721 i$  ( $R = 3.000$ ,  $k = 145$ )

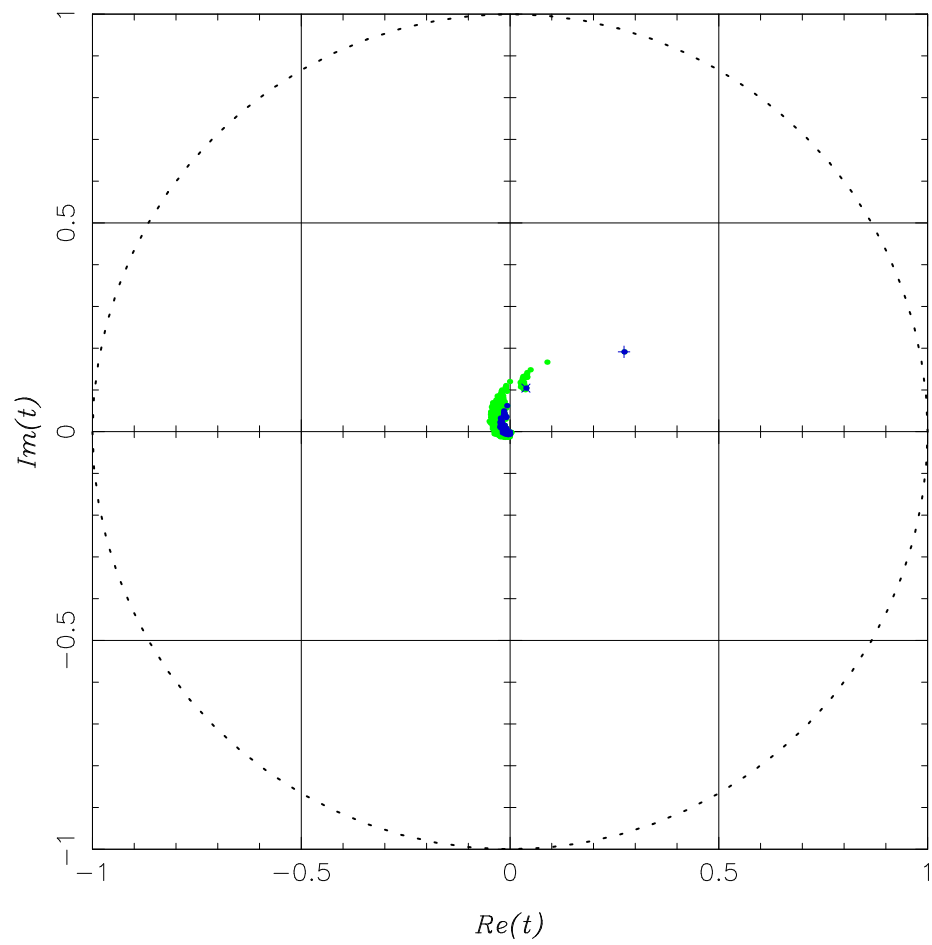

Plot for  $q = -1.598 + 1.500 i$  ( $R = 3.000$ ,  $k = 150$ )

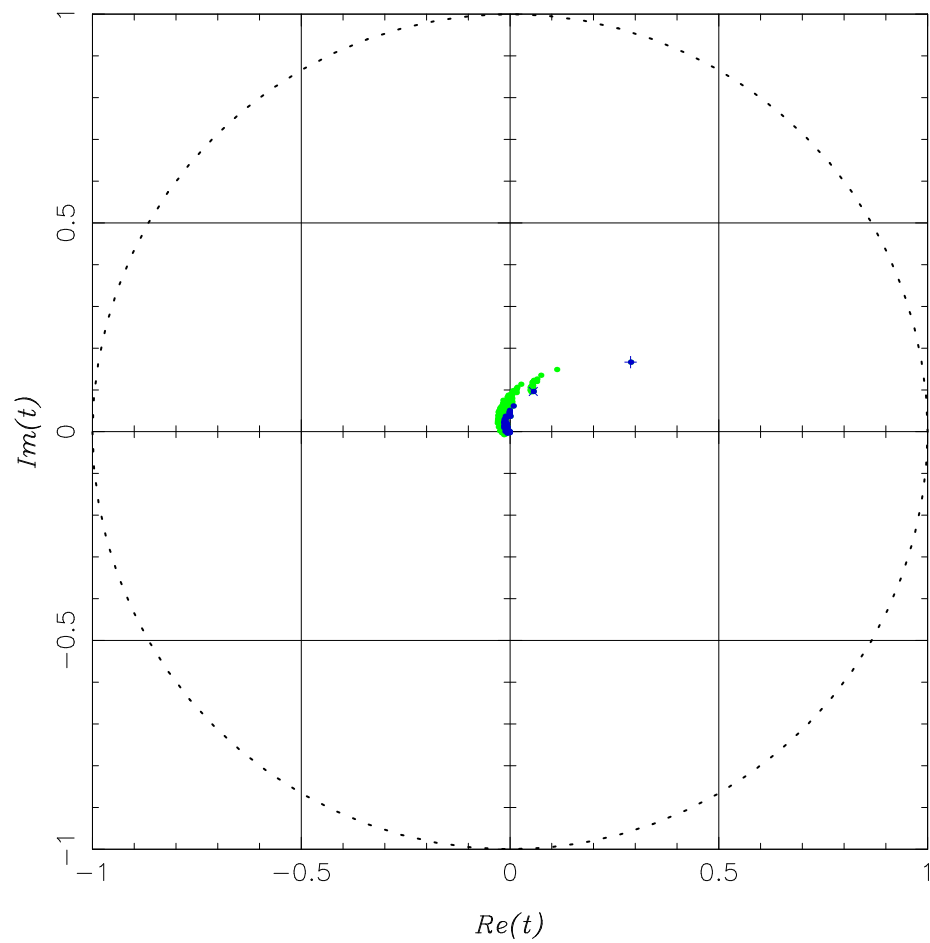



Plot for  $q = -1.719 + 1.268 i$  ( $R = 3.000$ ,  $k = 155$ )

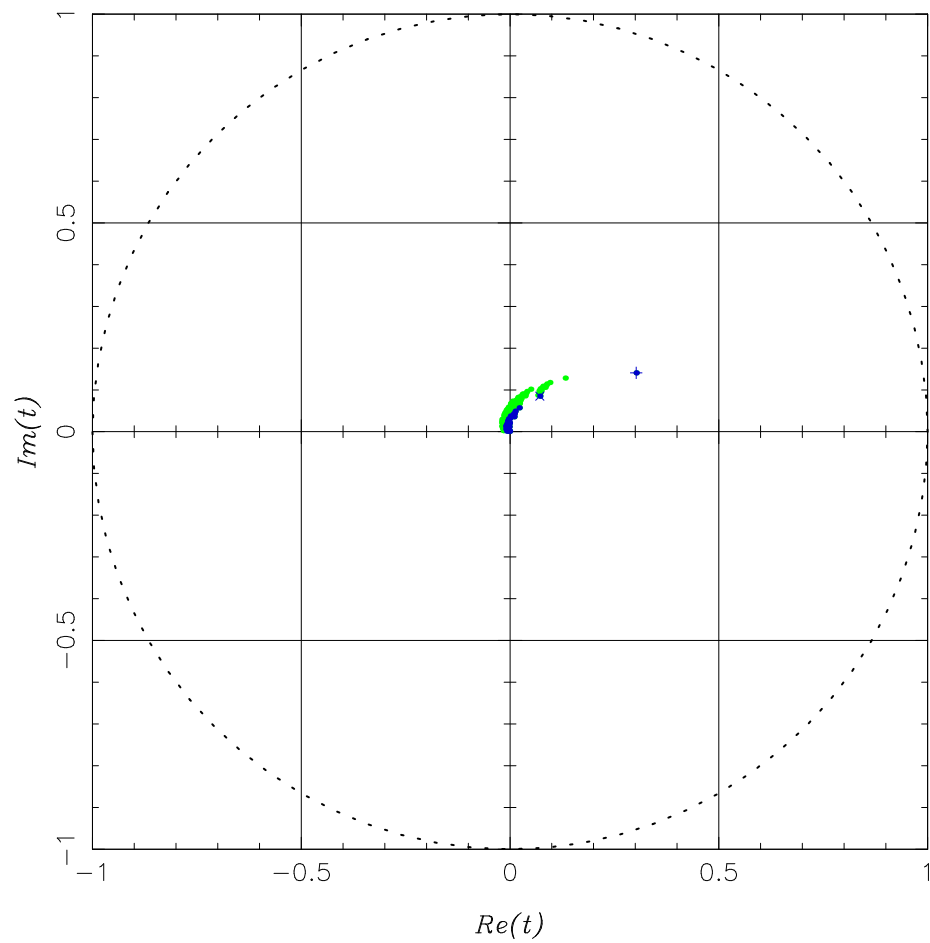

Plot for  $q = -1.819 + 1.026 i$  ( $R = 3.000$ ,  $k = 160$ )

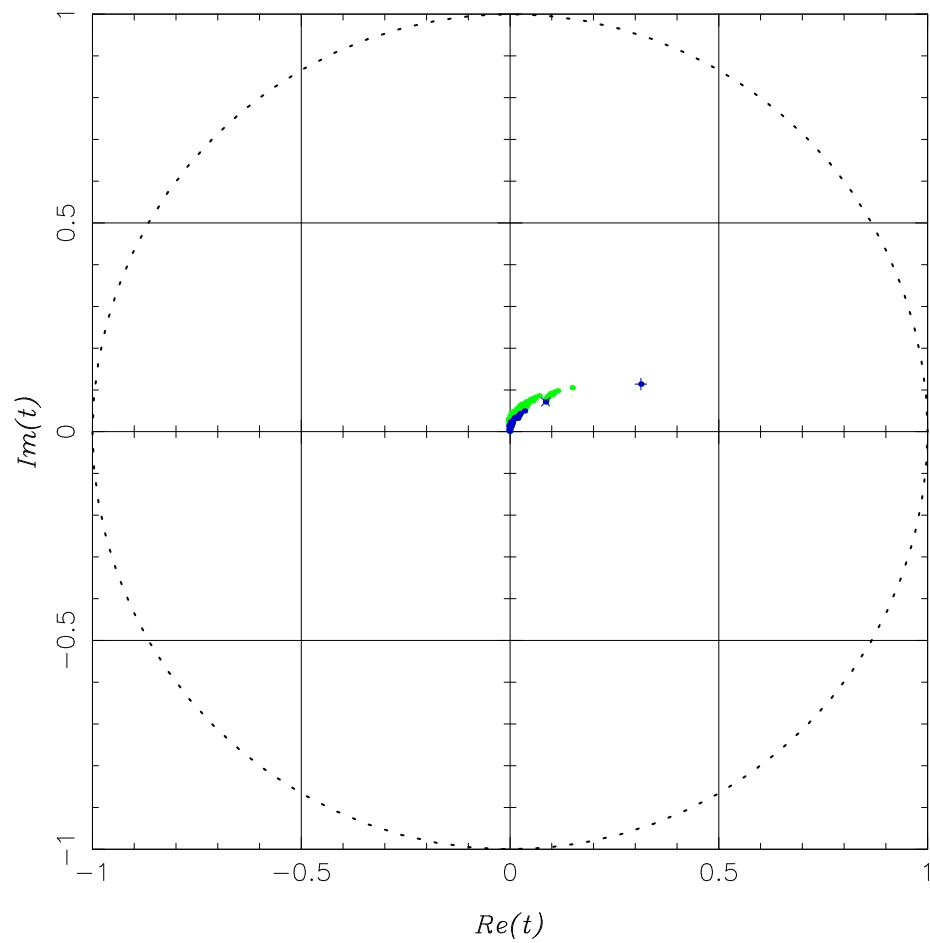

Plot for  $q = -1.898 + 0.776 i$  ( $R = 3.000$ ,  $k = 165$ )

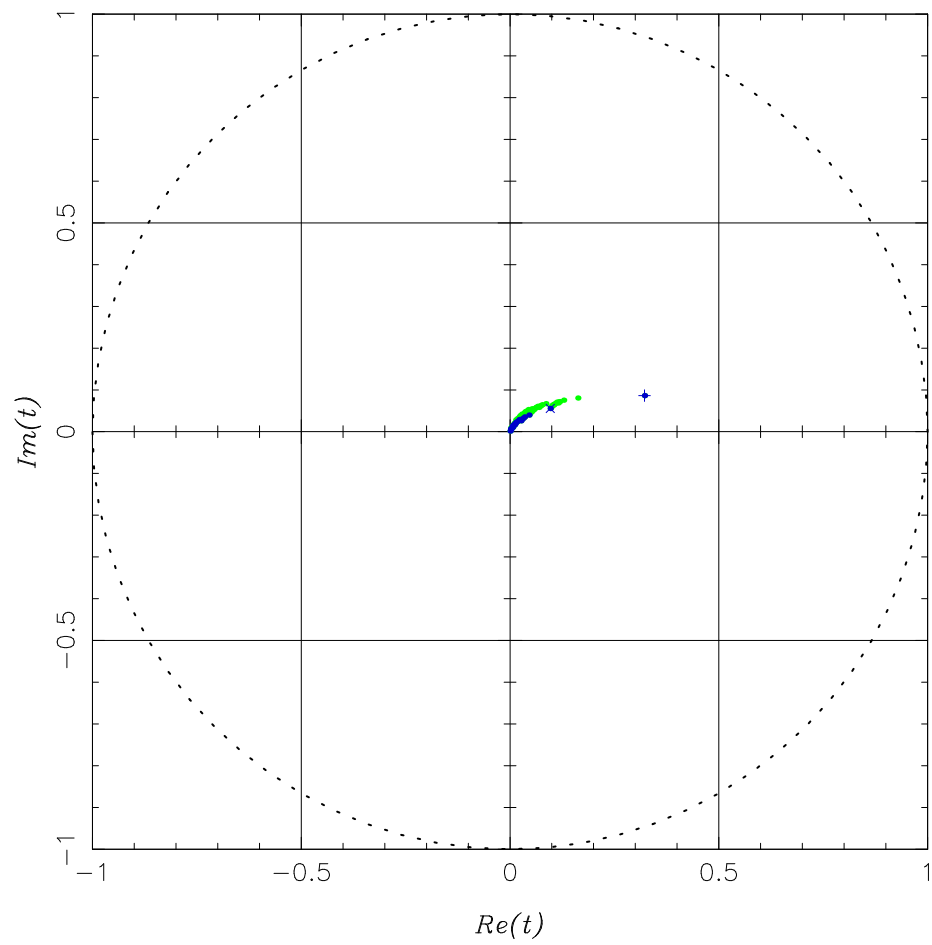

Plot for  $q = -1.954 + 0.521 i$  ( $R = 3.000$ ,  $k = 170$ )

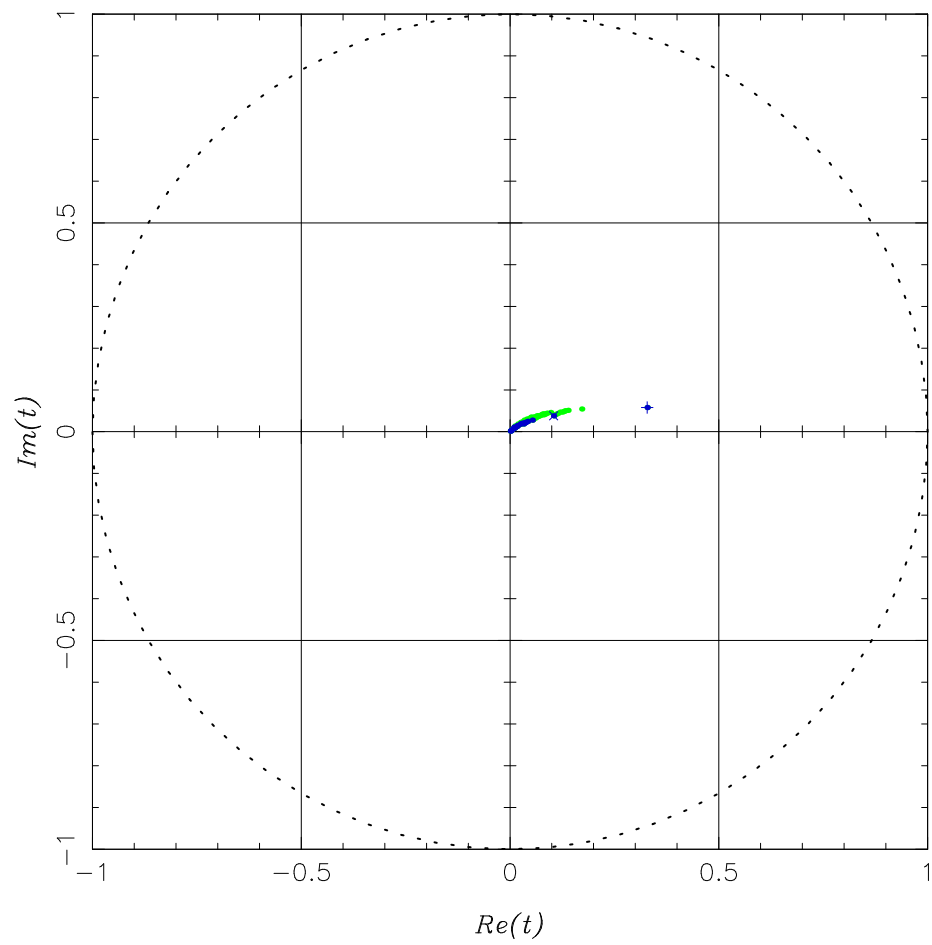

Plot for  $q = -1.989 + 0.261 i$  ( $R = 3.000$ ,  $k = 175$ )

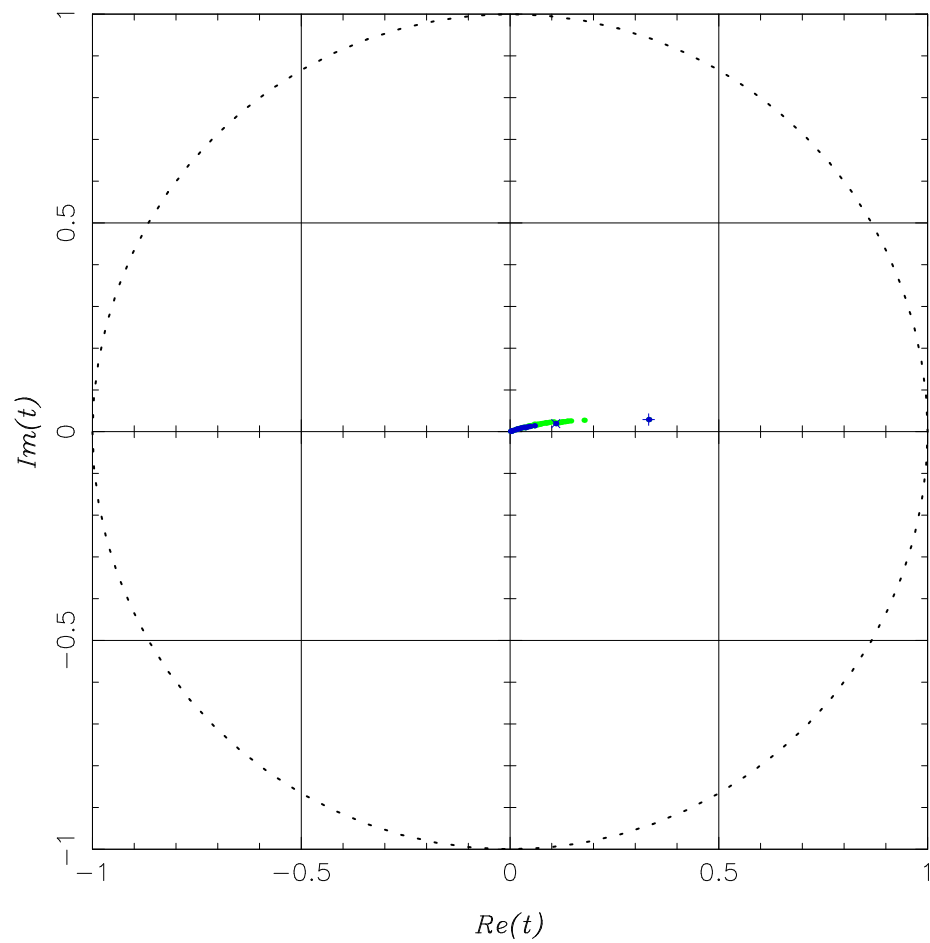

Plot for  $q = -2.000 + 0.000\ i$  ( $R = 3.000$ ,  $k = 180$ )

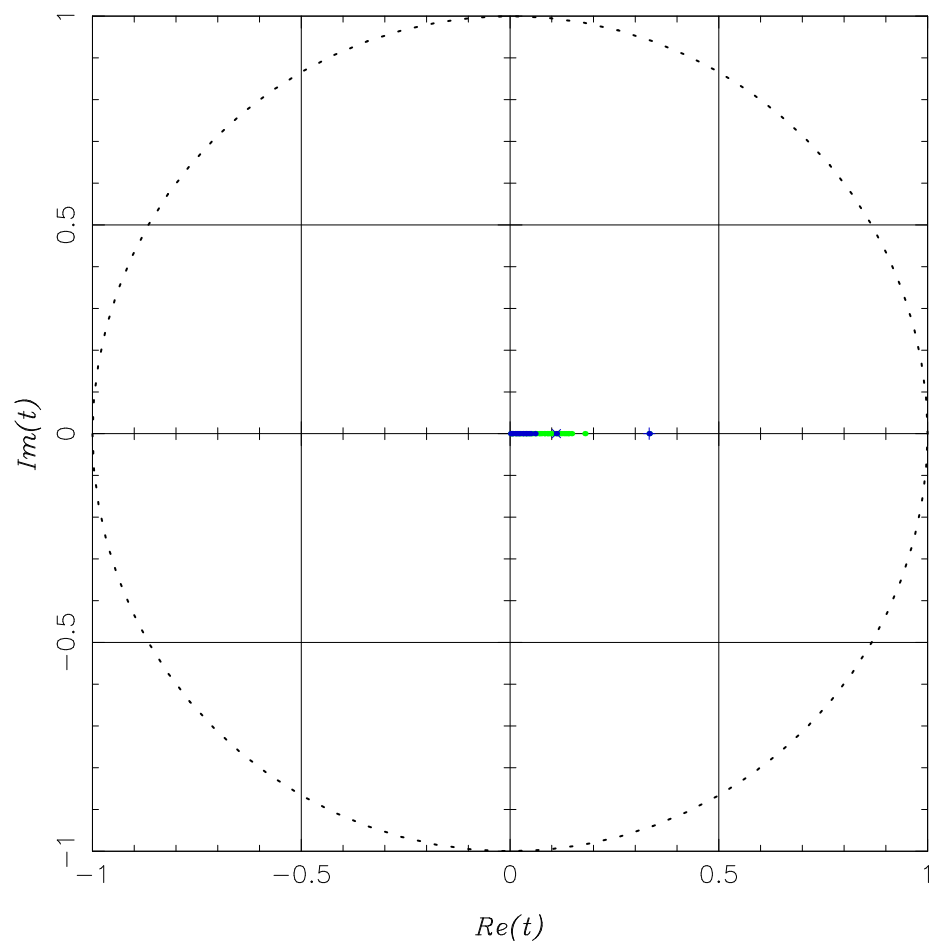

Supplement: Supplementary file 3 [file S1S2_3.0.pdf]
